# Supplementary material for: Approximations of the Iterative Stockholder Analysis scheme using exponential basis functions
Source: arXiv:2412.05079 source file (2025-06-30)
Supplement: Supplementary file 1 [file supp.pdf]

Supporting Information for:

# Approximations of the Iterative Stockholder Analysis scheme using exponential basis functions

YingXing Cheng and Benjamin Stamm\*

*Institute of Applied Analysis and Numerical Simulation, University of Stuttgart, Pfaffenwaldring  
57, 70569 Stuttgart, Germany*

E-mail: benjamin.stamm@mathematik.uni-stuttgart.de

## Contents

|                                |          |
|--------------------------------|----------|
| <b>S1 Coordinates</b>          | <b>5</b> |
| S1.1 $\text{CH}_3^+$ . . . . . | 5        |
| S1.2 $\text{CH}_4$ . . . . .   | 5        |
| S1.3 $\text{CH}_3^-$ . . . . . | 5        |
| S1.4 $\text{NH}_4^+$ . . . . . | 6        |
| S1.5 $\text{NH}_3$ . . . . .   | 6        |
| S1.6 $\text{NH}_2^-$ . . . . . | 6        |

|           |                             |           |
|-----------|-----------------------------|-----------|
| S1.7      | $\text{H}_3\text{O}^+$      | 7         |
| S1.8      | $\text{H}_2\text{O}$        | 7         |
| S1.9      | $\text{OH}^-$               | 7         |
| S1.10     | $\text{CS}_2$               | 8         |
| S1.11     | $\text{CCl}_4$              | 8         |
| S1.12     | $\text{B}_8$                | 8         |
| S1.13     | $\text{B}_8$ triplet        | 9         |
| S1.14     | $\text{B}_8^{2-}$           | 9         |
| S1.15     | $\text{B}_9^-$              | 10        |
| <b>S2</b> | <b>Basis functions info</b> | <b>10</b> |
| S2.1      | $\text{CH}_3^+$             | 10        |
| S2.2      | $\text{CH}_4$               | 14        |
| S2.3      | $\text{CH}_3^-$             | 18        |
| S2.4      | $\text{NH}_4^+$             | 22        |
| S2.5      | $\text{NH}_3$               | 26        |
| S2.6      | $\text{NH}_2^-$             | 30        |
| S2.7      | $\text{H}_3\text{O}^+$      | 34        |
| S2.8      | $\text{H}_2\text{O}$        | 37        |
| S2.9      | $\text{OH}^-$               | 41        |
| S2.10     | $\text{CS}_2$               | 45        |
| S2.11     | $\text{CCl}_4$              | 50        |
| S2.12     | $\text{B}_8$                | 55        |
| S2.13     | $\text{B}_8$ triplet        | 65        |
| S2.14     | $\text{B}_8^{2-}$           | 75        |
| S2.15     | $\text{B}_9^-$              | 85        |

|                                                         |            |
|---------------------------------------------------------|------------|
| <b>S3 Partitioning results with different methods</b>   | <b>91</b>  |
| S3.1 $\text{CH}_3^+$ . . . . .                          | 91         |
| S3.2 $\text{CH}_4$ . . . . .                            | 91         |
| S3.3 $\text{CH}_3^-$ . . . . .                          | 92         |
| S3.4 $\text{NH}_4^+$ . . . . .                          | 92         |
| S3.5 $\text{NH}_3$ . . . . .                            | 93         |
| S3.6 $\text{NH}_2^-$ . . . . .                          | 93         |
| S3.7 $\text{H}_3\text{O}^+$ . . . . .                   | 94         |
| S3.8 $\text{H}_2\text{O}$ . . . . .                     | 94         |
| S3.9 $\text{OH}^-$ . . . . .                            | 95         |
| S3.10 $\text{CS}_2$ . . . . .                           | 95         |
| S3.11 $\text{CCl}_4$ . . . . .                          | 96         |
| S3.12 $\text{B}_8$ . . . . .                            | 96         |
| S3.13 $\text{B}_8$ triplet . . . . .                    | 97         |
| S3.14 $\text{B}_8^{2-}$ . . . . .                       | 98         |
| S3.15 $\text{B}_9^-$ . . . . .                          | 99         |
| <b>S4 Radical density and entropy of selected atoms</b> | <b>100</b> |
| S4.1 $\text{CH}_3^+$ . . . . .                          | 100        |
| S4.2 $\text{CH}_4$ . . . . .                            | 103        |
| S4.3 $\text{CH}_3^-$ . . . . .                          | 106        |
| S4.4 $\text{NH}_4^+$ . . . . .                          | 109        |
| S4.5 $\text{NH}_3$ . . . . .                            | 112        |
| S4.6 $\text{NH}_2^-$ . . . . .                          | 115        |
| S4.7 $\text{H}_3\text{O}^+$ . . . . .                   | 118        |
| S4.8 $\text{H}_2\text{O}$ . . . . .                     | 121        |

|       |                      |     |
|-------|----------------------|-----|
| S4.9  | $\text{OH}^-$        | 124 |
| S4.10 | $\text{CS}_2$        | 127 |
| S4.11 | $\text{CCl}_4$       | 130 |
| S4.12 | $\text{B}_8$         | 133 |
| S4.13 | $\text{B}_8$ triplet | 136 |
| S4.14 | $\text{B}_8^{2-}$    | 139 |
| S4.15 | $\text{B}_9^-$       | 142 |

## S1 Coordinates

### S1.1 $\text{CH}_3^+$

Table S1: The coordinates of molecule  $\text{CH}_3^+$  (in a.u.).

| Atom | X         | Y         | Z        |
|------|-----------|-----------|----------|
| C    | 0.000000  | 0.000000  | 0.000000 |
| H    | 0.000000  | 2.080500  | 0.000000 |
| H    | 1.801765  | -1.040250 | 0.000000 |
| H    | -1.801765 | -1.040250 | 0.000000 |

### S1.2 $\text{CH}_4$

Table S2: The coordinates of molecule  $\text{CH}_4$  (in a.u.).

| Atom | X         | Y         | Z         |
|------|-----------|-----------|-----------|
| C    | 0.000000  | 0.000000  | 0.000000  |
| H    | 1.196816  | 1.196816  | 1.196816  |
| H    | -1.196816 | -1.196816 | 1.196816  |
| H    | -1.196816 | 1.196816  | -1.196816 |
| H    | 1.196816  | -1.196816 | -1.196816 |

### S1.3 $\text{CH}_3^-$

Table S3: The coordinates of molecule  $\text{CH}_3^-$  (in a.u.).

| Atom | X         | Y         | Z         |
|------|-----------|-----------|-----------|
| C    | 0.000000  | -0.000000 | 0.245833  |
| H    | -0.000000 | 1.967343  | -0.491665 |

Continued on next page

Table S3: The coordinates of molecule  $\text{CH}_3^-$  (in a.u.).

| Atom | X         | Y         | Z         |
|------|-----------|-----------|-----------|
| H    | 1.703769  | -0.983672 | -0.491665 |
| H    | -1.703769 | -0.983672 | -0.491665 |

## S1.4 $\text{NH}_4^+$

Table S4: The coordinates of molecule  $\text{NH}_4^+$  (in a.u.).

| Atom | X         | Y         | Z         |
|------|-----------|-----------|-----------|
| N    | 0.000000  | 0.000000  | 0.000000  |
| H    | 1.120861  | 1.120861  | 1.120861  |
| H    | -1.120861 | -1.120861 | 1.120861  |
| H    | -1.120861 | 1.120861  | -1.120861 |
| H    | 1.120861  | -1.120861 | -1.120861 |

## S1.5 $\text{NH}_3$

Table S5: The coordinates of molecule  $\text{NH}_3$  (in a.u.).

| Atom | X         | Y         | Z         |
|------|-----------|-----------|-----------|
| N    | 0.000000  | -0.000000 | 0.217039  |
| H    | -0.000000 | 1.783767  | -0.506422 |
| H    | 1.544788  | -0.891884 | -0.506422 |
| H    | -1.544788 | -0.891884 | -0.506422 |

## S1.6 $\text{NH}_2^-$

Table S6: The coordinates of molecule  $\text{NH}_2^-$  (in a.u.).

| Atom | X         | Y         | Z         |
|------|-----------|-----------|-----------|
| N    | 0.000000  | 0.000000  | 0.273275  |
| H    | 0.000000  | 1.519784  | -0.956462 |
| H    | -0.000000 | -1.519784 | -0.956462 |

## S1.7 $\text{H}_3\text{O}^+$

Table S7: The coordinates of molecule  $\text{H}_3\text{O}^+$  (in a.u.).

| Atom | X         | Y         | Z         |
|------|-----------|-----------|-----------|
| O    | 0.000000  | -0.000000 | 0.141522  |
| H    | -0.000000 | 1.783110  | -0.377390 |
| H    | 1.544218  | -0.891555 | -0.377390 |
| H    | -1.544218 | -0.891555 | -0.377390 |

## S1.8 $\text{H}_2\text{O}$

Table S8: The coordinates of molecule  $\text{H}_2\text{O}$  (in a.u.).

| Atom | X         | Y         | Z         |
|------|-----------|-----------|-----------|
| O    | 0.000000  | 0.000000  | 0.222597  |
| H    | 0.000000  | 1.444149  | -0.890388 |
| H    | -0.000000 | -1.444149 | -0.890388 |

## S1.9 $\text{OH}^-$

Table S9: The coordinates of molecule OH<sup>-</sup> (in a.u.).

| Atom | X        | Y        | Z         |
|------|----------|----------|-----------|
| O    | 0.000000 | 0.000000 | 0.203631  |
| H    | 0.000000 | 0.000000 | -1.629046 |

## S1.10 CS<sub>2</sub>

Table S10: The coordinates of molecule CS<sub>2</sub> (in a.u.).

| Atom | X        | Y        | Z         |
|------|----------|----------|-----------|
| C    | 0.000000 | 0.000000 | 0.000000  |
| S    | 0.000000 | 0.000000 | 2.967061  |
| S    | 0.000000 | 0.000000 | -2.967061 |

## S1.11 CCl<sub>4</sub>

Table S11: The coordinates of molecule CCl<sub>4</sub> (in a.u.).

| Atom | X         | Y         | Z         |
|------|-----------|-----------|-----------|
| C    | 0.000000  | 0.000000  | 0.000000  |
| Cl   | 1.955974  | 1.955974  | 1.955974  |
| Cl   | -1.955974 | -1.955974 | 1.955974  |
| Cl   | -1.955974 | 1.955974  | -1.955974 |
| Cl   | 1.955974  | -1.955974 | -1.955974 |

## S1.12 B<sub>8</sub>



Table S12: The coordinates of molecule B<sub>8</sub> (in a.u.).

| Atom | X         | Y         | Z        |
|------|-----------|-----------|----------|
| B1   | 0.000000  | 0.000000  | 0.000000 |
| B2   | 3.382610  | 0.000000  | 0.000000 |
| B3   | 2.109023  | 2.644631  | 0.000000 |
| B4   | -0.752702 | 3.297801  | 0.000000 |
| B5   | -3.047626 | 1.467659  | 0.000000 |
| B6   | -3.047626 | -1.467659 | 0.000000 |
| B7   | -0.752702 | -3.297801 | 0.000000 |
| B8   | 2.109023  | -2.644631 | 0.000000 |

### S1.13 B<sub>8</sub> triplet

Table S13: The coordinates of molecule B<sub>8</sub> triplet (in a.u.).

| Atom | X         | Y         | Z        |
|------|-----------|-----------|----------|
| B1   | 0.000000  | 0.000000  | 0.000000 |
| B2   | 3.382610  | 0.000000  | 0.000000 |
| B3   | 2.109023  | 2.644631  | 0.000000 |
| B4   | -0.752702 | 3.297801  | 0.000000 |
| B5   | -3.047626 | 1.467659  | 0.000000 |
| B6   | -3.047626 | -1.467659 | 0.000000 |
| B7   | -0.752702 | -3.297801 | 0.000000 |
| B8   | 2.109023  | -2.644631 | 0.000000 |

### S1.14 B<sub>8</sub><sup>2-</sup>

Table S14: The coordinates of molecule B<sub>8</sub><sup>2-</sup> (in a.u.).

| Atom                   | X        | Y        | Z        |
|------------------------|----------|----------|----------|
| B1                     | 0.000000 | 0.000000 | 0.000000 |
| Continued on next page |          |          |          |

Table S14: The coordinates of molecule  $B_8^{2-}$  (in a.u.).

| Atom | X         | Y         | Z        |
|------|-----------|-----------|----------|
| B2   | 3.382610  | 0.000000  | 0.000000 |
| B3   | 2.109023  | 2.644631  | 0.000000 |
| B4   | -0.752702 | 3.297801  | 0.000000 |
| B5   | -3.047626 | 1.467659  | 0.000000 |
| B6   | -3.047626 | -1.467659 | 0.000000 |
| B7   | -0.752702 | -3.297801 | 0.000000 |
| B8   | 2.109023  | -2.644631 | 0.000000 |

## S1.15 $B_9^-$

Table S15: The coordinates of molecule  $B_9^-$  (in a.u.).

| Atom | X         | Y         | Z        |
|------|-----------|-----------|----------|
| B1   | 0.000000  | 0.000000  | 0.000000 |
| B2   | 3.779453  | 0.000000  | 0.000000 |
| B3   | 2.672477  | 2.672477  | 0.000000 |
| B4   | 0.000000  | 3.779453  | 0.000000 |
| B5   | -2.672477 | 2.672477  | 0.000000 |
| B6   | -3.779453 | 0.000000  | 0.000000 |
| B7   | -2.672477 | -2.672477 | 0.000000 |
| B8   | 0.000000  | -3.779453 | 0.000000 |
| B9   | 2.672477  | -2.672477 | 0.000000 |

## S2 Basis functions info

### S2.1 $CH_3^+$

Table S16: The basis info of molecule  $\text{CH}_3^+$ .

|       |      |     | $n_{a,k}$ | $\alpha_{a,k}$ | $c_{a,k}$ |
|-------|------|-----|-----------|----------------|-----------|
| Model | Atom | $k$ |           |                |           |
| LISA1 | C    | 1   | 2.0000    | 148.3000       | 0.1404    |
|       |      | 2   | 2.0000    | 42.1900        | 0.5769    |
|       |      | 3   | 2.0000    | 15.3300        | 1.0779    |
|       |      | 4   | 2.0000    | 6.1460         | 0.0000    |
|       |      | 5   | 2.0000    | 0.7846         | 3.2954    |
|       |      | 6   | 2.0000    | 0.2511         | 0.4810    |
|       | H    | 1   | 2.0000    | 5.6720         | 0.0336    |
|       |      | 2   | 2.0000    | 1.5050         | 0.4905    |
|       |      | 3   | 2.0000    | 0.5308         | 0.2803    |
|       |      | 4   | 2.0000    | 0.2204         | 0.0050    |
| LISA2 | C    | 1   | 2.0000    | 148.3000       | 0.1404    |
|       |      | 2   | 2.0000    | 42.1900        | 0.5768    |
|       |      | 3   | 2.0000    | 15.3300        | 1.0781    |
|       |      | 4   | 2.0000    | 6.1460         | 0.0000    |
|       |      | 5   | 2.0000    | 0.7846         | 3.2934    |
|       |      | 6   | 2.0000    | 0.2511         | 0.4851    |
|       | H    | 1   | 2.0000    | 5.6720         | 0.0338    |
|       |      | 2   | 2.0000    | 1.5050         | 0.4894    |
|       |      | 3   | 2.0000    | 0.5308         | 0.2823    |
|       |      | 4   | 2.0000    | 0.2204         | 0.0023    |
|       |      | 5   | 1.0000    | 1.0000         | 0.0009    |
| LISA3 | --   | --  | --        | --             | --        |
| LISA4 | C    | 1   | 2.0000    | 233.9861       | 0.0211    |
|       |      | 2   | 2.0000    | 191.1093       | 0.0732    |
|       |      | 3   | 2.0000    | 51.2230        | 0.1144    |
|       |      | 4   | 2.0000    | 42.7414        | 0.5354    |
|       |      | 5   | 2.0000    | 14.7443        | 1.0667    |
|       |      | 6   | 2.0000    | 0.8016         | 2.8024    |
|       |      | 7   | 2.0000    | 0.3994         | 0.9732    |
|       |      | 8   | 2.0000    | 0.3312         | 0.0000    |
|       |      | 9   | 2.0000    | 0.2759         | 0.0000    |
|       |      | 10  | 2.0000    | 0.2377         | 0.0000    |
|       |      | 11  | 2.0000    | 0.1169         | 0.0000    |

Continued on next page

Table S16: The basis info of molecule CH<sub>3</sub><sup>+</sup>.

| Model | Atom | $k$ | $n_{a,k}$ | $\alpha_{a,k}$ | $c_{a,k}$ |
|-------|------|-----|-----------|----------------|-----------|
|       | H    | 12  | 2.0000    | 0.0786         | 0.0000    |
|       |      | 13  | 2.0000    | 0.0696         | 0.0001    |
|       |      | 1   | 2.0000    | 7.1896         | 0.0203    |
|       |      | 2   | 2.0000    | 1.6120         | 0.4876    |
|       |      | 3   | 2.0000    | 0.5023         | 0.2827    |
|       |      | 4   | 2.0000    | 0.2097         | 0.0000    |
|       |      | 5   | 2.0000    | 0.1683         | 0.0138    |
|       |      |     |           |                |           |
| LISA5 | --   | --  | --        | --             | --        |
| LISA6 | C    | 1   | 1.0000    | 13.0886        | 1.6078    |
|       |      | 2   | 1.0000    | 2.4356         | 1.2660    |
|       |      | 3   | 1.0000    | 1.9858         | 2.9333    |
|       |      | 4   | 1.0000    | 0.9936         | 0.0000    |
|       |      | 5   | 1.0000    | 0.8363         | 0.0000    |
|       | H    | 1   | 1.0000    | 4.2476         | 0.0000    |
|       |      | 2   | 1.0000    | 3.4951         | 0.4824    |
|       |      | 3   | 1.0000    | 1.9499         | 0.2485    |
|       |      | 4   | 1.0000    | 1.4845         | 0.0000    |
|       |      | 5   | 1.0000    | 1.2133         | 0.0000    |
| NLIS1 | C    | 1   | 2.0000    | 202.0774       | 0.0924    |
|       |      | 2   | 2.0000    | 44.9054        | 0.6399    |
|       |      | 3   | 2.0000    | 14.6453        | 1.0924    |
|       |      | 4   | 2.0000    | 0.7169         | 1.4447    |
|       |      | 5   | 2.0000    | 0.7169         | 1.9937    |
|       |      | 6   | 2.0000    | 0.2495         | 0.3444    |
|       | H    | 1   | 2.0000    | 10.7652        | 0.0176    |
|       |      | 2   | 2.0000    | 1.8069         | 0.3365    |
|       |      | 3   | 2.0000    | 0.7655         | 0.3862    |
|       |      | 4   | 2.0000    | 0.2958         | 0.0570    |
| NLIS2 | C    | 1   | 2.0000    | 220.1466       | 0.0794    |
|       |      | 2   | 2.0000    | 48.4201        | 0.5894    |
|       |      | 3   | 2.0000    | 15.4764        | 1.1269    |
|       |      | 4   | 2.0000    | 0.6991         | 1.5319    |
|       |      | 5   | 2.0000    | 0.6991         | 1.5430    |

Continued on next page

Table S16: The basis info of molecule  $\text{CH}_3^+$ .

| Model | Atom | $k$ | $n_{a,k}$ | $\alpha_{a,k}$ | $c_{a,k}$ |
|-------|------|-----|-----------|----------------|-----------|
|       |      |     |           |                |           |
| NLIS3 | H    | 6   | 1.0000    | 1.8155         | 0.7283    |
|       |      | 1   | 2.0000    | 8329010.0172   | 0.0000    |
|       |      | 2   | 2.0000    | 1.2967         | 0.3323    |
|       |      | 3   | 2.0000    | 0.4551         | 0.1116    |
|       |      | 4   | 1.0000    | 2.7140         | 0.3563    |
|       | C    | 1   | 2.0000    | 220.1466       | 0.0794    |
|       |      | 2   | 2.0000    | 48.4201        | 0.5894    |
|       |      | 3   | 2.0000    | 15.4764        | 1.1269    |
|       |      | 4   | 2.0000    | 0.6991         | 3.0749    |
|       |      | 5   | 1.0000    | 1.8155         | 0.5693    |
|       |      | 6   | 1.0000    | 1.8155         | 0.1590    |
|       |      | 1   | 2.0000    | 1.2967         | 0.3323    |
|       |      | 2   | 2.0000    | 0.4551         | 0.1116    |
|       |      | 3   | 1.0000    | 2.7140         | 0.3507    |
|       |      | 4   | 1.0000    | 2.7140         | 0.0056    |
| NLIS4 | C    | 1   | 1.0000    | 13.3617        | 0.8612    |
|       |      | 2   | 1.0000    | 13.3617        | 0.6012    |
|       |      | 3   | 1.0000    | 2.1642         | 1.5511    |
|       |      | 4   | 1.0000    | 2.1642         | 1.5025    |
|       |      | 5   | 1.0000    | 2.1642         | 1.0028    |
|       |      | 6   | 1.0000    | 13.3617        | 0.1326    |
|       | H    | 1   | 1.0000    | 2.7166         | 0.0390    |
|       |      | 2   | 1.0000    | 2.7166         | 0.3961    |
|       |      | 3   | 1.0000    | 2.7166         | 0.2563    |
|       |      | 4   | 1.0000    | 2.7166         | 0.0915    |
| MBIS  | C    | 1   | 1.0000    | 13.3617        | 1.5951    |
|       |      | 2   | 1.0000    | 2.1642         | 4.0564    |
|       | H    | 1   | 1.0000    | 2.7166         | 0.7828    |
| GMBIS | C    | 1   | 1.1380    | 14.4790        | 1.5748    |
|       |      | 2   | 1.0000    | 2.1692         | 4.0736    |
|       | H    | 1   | 1.0380    | 2.6014         | 0.7839    |

## S2.2 CH<sub>4</sub>

Table S17: The basis info of molecule CH<sub>4</sub>.

|       |      |     | $n_{a,k}$ | $\alpha_{a,k}$ | $c_{a,k}$ |
|-------|------|-----|-----------|----------------|-----------|
| Model | Atom | $k$ |           |                |           |
| LISA1 | C    | 1   | 2.0000    | 148.3000       | 0.1401    |
|       |      | 2   | 2.0000    | 42.1900        | 0.5701    |
|       |      | 3   | 2.0000    | 15.3300        | 1.0786    |
|       |      | 4   | 2.0000    | 6.1460         | 0.0000    |
|       |      | 5   | 2.0000    | 0.7846         | 3.2961    |
|       |      | 6   | 2.0000    | 0.2511         | 1.5029    |
|       | H    | 1   | 2.0000    | 5.6720         | 0.0442    |
|       |      | 2   | 2.0000    | 1.5050         | 0.4636    |
|       |      | 3   | 2.0000    | 0.5308         | 0.2822    |
|       |      | 4   | 2.0000    | 0.2204         | 0.0634    |
| LISA2 | C    | 1   | 2.0000    | 148.3000       | 0.1402    |
|       |      | 2   | 2.0000    | 42.1900        | 0.5697    |
|       |      | 3   | 2.0000    | 15.3300        | 1.0791    |
|       |      | 4   | 2.0000    | 6.1460         | 0.0000    |
|       |      | 5   | 2.0000    | 0.7846         | 3.2889    |
|       |      | 6   | 2.0000    | 0.2511         | 1.5209    |
|       | H    | 1   | 2.0000    | 5.6720         | 0.0448    |
|       |      | 2   | 2.0000    | 1.5050         | 0.4600    |
|       |      | 3   | 2.0000    | 0.5308         | 0.2888    |
|       |      | 4   | 2.0000    | 0.2204         | 0.0522    |
|       |      | 5   | 1.0000    | 1.0000         | 0.0048    |
| LISA3 | --   | --  | --        | --             | --        |
| LISA4 | C    | 1   | 2.0000    | 233.9861       | 0.0299    |
|       |      | 2   | 2.0000    | 191.1093       | 0.0597    |
|       |      | 3   | 2.0000    | 51.2230        | 0.1834    |
|       |      | 4   | 2.0000    | 42.7414        | 0.4525    |
|       |      | 5   | 2.0000    | 14.7443        | 1.0853    |
|       |      | 6   | 2.0000    | 0.8016         | 2.5510    |
|       |      | 7   | 2.0000    | 0.3994         | 1.7620    |
|       |      | 8   | 2.0000    | 0.3312         | 0.0000    |

Continued on next page

Table S17: The basis info of molecule CH<sub>4</sub>.

|       |      |     | $n_{a,k}$ | $\alpha_{a,k}$ | $c_{a,k}$ |
|-------|------|-----|-----------|----------------|-----------|
| Model | Atom | $k$ |           |                |           |
|       |      | 9   | 2.0000    | 0.2759         | 0.0000    |
|       |      | 10  | 2.0000    | 0.2377         | 0.3592    |
|       |      | 11  | 2.0000    | 0.1169         | 0.0767    |
|       |      | 12  | 2.0000    | 0.0786         | 0.0000    |
|       |      | 13  | 2.0000    | 0.0696         | 0.0017    |
|       | H    | 1   | 2.0000    | 7.1896         | 0.0308    |
|       |      | 2   | 2.0000    | 1.6120         | 0.4456    |
|       |      | 3   | 2.0000    | 0.5023         | 0.3235    |
|       |      | 4   | 2.0000    | 0.2097         | 0.0601    |
|       |      | 5   | 2.0000    | 0.1683         | 0.0000    |
| LISA5 | --   | --  | --        | --             | --        |
| LISA6 | C    | 1   | 1.0000    | 13.0886        | 1.6105    |
|       |      | 2   | 1.0000    | 2.4356         | 0.0000    |
|       |      | 3   | 1.0000    | 1.9858         | 4.9211    |
|       |      | 4   | 1.0000    | 0.9936         | 0.0000    |
|       |      | 5   | 1.0000    | 0.8363         | 0.0001    |
|       | H    | 1   | 1.0000    | 4.2476         | 0.0000    |
|       |      | 2   | 1.0000    | 3.4951         | 0.3387    |
|       |      | 3   | 1.0000    | 1.9499         | 0.5279    |
|       |      | 4   | 1.0000    | 1.4845         | 0.0000    |
|       |      | 5   | 1.0000    | 1.2133         | 0.0000    |
| NLIS1 | C    | 1   | 2.0000    | 190.0902       | 0.1025    |
|       |      | 2   | 2.0000    | 42.4657        | 0.6758    |
|       |      | 3   | 2.0000    | 13.9753        | 1.0578    |
|       |      | 4   | 2.0000    | 0.6521         | 1.7064    |
|       |      | 5   | 2.0000    | 0.6521         | 2.1839    |
|       |      | 6   | 2.0000    | 0.2125         | 0.8758    |
|       | H    | 1   | 2.0000    | 9.4192         | 0.0233    |
|       |      | 2   | 2.0000    | 1.7696         | 0.3707    |
|       |      | 3   | 2.0000    | 0.6190         | 0.3937    |
|       |      | 4   | 2.0000    | 0.2001         | 0.0620    |
| NLIS2 | C    | 1   | 2.0000    | 223.5187       | 0.0769    |
|       |      | 2   | 2.0000    | 49.0097        | 0.5790    |

Continued on next page

Table S17: The basis info of molecule CH<sub>4</sub>.

| Model | Atom | $k$ | $n_{a,k}$ | $\alpha_{a,k}$ | $c_{a,k}$ |
|-------|------|-----|-----------|----------------|-----------|
| NLIS3 |      | 3   | 2.0000    | 15.5417        | 1.1280    |
|       |      | 4   | 2.0000    | 0.6241         | 1.5073    |
|       |      | 5   | 2.0000    | 0.6241         | 1.6027    |
|       |      | 6   | 1.0000    | 1.6422         | 1.6528    |
|       | H    | 1   | 2.0000    | 1.5847         | 0.0242    |
|       |      | 2   | 2.0000    | 1.5847         | 0.0696    |
|       |      | 3   | 2.0000    | 1.5839         | 0.0732    |
|       |      | 4   | 1.0000    | 2.2718         | 0.6962    |
|       | C    | 1   | 2.0000    | 223.5187       | 0.0769    |
|       |      | 2   | 2.0000    | 49.0097        | 0.5790    |
|       |      | 3   | 2.0000    | 15.5417        | 1.1280    |
|       |      | 4   | 2.0000    | 0.6241         | 3.1100    |
|       |      | 5   | 1.0000    | 1.6422         | 1.1291    |
|       |      | 6   | 1.0000    | 1.6422         | 0.5237    |
|       |      | 1   | 2.0000    | 1.5844         | 0.0838    |
|       |      | 2   | 2.0000    | 1.5843         | 0.0833    |
|       |      | 3   | 1.0000    | 2.2718         | 0.6962    |
|       |      | 4   | 1.0000    | 0.0000         | 0.0000    |
| NLIS4 | C    | 1   | 1.0000    | 13.0563        | 1.0008    |
|       |      | 2   | 1.0000    | 13.0563        | 0.6439    |
|       |      | 3   | 1.0000    | 1.8766         | 1.7391    |
|       |      | 4   | 1.0000    | 1.8766         | 1.6643    |
|       |      | 5   | 1.0000    | 1.8766         | 1.1979    |
|       |      | 6   | 1.0000    | 1.8766         | 0.4881    |
|       | H    | 1   | 1.0000    | 0.4996         | 0.0001    |
|       |      | 2   | 1.0000    | 0.4996         | 0.0000    |
|       |      | 3   | 1.0000    | 2.5742         | 0.4604    |
|       |      | 4   | 1.0000    | 2.5742         | 0.3556    |
| MBIS  | C    | 1   | 1.0000    | 13.0545        | 1.6450    |
|       |      | 2   | 1.0000    | 1.8757         | 5.0914    |
|       | H    | 1   | 1.0000    | 2.5749         | 0.8155    |
| GMBIS | C    | 1   | 1.1380    | 14.1043        | 1.6245    |
|       |      | 2   | 1.0000    | 1.8737         | 5.1300    |

Continued on next page



Table S17: The basis info of molecule CH<sub>4</sub>.

|       |      |     | $n_{a,k}$ | $\alpha_{a,k}$ | $c_{a,k}$ |
|-------|------|-----|-----------|----------------|-----------|
| Model | Atom | $k$ |           |                |           |
|       | H    | 1   | 1.0380    | 2.4722         | 0.8111    |

## S2.3 CH<sub>3</sub><sup>-</sup>

Table S18: The basis info of molecule CH<sub>3</sub><sup>-</sup>.

| Model | Atom | <i>k</i> | $n_{a,k}$ | $\alpha_{a,k}$ | $c_{a,k}$ |
|-------|------|----------|-----------|----------------|-----------|
| LISA1 | C    | 1        | 2.0000    | 148.3000       | 0.1412    |
|       |      | 2        | 2.0000    | 42.1900        | 0.5680    |
|       |      | 3        | 2.0000    | 15.3300        | 1.0741    |
|       |      | 4        | 2.0000    | 6.1460         | 0.0451    |
|       |      | 5        | 2.0000    | 0.7846         | 2.6463    |
|       |      | 6        | 2.0000    | 0.2511         | 2.5919    |
|       | H    | 1        | 2.0000    | 5.6720         | 0.0356    |
|       |      | 2        | 2.0000    | 1.5050         | 0.5111    |
|       |      | 3        | 2.0000    | 0.5308         | 0.0000    |
|       |      | 4        | 2.0000    | 0.2204         | 0.4313    |
| LISA2 | C    | 1        | 2.0000    | 148.3000       | 0.1423    |
|       |      | 2        | 2.0000    | 42.1900        | 0.5615    |
|       |      | 3        | 2.0000    | 15.3300        | 1.0911    |
|       |      | 4        | 2.0000    | 6.1460         | 0.0221    |
|       |      | 5        | 2.0000    | 0.7846         | 2.7400    |
|       |      | 6        | 2.0000    | 0.2511         | 2.4949    |
|       | H    | 1        | 2.0000    | 5.6720         | 0.0350    |
|       |      | 2        | 2.0000    | 1.5050         | 0.4832    |
|       |      | 3        | 2.0000    | 0.5308         | 0.0935    |
|       |      | 4        | 2.0000    | 0.2204         | 0.0000    |
|       |      | 5        | 1.0000    | 1.0000         | 0.3712    |
| LISA3 | C    | 1        | 2.0000    | 233.9861       | 0.0513    |
|       |      | 2        | 2.0000    | 191.1093       | 0.0285    |
|       |      | 3        | 2.0000    | 51.2230        | 0.3382    |
|       |      | 4        | 2.0000    | 42.7414        | 0.2814    |
|       |      | 5        | 2.0000    | 14.7443        | 1.1315    |
|       |      | 6        | 2.0000    | 0.8016         | 1.7504    |
|       |      | 7        | 2.0000    | 0.3994         | 9.2068    |
|       |      | 8        | 2.0000    | 0.3312         | -12.2667  |
|       |      | 9        | 2.0000    | 0.2759         | 3.8427    |

Continued on next page

Table S18: The basis info of molecule  $\text{CH}_3^-$ .

|       |      |     | $n_{a,k}$ | $\alpha_{a,k}$ | $c_{a,k}$ |
|-------|------|-----|-----------|----------------|-----------|
| Model | Atom | $k$ |           |                |           |
| LISA4 |      | 10  | 2.0000    | 0.2377         | 2.3288    |
|       |      | 11  | 2.0000    | 0.1169         | 0.7194    |
|       |      | 12  | 2.0000    | 0.0786         | -0.9834   |
|       |      | 13  | 2.0000    | 0.0696         | 1.1769    |
|       |      |     |           |                |           |
|       | H    | 1   | 2.0000    | 7.1896         | 0.0317    |
|       |      | 2   | 2.0000    | 1.6120         | 0.4167    |
|       |      | 3   | 2.0000    | 0.5023         | 0.4113    |
|       |      | 4   | 2.0000    | 0.2097         | -0.2722   |
|       |      | 5   | 2.0000    | 0.1683         | 0.2122    |
|       | C    | 1   | 2.0000    | 233.9861       | 0.0393    |
|       |      | 2   | 2.0000    | 191.1093       | 0.0461    |
|       |      | 3   | 2.0000    | 51.2230        | 0.2507    |
|       |      | 4   | 2.0000    | 42.7414        | 0.3789    |
|       |      | 5   | 2.0000    | 14.7443        | 1.1061    |
|       |      | 6   | 2.0000    | 0.8016         | 2.3528    |
|       |      | 7   | 2.0000    | 0.3994         | 1.4483    |
|       |      | 8   | 2.0000    | 0.3312         | 0.0000    |
|       |      | 9   | 2.0000    | 0.2759         | 0.0000    |
|       |      | 10  | 2.0000    | 0.2377         | 0.8949    |
|       |      | 11  | 2.0000    | 0.1169         | 0.5903    |
|       |      | 12  | 2.0000    | 0.0786         | 0.0000    |
|       |      | 13  | 2.0000    | 0.0696         | 0.5145    |
|       | H    | 1   | 2.0000    | 7.1896         | 0.0288    |
|       |      | 2   | 2.0000    | 1.6120         | 0.4407    |
|       |      | 3   | 2.0000    | 0.5023         | 0.3234    |
|       |      | 4   | 2.0000    | 0.2097         | 0.0000    |
|       |      | 5   | 2.0000    | 0.1683         | 0.0000    |
| LISA5 | --   | --  | --        | --             | --        |
| LISA6 | C    | 1   | 1.0000    | 13.0886        | 1.6392    |
|       |      | 2   | 1.0000    | 2.4356         | 0.0000    |
|       |      | 3   | 1.0000    | 1.9858         | 4.1798    |
|       |      | 4   | 1.0000    | 0.9936         | 1.5988    |
|       |      | 5   | 1.0000    | 0.8363         | 0.0000    |

Continued on next page

Table S18: The basis info of molecule  $\text{CH}_3^-$ .

|       |      |                        | $n_{a,k}$ | $\alpha_{a,k}$ | $c_{a,k}$ |
|-------|------|------------------------|-----------|----------------|-----------|
| Model | Atom | $k$                    |           |                |           |
| NLIS1 | H    | 1                      | 1.0000    | 4.2476         | 0.0000    |
|       |      | 2                      | 1.0000    | 3.4951         | 0.3038    |
|       |      | 3                      | 1.0000    | 1.9499         | 0.5564    |
|       |      | 4                      | 1.0000    | 1.4845         | 0.0000    |
|       |      | 5                      | 1.0000    | 1.2133         | 0.0000    |
|       | C    | 1                      | 2.0000    | 178.8743       | 0.1141    |
|       |      | 2                      | 2.0000    | 40.2184        | 0.7149    |
|       |      | 3                      | 2.0000    | 13.4622        | 1.0199    |
|       |      | 4                      | 2.0000    | 0.6520         | 3.5902    |
|       |      | 5                      | 2.0000    | 0.1729         | 1.7342    |
| H     | 6    | 2.0000                 | 0.0657    | 0.5190         |           |
|       | 1    | 2.0000                 | 12.3993   | 0.0145         |           |
|       | 2    | 2.0000                 | 2.1104    | 0.2694         |           |
|       | 3    | 2.0000                 | 0.7422    | 0.4854         |           |
| NLIS2 | C    | 4                      | 2.0000    | 0.0273         | 0.0001    |
|       |      | 1                      | 2.0000    | 198.2005       | 0.0953    |
|       |      | 2                      | 2.0000    | 44.1341        | 0.6486    |
|       |      | 3                      | 2.0000    | 14.4504        | 1.0759    |
|       | H    | 4                      | 2.0000    | 0.6631         | 1.3703    |
|       |      | 5                      | 2.0000    | 0.6631         | 1.4837    |
|       |      | 6                      | 1.0000    | 1.1230         | 3.0097    |
|       |      | 1                      | 2.0000    | 12.2018        | 0.0150    |
|       |      | 2                      | 2.0000    | 2.0659         | 0.2811    |
|       |      | 3                      | 2.0000    | 0.7249         | 0.4762    |
| NLIS3 | C    | 4                      | 1.0000    | 0.8781         | 0.0000    |
|       |      | 1                      | 2.0000    | 37.9458        | 0.2585    |
|       |      | 2                      | 2.0000    | 13.7124        | 0.8022    |
|       |      | 3                      | 2.0000    | 0.6613         | 0.4577    |
|       | H    | 4                      | 2.0000    | 0.6613         | 2.3998    |
|       |      | 5                      | 1.0000    | 1.1221         | 2.9997    |
|       |      | 6                      | 1.0000    | 15.4746        | 0.7632    |
|       |      | 1                      | 2.0000    | 1.8735         | 0.2411    |
|       |      | 2                      | 2.0000    | 0.7074         | 0.4433    |
|       |      | Continued on next page |           |                |           |

Table S18: The basis info of molecule  $\text{CH}_3^-$ .

|       |      |     | $n_{a,k}$ | $\alpha_{a,k}$ | $c_{a,k}$ |
|-------|------|-----|-----------|----------------|-----------|
| Model | Atom | $k$ |           |                |           |
| NLIS4 | C    | 3   | 1.0000    | 0.9000         | 0.0000    |
|       |      | 4   | 1.0000    | 4.0886         | 0.0886    |
|       |      | 1   | 1.0000    | 12.7838        | 1.0425    |
|       |      | 2   | 1.0000    | 12.7838        | 0.6572    |
|       |      | 3   | 1.0000    | 1.7834         | 2.1311    |
|       |      | 4   | 1.0000    | 1.7834         | 1.7217    |
|       | H    | 5   | 1.0000    | 0.9388         | 1.2430    |
|       |      | 6   | 1.0000    | 1.7834         | 0.8485    |
|       |      | 1   | 1.0000    | 2.5781         | 0.5403    |
|       |      | 2   | 1.0000    | 2.5776         | 0.0000    |
|       |      | 3   | 1.0000    | 2.5776         | 0.0000    |
|       |      | 4   | 1.0000    | 2.5781         | 0.2446    |
| MBIS  | C    | 1   | 1.0000    | 12.2068        | 1.8049    |
|       |      | 2   | 1.0000    | 1.4612         | 6.1151    |
|       | H    | 1   | 1.0000    | 2.7417         | 0.6931    |
| GMBIS | C    | 1   | 1.1380    | 13.1340        | 1.7744    |
|       |      | 2   | 1.0000    | 1.4642         | 6.1646    |
|       | H    | 1   | 1.0380    | 2.6474         | 0.6868    |

## S2.4 $\text{NH}_4^+$

Table S19: The basis info of molecule  $\text{NH}_4^+$ .

| Model | Atom | $k$ | $n_{a,k}$ | $\alpha_{a,k}$ | $c_{a,k}$ |
|-------|------|-----|-----------|----------------|-----------|
| LISA1 | N    | 1   | 2.0000    | 178.0000       | 0.1751    |
|       |      | 2   | 2.0000    | 52.4200        | 0.6243    |
|       |      | 3   | 2.0000    | 19.8700        | 1.0131    |
|       |      | 4   | 2.0000    | 1.2760         | 2.0633    |
|       |      | 5   | 2.0000    | 0.6291         | 3.2935    |
|       |      | 6   | 2.0000    | 0.2857         | 0.5915    |
|       | H    | 1   | 2.0000    | 5.6720         | 0.0593    |
|       |      | 2   | 2.0000    | 1.5050         | 0.3530    |
|       |      | 3   | 2.0000    | 0.5308         | 0.1404    |
|       |      | 4   | 2.0000    | 0.2204         | 0.0074    |
| LISA2 | N    | 1   | 2.0000    | 178.0000       | 0.1750    |
|       |      | 2   | 2.0000    | 52.4200        | 0.6246    |
|       |      | 3   | 2.0000    | 19.8700        | 1.0126    |
|       |      | 4   | 2.0000    | 1.2760         | 2.0701    |
|       |      | 5   | 2.0000    | 0.6291         | 3.2779    |
|       |      | 6   | 2.0000    | 0.2857         | 0.6050    |
|       | H    | 1   | 2.0000    | 5.6720         | 0.0595    |
|       |      | 2   | 2.0000    | 1.5050         | 0.3520    |
|       |      | 3   | 2.0000    | 0.5308         | 0.1422    |
|       |      | 4   | 2.0000    | 0.2204         | 0.0043    |
|       |      | 5   | 1.0000    | 1.0000         | 0.0010    |
| LISA3 | --   | --  | --        | --             | --        |
| LISA4 | N    | 1   | 2.0000    | 289.9075       | 0.0794    |
|       |      | 2   | 2.0000    | 253.6613       | 0.0000    |
|       |      | 3   | 2.0000    | 107.1174       | 0.0626    |
|       |      | 4   | 2.0000    | 64.4812        | 0.2505    |
|       |      | 5   | 2.0000    | 56.9290        | 0.3318    |
|       |      | 6   | 2.0000    | 24.6298        | 0.0000    |
|       |      | 7   | 2.0000    | 20.4266        | 1.0924    |
|       |      | 8   | 2.0000    | 2.4028         | 0.1693    |

Continued on next page

Table S19: The basis info of molecule  $\text{NH}_4^+$ .

| Model | Atom | $k$ | $n_{a,k}$ | $\alpha_{a,k}$ | $c_{a,k}$ |
|-------|------|-----|-----------|----------------|-----------|
|       |      | 9   | 2.0000    | 1.5267         | 0.0000    |
|       |      | 10  | 2.0000    | 1.1847         | 0.0000    |
|       |      | 11  | 2.0000    | 0.9018         | 4.3098    |
|       |      | 12  | 2.0000    | 0.4911         | 0.0000    |
|       |      | 13  | 2.0000    | 0.4324         | 0.0000    |
|       |      | 14  | 2.0000    | 0.3854         | 1.1506    |
|       |      | 15  | 2.0000    | 0.2972         | 0.3025    |
|       |      | 16  | 2.0000    | 0.2087         | 0.0000    |
|       |      | 17  | 2.0000    | 0.1087         | 0.0142    |
|       | H    | 1   | 2.0000    | 7.1896         | 0.0389    |
|       |      | 2   | 2.0000    | 1.6120         | 0.3725    |
|       |      | 3   | 2.0000    | 0.5023         | 0.1481    |
|       |      | 4   | 2.0000    | 0.2097         | 0.0000    |
|       |      | 5   | 2.0000    | 0.1683         | 0.0000    |
| LISA5 | --   | --  | --        | --             | --        |
| LISA6 | N    | 1   | 1.0000    | 15.5442        | 1.5260    |
|       |      | 2   | 1.0000    | 2.4595         | 6.0630    |
|       |      | 3   | 1.0000    | 1.2198         | 0.0000    |
|       |      | 4   | 1.0000    | 1.0679         | 0.0000    |
|       | H    | 1   | 1.0000    | 4.2476         | 0.0000    |
|       |      | 2   | 1.0000    | 3.4951         | 0.4068    |
|       |      | 3   | 1.0000    | 1.9499         | 0.1956    |
|       |      | 4   | 1.0000    | 1.4845         | 0.0000    |
|       |      | 5   | 1.0000    | 1.2133         | 0.0000    |
| NLIS1 | N    | 1   | 2.0000    | 302.8723       | 0.0791    |
|       |      | 2   | 2.0000    | 67.0008        | 0.5831    |
|       |      | 3   | 2.0000    | 21.7351        | 1.1102    |
|       |      | 4   | 2.0000    | 4.5188         | 0.1714    |
|       |      | 5   | 2.0000    | 0.8711         | 4.6797    |
|       |      | 6   | 2.0000    | 0.3143         | 1.1553    |
|       | H    | 1   | 2.0000    | 12.5114        | 0.0136    |
|       |      | 2   | 2.0000    | 2.2099         | 0.2683    |
|       |      | 3   | 2.0000    | 0.7562         | 0.2673    |

Continued on next page

Table S19: The basis info of molecule  $\text{NH}_4^+$ .

| Model | Atom | $k$ | $n_{a,k}$ | $\alpha_{a,k}$ | $c_{a,k}$ |
|-------|------|-----|-----------|----------------|-----------|
| NLIS2 | N    | 4   | 2.0000    | 0.1722         | 0.0062    |
|       |      | 1   | 2.0000    | 110.6568       | 0.4277    |
|       |      | 2   | 2.0000    | 25.1643        | 1.3012    |
|       |      | 3   | 2.0000    | 0.8177         | 0.4615    |
|       |      | 4   | 2.0000    | 0.8177         | 1.5946    |
|       |      | 5   | 2.0000    | 0.8177         | 1.2011    |
|       |      | 6   | 1.0000    | 2.0843         | 2.7738    |
|       | H    | 1   | 2.0000    | 2.0524         | 0.2306    |
|       |      | 2   | 2.0000    | 0.6981         | 0.1113    |
|       |      | 3   | 2.0000    | 0.6981         | 0.1368    |
|       |      | 4   | 1.0000    | 4.1228         | 0.0810    |
| NLIS3 | N    | 1   | 2.0000    | 63.0040        | 0.2875    |
|       |      | 2   | 2.0000    | 21.6972        | 0.9741    |
|       |      | 3   | 2.0000    | 0.8177         | 1.1645    |
|       |      | 4   | 2.0000    | 0.8177         | 2.2291    |
|       |      | 5   | 1.0000    | 2.0590         | 2.6083    |
|       |      | 6   | 1.0000    | 20.5671        | 0.4919    |
|       | H    | 1   | 2.0000    | 2.0605         | 0.2306    |
|       |      | 2   | 2.0000    | 0.6997         | 0.2521    |
|       |      | 3   | 1.0000    | 4.1701         | 0.0782    |
|       |      | 4   | 1.0000    | 0.0000         | 0.0000    |
| NLIS4 | N    | 1   | 1.0000    | 15.6837        | 0.8967    |
|       |      | 2   | 1.0000    | 15.6837        | 0.6250    |
|       |      | 3   | 1.0000    | 2.2432         | 2.5588    |
|       |      | 4   | 1.0000    | 2.2432         | 2.2218    |
|       |      | 5   | 1.0000    | 2.2432         | 1.5067    |
|       |      | 6   | 1.0000    | 15.6837        | 0.0676    |
|       | H    | 1   | 1.0000    | 3.0250         | 0.1159    |
|       |      | 2   | 1.0000    | 3.0250         | 0.0785    |
|       |      | 3   | 1.0000    | 3.0250         | 0.2543    |
|       |      | 4   | 1.0000    | 3.0250         | 0.0818    |
| MBIS  | N    | 1   | 1.0000    | 15.6837        | 1.5893    |
|       |      | 2   | 1.0000    | 2.2432         | 6.2873    |

Continued on next page



Table S19: The basis info of molecule  $\text{NH}_4^+$ .

|       |      |     | $n_{a,k}$ | $\alpha_{a,k}$ | $c_{a,k}$ |
|-------|------|-----|-----------|----------------|-----------|
| Model | Atom | $k$ |           |                |           |
|       | H    | 1   | 1.0000    | 3.0250         | 0.5305    |
| GMBIS | N    | 1   | 1.1720    | 17.8939        | 1.5629    |
|       |      | 2   | 1.0000    | 2.2485         | 6.3102    |
|       | H    | 1   | 1.0380    | 2.9106         | 0.5314    |

## S2.5 NH<sub>3</sub>

Table S20: The basis info of molecule NH<sub>3</sub>.

| Model | Atom | $k$ | $n_{a,k}$ | $\alpha_{a,k}$ | $c_{a,k}$ |
|-------|------|-----|-----------|----------------|-----------|
| LISA1 | N    | 1   | 2.0000    | 178.0000       | 0.1744    |
|       |      | 2   | 2.0000    | 52.4200        | 0.6305    |
|       |      | 3   | 2.0000    | 19.8700        | 1.0056    |
|       |      | 4   | 2.0000    | 1.2760         | 2.2167    |
|       |      | 5   | 2.0000    | 0.6291         | 2.5233    |
|       |      | 6   | 2.0000    | 0.2857         | 1.4345    |
|       | H    | 1   | 2.0000    | 5.6720         | 0.0573    |
|       |      | 2   | 2.0000    | 1.5050         | 0.3984    |
|       |      | 3   | 2.0000    | 0.5308         | 0.1341    |
|       |      | 4   | 2.0000    | 0.2204         | 0.0819    |
| LISA2 | N    | 1   | 2.0000    | 178.0000       | 0.1743    |
|       |      | 2   | 2.0000    | 52.4200        | 0.6309    |
|       |      | 3   | 2.0000    | 19.8700        | 1.0048    |
|       |      | 4   | 2.0000    | 1.2760         | 2.2274    |
|       |      | 5   | 2.0000    | 0.6291         | 2.4953    |
|       |      | 6   | 2.0000    | 0.2857         | 1.4596    |
|       | H    | 1   | 2.0000    | 5.6720         | 0.0600    |
|       |      | 2   | 2.0000    | 1.5050         | 0.3816    |
|       |      | 3   | 2.0000    | 0.5308         | 0.1695    |
|       |      | 4   | 2.0000    | 0.2204         | 0.0328    |
|       |      | 5   | 1.0000    | 1.0000         | 0.0254    |
| LISA3 | N    | 1   | 2.0000    | 289.9075       | 0.3458    |
|       |      | 2   | 2.0000    | 253.6613       | -0.3741   |
|       |      | 3   | 2.0000    | 107.1174       | 0.6048    |
|       |      | 4   | 2.0000    | 64.4812        | -2.3706   |
|       |      | 5   | 2.0000    | 56.9290        | 2.7224    |
|       |      | 6   | 2.0000    | 24.6298        | -0.5161   |
|       |      | 7   | 2.0000    | 20.4266        | 1.4000    |
|       |      | 8   | 2.0000    | 2.4028         | 0.1976    |
|       |      | 9   | 2.0000    | 1.5267         | 2.1058    |

Continued on next page

Table S20: The basis info of molecule NH<sub>3</sub>.

|       |       |     | $n_{a,k}$ | $\alpha_{a,k}$ | $c_{a,k}$ |        |
|-------|-------|-----|-----------|----------------|-----------|--------|
| Model | Atom  | $k$ |           |                |           |        |
|       |       | 10  | 2.0000    | 1.1847         | -6.7108   |        |
|       |       | 11  | 2.0000    | 0.9018         | 11.7826   |        |
|       |       | 12  | 2.0000    | 0.4911         | -32.9790  |        |
|       |       | 13  | 2.0000    | 0.4324         | 60.2220   |        |
|       |       | 14  | 2.0000    | 0.3854         | -33.1133  |        |
|       |       | 15  | 2.0000    | 0.2972         | 4.5674    |        |
|       |       | 16  | 2.0000    | 0.2087         | 0.0691    |        |
|       |       | 17  | 2.0000    | 0.1087         | 0.0894    |        |
|       | H     | 1   | 2.0000    | 7.1896         | 0.0410    |        |
|       |       | 2   | 2.0000    | 1.6120         | 0.3865    |        |
|       |       | 3   | 2.0000    | 0.5023         | 0.2307    |        |
|       |       | 4   | 2.0000    | 0.2097         | -0.0416   |        |
|       |       | 5   | 2.0000    | 0.1683         | 0.0358    |        |
|       | LISA4 | N   | 1         | 2.0000         | 289.9075  | 0.0782 |
|       |       |     | 2         | 2.0000         | 253.6613  | 0.0000 |
|       |       |     | 3         | 2.0000         | 107.1174  | 0.0835 |
|       |       |     | 4         | 2.0000         | 64.4812   | 0.1038 |
| 5     |       |     | 2.0000    | 56.9290        | 0.4715    |        |
| 6     |       |     | 2.0000    | 24.6298        | 0.0000    |        |
| 7     |       |     | 2.0000    | 20.4266        | 1.0761    |        |
| 8     |       |     | 2.0000    | 2.4028         | 0.2191    |        |
| 9     |       |     | 2.0000    | 1.5267         | 0.0000    |        |
| 10    |       |     | 2.0000    | 1.1847         | 0.0000    |        |
| 11    |       |     | 2.0000    | 0.9018         | 4.1126    |        |
| 12    |       |     | 2.0000    | 0.4911         | 0.0000    |        |
| 13    |       |     | 2.0000    | 0.4324         | 0.0000    |        |
| 14    |       |     | 2.0000    | 0.3854         | 0.1718    |        |
| 15    |       |     | 2.0000    | 0.2972         | 1.6025    |        |
| 16    |       |     | 2.0000    | 0.2087         | 0.0000    |        |
| 17    |       |     | 2.0000    | 0.1087         | 0.1212    |        |
|       | H     | 1   | 2.0000    | 7.1896         | 0.0405    |        |
|       |       | 2   | 2.0000    | 1.6120         | 0.3912    |        |
|       |       | 3   | 2.0000    | 0.5023         | 0.2155    |        |

Continued on next page

Table S20: The basis info of molecule NH<sub>3</sub>.

| Model | Atom | $k$ | $n_{a,k}$ | $\alpha_{a,k}$ | $c_{a,k}$ |
|-------|------|-----|-----------|----------------|-----------|
|       |      | 4   | 2.0000    | 0.2097         | 0.0000    |
|       |      | 5   | 2.0000    | 0.1683         | 0.0062    |
| LISA5 | --   | --  | --        | --             | --        |
| LISA6 | N    | 1   | 1.0000    | 15.5442        | 1.5418    |
|       |      | 2   | 1.0000    | 2.4595         | 5.6992    |
|       |      | 3   | 1.0000    | 1.2198         | 0.4989    |
|       |      | 4   | 1.0000    | 1.0679         | 0.0000    |
|       | H    | 1   | 1.0000    | 4.2476         | 0.0000    |
|       |      | 2   | 1.0000    | 3.4951         | 0.3416    |
|       |      | 3   | 1.0000    | 1.9499         | 0.4115    |
|       |      | 4   | 1.0000    | 1.4845         | 0.0000    |
|       |      | 5   | 1.0000    | 1.2133         | 0.0000    |
| NLIS1 | N    | 1   | 2.0000    | 224.6030       | 0.1341    |
|       |      | 2   | 2.0000    | 50.9597        | 0.7831    |
|       |      | 3   | 2.0000    | 17.5823        | 0.9398    |
|       |      | 4   | 2.0000    | 0.9373         | 4.2442    |
|       |      | 5   | 2.0000    | 0.3048         | 1.8174    |
|       |      | 6   | 2.0000    | 0.1100         | 0.1240    |
|       | H    | 1   | 2.0000    | 13.5566        | 0.0126    |
|       |      | 2   | 2.0000    | 2.3406         | 0.2532    |
|       |      | 3   | 2.0000    | 0.8190         | 0.3281    |
|       |      | 4   | 2.0000    | 0.2961         | 0.0586    |
| NLIS2 | N    | 1   | 2.0000    | 108.8555       | 0.4391    |
|       |      | 2   | 2.0000    | 24.8295        | 1.3034    |
|       |      | 3   | 2.0000    | 0.8984         | 0.2081    |
|       |      | 4   | 2.0000    | 0.8984         | 1.2717    |
|       |      | 5   | 2.0000    | 0.8984         | 1.1623    |
|       |      | 6   | 1.0000    | 1.8338         | 3.6619    |
|       | H    | 1   | 2.0000    | 11.4046        | 0.0170    |
|       |      | 2   | 2.0000    | 2.0841         | 0.3034    |
|       |      | 3   | 2.0000    | 0.6670         | 0.3087    |
|       |      | 4   | 1.0000    | 1.3600         | 0.0221    |
| NLIS3 | N    | 1   | 2.0000    | 108.7574       | 0.4397    |

Continued on next page

Table S20: The basis info of molecule NH<sub>3</sub>.

|       |      |     | $n_{a,k}$ | $\alpha_{a,k}$ | $c_{a,k}$ |
|-------|------|-----|-----------|----------------|-----------|
| Model | Atom | $k$ |           |                |           |
| NLIS4 |      | 2   | 2.0000    | 24.8103        | 1.3034    |
|       |      | 3   | 2.0000    | 0.8984         | 0.8893    |
|       |      | 4   | 2.0000    | 0.8984         | 1.7631    |
|       |      | 5   | 1.0000    | 1.8326         | 2.5981    |
|       |      | 6   | 1.0000    | 1.8326         | 1.0509    |
|       | H    | 1   | 2.0000    | 2.0459         | 0.1568    |
|       |      | 2   | 2.0000    | 0.6633         | 0.1404    |
|       |      | 3   | 1.0000    | 1.0592         | 0.0059    |
|       |      | 4   | 1.0000    | 2.7228         | 0.3487    |
|       | N    | 1   | 1.0000    | 15.2968        | 0.9880    |
|       |      | 2   | 1.0000    | 15.2968        | 0.6649    |
|       |      | 3   | 1.0000    | 2.0938         | 2.3583    |
|       |      | 4   | 1.0000    | 2.0938         | 2.0435    |
|       |      | 5   | 1.0000    | 2.0938         | 1.4325    |
|       |      | 6   | 1.0000    | 2.0938         | 0.5885    |
|       | H    | 1   | 1.0000    | 1.0025         | 0.0127    |
|       |      | 2   | 1.0000    | 2.7694         | 0.0909    |
|       |      | 3   | 1.0000    | 2.7694         | 0.3213    |
|       |      | 4   | 1.0000    | 2.7694         | 0.2163    |
| MBIS  | N    | 1   | 1.0000    | 15.2486        | 1.6603    |
|       |      | 2   | 1.0000    | 2.0769         | 6.4482    |
|       | H    | 1   | 1.0000    | 2.7534         | 0.6302    |
| GMBIS | N    | 1   | 1.1720    | 17.3441        | 1.6304    |
|       |      | 2   | 1.0000    | 2.0797         | 6.4867    |
|       | H    | 1   | 1.0380    | 2.6507         | 0.6274    |

## S2.6 $\text{NH}_2^-$

Table S21: The basis info of molecule  $\text{NH}_2^-$ .

| Model | Atom | $k$ | $n_{a,k}$ | $\alpha_{a,k}$ | $c_{a,k}$ |
|-------|------|-----|-----------|----------------|-----------|
| LISA1 | N    | 1   | 2.0000    | 178.0000       | 0.1711    |
|       |      | 2   | 2.0000    | 52.4200        | 0.6505    |
|       |      | 3   | 2.0000    | 19.8700        | 0.9766    |
|       |      | 4   | 2.0000    | 1.2760         | 2.6786    |
|       |      | 5   | 2.0000    | 0.6291         | 1.0432    |
|       |      | 6   | 2.0000    | 0.2857         | 2.6629    |
|       | H    | 1   | 2.0000    | 5.6720         | 0.0531    |
|       |      | 2   | 2.0000    | 1.5050         | 0.4308    |
|       |      | 3   | 2.0000    | 0.5308         | 0.0000    |
|       |      | 4   | 2.0000    | 0.2204         | 0.4246    |
| LISA2 | N    | 1   | 2.0000    | 178.0000       | 0.1727    |
|       |      | 2   | 2.0000    | 52.4200        | 0.6427    |
|       |      | 3   | 2.0000    | 19.8700        | 0.9894    |
|       |      | 4   | 2.0000    | 1.2760         | 2.4979    |
|       |      | 5   | 2.0000    | 0.6291         | 1.4260    |
|       |      | 6   | 2.0000    | 0.2857         | 2.4440    |
|       | H    | 1   | 2.0000    | 5.6720         | 0.0485    |
|       |      | 2   | 2.0000    | 1.5050         | 0.4201    |
|       |      | 3   | 2.0000    | 0.5308         | 0.0495    |
|       |      | 4   | 2.0000    | 0.2204         | 0.0000    |
|       |      | 5   | 1.0000    | 1.0000         | 0.3955    |
| LISA3 | N    | 1   | 2.0000    | 289.9075       | 0.3565    |
|       |      | 2   | 2.0000    | 253.6613       | -0.3898   |
|       |      | 3   | 2.0000    | 107.1174       | 0.6389    |
|       |      | 4   | 2.0000    | 64.4812        | -2.5954   |
|       |      | 5   | 2.0000    | 56.9290        | 2.9479    |
|       |      | 6   | 2.0000    | 24.6298        | -0.6262   |
|       |      | 7   | 2.0000    | 20.4266        | 1.4898    |
|       |      | 8   | 2.0000    | 2.4028         | -0.4139   |
|       |      | 9   | 2.0000    | 1.5267         | 7.8642    |

Continued on next page

Table S21: The basis info of molecule  $\text{NH}_2^-$ .

| Model | Atom | $k$ | $n_{a,k}$ | $\alpha_{a,k}$ | $c_{a,k}$ |
|-------|------|-----|-----------|----------------|-----------|
|       |      |     |           |                |           |
| LISA4 |      | 10  | 2.0000    | 1.1847         | -20.5449  |
|       |      | 11  | 2.0000    | 0.9018         | 27.1950   |
|       |      | 12  | 2.0000    | 0.4911         | -170.8964 |
|       |      | 13  | 2.0000    | 0.4324         | 381.9004  |
|       |      | 14  | 2.0000    | 0.3854         | -262.6818 |
|       |      | 15  | 2.0000    | 0.2972         | 49.4596   |
|       |      | 16  | 2.0000    | 0.2087         | -6.3385   |
|       |      | 17  | 2.0000    | 0.1087         | 1.1675    |
|       | H    | 1   | 2.0000    | 7.1896         | 0.0398    |
|       |      | 2   | 2.0000    | 1.6120         | 0.3790    |
|       |      | 3   | 2.0000    | 0.5023         | 0.3131    |
|       |      | 4   | 2.0000    | 0.2097         | -0.1223   |
|       |      | 5   | 2.0000    | 0.1683         | 0.1239    |
|       | N    | 1   | 2.0000    | 289.9075       | 0.0780    |
|       |      | 2   | 2.0000    | 253.6613       | 0.0000    |
|       |      | 3   | 2.0000    | 107.1174       | 0.0947    |
|       |      | 4   | 2.0000    | 64.4812        | 0.0000    |
|       |      | 5   | 2.0000    | 56.9290        | 0.5776    |
|       |      | 6   | 2.0000    | 24.6298        | 0.0000    |
|       |      | 7   | 2.0000    | 20.4266        | 1.0592    |
|       |      | 8   | 2.0000    | 2.4028         | 0.2730    |
|       |      | 9   | 2.0000    | 1.5267         | 0.0000    |
|       |      | 10  | 2.0000    | 1.1847         | 0.2077    |
|       |      | 11  | 2.0000    | 0.9018         | 3.4755    |
|       |      | 12  | 2.0000    | 0.4911         | 0.0000    |
|       |      | 13  | 2.0000    | 0.4324         | 0.0000    |
|       |      | 14  | 2.0000    | 0.3854         | 0.5453    |
|       |      | 15  | 2.0000    | 0.2972         | 1.3233    |
|       |      | 16  | 2.0000    | 0.2087         | 0.0000    |
|       |      | 17  | 2.0000    | 0.1087         | 0.9136    |
|       | H    | 1   | 2.0000    | 7.1896         | 0.0390    |
|       |      | 2   | 2.0000    | 1.6120         | 0.3852    |
|       |      | 3   | 2.0000    | 0.5023         | 0.2858    |

Continued on next page

Table S21: The basis info of molecule  $\text{NH}_2^-$ .

| Model | Atom | $k$ | $n_{a,k}$ | $\alpha_{a,k}$ | $c_{a,k}$ |
|-------|------|-----|-----------|----------------|-----------|
|       |      | 4   | 2.0000    | 0.2097         | 0.0000    |
|       |      | 5   | 2.0000    | 0.1683         | 0.0161    |
| LISA5 | --   | --  | --        | --             | --        |
| LISA6 | N    | 1   | 1.0000    | 15.5442        | 1.5952    |
|       |      | 2   | 1.0000    | 2.4595         | 4.5974    |
|       |      | 3   | 1.0000    | 1.2198         | 2.2751    |
|       |      | 4   | 1.0000    | 1.0679         | 0.0000    |
|       | H    | 1   | 1.0000    | 4.2476         | 0.0000    |
|       |      | 2   | 1.0000    | 3.4951         | 0.3001    |
|       |      | 3   | 1.0000    | 1.9499         | 0.4662    |
|       |      | 4   | 1.0000    | 1.4845         | 0.0000    |
|       |      | 5   | 1.0000    | 1.2133         | 0.0000    |
| NLIS1 | N    | 1   | 2.0000    | 229.0379       | 0.1299    |
|       |      | 2   | 2.0000    | 51.9479        | 0.7689    |
|       |      | 3   | 2.0000    | 17.9199        | 0.9547    |
|       |      | 4   | 2.0000    | 0.9811         | 3.8207    |
|       |      | 5   | 2.0000    | 0.3141         | 2.0182    |
|       |      | 6   | 2.0000    | 0.1078         | 0.8395    |
|       | H    | 1   | 2.0000    | 8.3927         | 0.0289    |
|       |      | 2   | 2.0000    | 1.7932         | 0.3491    |
|       |      | 3   | 2.0000    | 0.5544         | 0.3338    |
|       |      | 4   | 2.0000    | 0.0687         | 0.0222    |
| NLIS2 | N    | 1   | 2.0000    | 260.0949       | 0.1040    |
|       |      | 2   | 2.0000    | 58.4598        | 0.6794    |
|       |      | 3   | 2.0000    | 19.6645        | 1.0380    |
|       |      | 4   | 2.0000    | 1.0493         | 2.7574    |
|       |      | 5   | 2.0000    | 0.5522         | 0.9948    |
|       |      | 6   | 1.0000    | 1.3110         | 2.9538    |
|       | H    | 1   | 2.0000    | 13.0010        | 0.0135    |
|       |      | 2   | 2.0000    | 2.2360         | 0.2634    |
|       |      | 3   | 2.0000    | 0.7262         | 0.3692    |
|       |      | 4   | 1.0000    | 1.2503         | 0.0902    |
| NLIS3 | N    | 1   | 2.0000    | 109.7802       | 0.4342    |

Continued on next page



Table S21: The basis info of molecule  $\text{NH}_2^-$ .

| Model | Atom | $k$ | $n_{a,k}$ | $\alpha_{a,k}$ | $c_{a,k}$ |
|-------|------|-----|-----------|----------------|-----------|
|       |      |     |           |                |           |
| NLIS4 |      | 2   | 2.0000    | 25.0710        | 1.3015    |
|       |      | 3   | 2.0000    | 0.8917         | 0.8921    |
|       |      | 4   | 2.0000    | 0.8917         | 1.7275    |
|       |      | 5   | 1.0000    | 1.3007         | 2.8494    |
|       |      | 6   | 1.0000    | 2.4147         | 1.3241    |
|       | H    | 1   | 2.0000    | 3.0455         | 0.1859    |
|       |      | 2   | 2.0000    | 0.8748         | 0.4075    |
|       |      | 3   | 1.0000    | 1.4681         | 0.0914    |
|       |      | 4   | 1.0000    | 1.4681         | 0.0504    |
|       | N    | 1   | 1.0000    | 15.1838        | 1.0402    |
|       |      | 2   | 1.0000    | 15.1838        | 0.6340    |
|       |      | 3   | 1.0000    | 2.1337         | 3.1522    |
|       |      | 4   | 1.0000    | 1.1107         | 1.3136    |
|       |      | 5   | 1.0000    | 2.1337         | 1.2959    |
|       |      | 6   | 1.0000    | 2.1337         | 1.0968    |
|       | H    | 1   | 1.0000    | 1.1872         | 0.0296    |
|       |      | 2   | 1.0000    | 1.1872         | 0.0364    |
|       |      | 3   | 1.0000    | 2.6481         | 0.3243    |
|       |      | 4   | 1.0000    | 2.6481         | 0.3435    |
| MBIS  | N    | 1   | 1.0000    | 14.3135        | 1.8090    |
|       |      | 2   | 1.0000    | 1.7523         | 6.9344    |
|       | H    | 1   | 1.0000    | 2.6513         | 0.6284    |
| GMBIS | N    | 1   | 1.1720    | 16.2111        | 1.7675    |
|       |      | 2   | 1.0000    | 1.7562         | 6.9946    |
|       | H    | 1   | 1.0380    | 2.5720         | 0.6190    |

## S2.7 H<sub>3</sub>O<sup>+</sup>

Table S22: The basis info of molecule H<sub>3</sub>O<sup>+</sup>.

| Model | Atom | <i>k</i> | $n_{a,k}$ | $\alpha_{a,k}$ | $c_{a,k}$ |
|-------|------|----------|-----------|----------------|-----------|
| LISA1 | O    | 1        | 2.0000    | 220.1000       | 0.1985    |
|       |      | 2        | 2.0000    | 65.6600        | 0.6308    |
|       |      | 3        | 2.0000    | 25.9800        | 0.9884    |
|       |      | 4        | 2.0000    | 1.6850         | 2.8912    |
|       |      | 5        | 2.0000    | 0.6860         | 3.6758    |
|       |      | 6        | 2.0000    | 0.2311         | 0.3084    |
|       | H    | 1        | 2.0000    | 5.6720         | 0.0621    |
|       |      | 2        | 2.0000    | 1.5050         | 0.2748    |
|       |      | 3        | 2.0000    | 0.5308         | 0.0987    |
|       |      | 4        | 2.0000    | 0.2204         | 0.0000    |
| LISA2 | O    | 1        | 2.0000    | 220.1000       | 0.1986    |
|       |      | 2        | 2.0000    | 65.6600        | 0.6308    |
|       |      | 3        | 2.0000    | 25.9800        | 0.9884    |
|       |      | 4        | 2.0000    | 1.6850         | 2.8902    |
|       |      | 5        | 2.0000    | 0.6860         | 3.6779    |
|       |      | 6        | 2.0000    | 0.2311         | 0.3062    |
|       | H    | 1        | 2.0000    | 5.6720         | 0.0621    |
|       |      | 2        | 2.0000    | 1.5050         | 0.2746    |
|       |      | 3        | 2.0000    | 0.5308         | 0.0990    |
|       |      | 4        | 2.0000    | 0.2204         | 0.0000    |
|       |      | 5        | 1.0000    | 1.0000         | 0.0002    |
| LISA3 | --   | --       | --        | --             | --        |
| LISA4 | O    | 1        | 2.0000    | 385.6603       | 0.0789    |
|       |      | 2        | 2.0000    | 143.8070       | 0.0373    |
|       |      | 3        | 2.0000    | 85.6482        | 0.5512    |
|       |      | 4        | 2.0000    | 33.0976        | 0.0000    |
|       |      | 5        | 2.0000    | 28.5587        | 1.1226    |
|       |      | 6        | 2.0000    | 2.8863         | 0.6305    |
|       |      | 7        | 2.0000    | 2.3338         | 0.0000    |
|       |      | 8        | 2.0000    | 1.9709         | 0.0000    |

Continued on next page

Table S22: The basis info of molecule  $\text{H}_3\text{O}^+$ .

| Model | Atom | $k$ | $n_{a,k}$ | $\alpha_{a,k}$ | $c_{a,k}$ |
|-------|------|-----|-----------|----------------|-----------|
|       | H    | 9   | 2.0000    | 1.1642         | 4.2839    |
|       |      | 10  | 2.0000    | 0.4925         | 1.3359    |
|       |      | 11  | 2.0000    | 0.3884         | 0.6440    |
|       |      | 12  | 2.0000    | 0.1503         | 0.0290    |
|       |      | 1   | 2.0000    | 7.1896         | 0.0427    |
|       |      | 2   | 2.0000    | 1.6120         | 0.2979    |
|       |      | 3   | 2.0000    | 0.5023         | 0.0882    |
|       |      | 4   | 2.0000    | 0.2097         | 0.0000    |
|       |      | 5   | 2.0000    | 0.1683         | 0.0000    |
| LISA5 | --   | --  | --        | --             | --        |
| LISA6 | O    | 1   | 1.0000    | 17.9859        | 1.5104    |
|       |      | 2   | 1.0000    | 2.8225         | 6.7741    |
|       |      | 3   | 1.0000    | 1.4828         | 0.3489    |
|       |      | 4   | 1.0000    | 1.2932         | 0.0000    |
|       | H    | 1   | 1.0000    | 4.2476         | 0.0000    |
|       |      | 2   | 1.0000    | 3.4951         | 0.3755    |
|       |      | 3   | 1.0000    | 1.9499         | 0.0801    |
|       |      | 4   | 1.0000    | 1.4845         | 0.0000    |
|       |      | 5   | 1.0000    | 1.2133         | 0.0000    |
| NLIS1 | O    | 1   | 2.0000    | 405.8804       | 0.0769    |
|       |      | 2   | 2.0000    | 89.6396        | 0.5783    |
|       |      | 3   | 2.0000    | 28.9723        | 1.1202    |
|       |      | 4   | 2.0000    | 3.2675         | 0.6224    |
|       |      | 5   | 2.0000    | 1.1094         | 4.6823    |
|       |      | 6   | 2.0000    | 0.4066         | 1.6321    |
|       | H    | 1   | 2.0000    | 13.1110        | 0.0118    |
|       |      | 2   | 2.0000    | 2.4098         | 0.2196    |
|       |      | 3   | 2.0000    | 0.7823         | 0.1926    |
|       |      | 4   | 2.0000    | 0.1372         | 0.0053    |
| NLIS2 | O    | 1   | 2.0000    | 151.5622       | 0.4053    |
|       |      | 2   | 2.0000    | 34.5264        | 1.2911    |
|       |      | 3   | 2.0000    | 1.1418         | 1.0984    |
|       |      | 4   | 2.0000    | 1.1418         | 1.8453    |

Continued on next page

Table S22: The basis info of molecule  $\text{H}_3\text{O}^+$ .

| Model | Atom | $k$ | $n_{a,k}$ | $\alpha_{a,k}$ | $c_{a,k}$ |
|-------|------|-----|-----------|----------------|-----------|
| NLIS3 | H    | 5   | 2.0000    | 0.4099         | 0.7969    |
|       |      | 6   | 1.0000    | 2.5764         | 3.2791    |
|       |      | 1   | 2.0000    | 2.3086         | 0.1556    |
|       |      | 2   | 2.0000    | 0.7496         | 0.1542    |
|       |      | 3   | 2.0000    | 0.1189         | 0.0023    |
|       |      | 4   | 1.0000    | 3.6116         | 0.1159    |
|       | O    | 1   | 2.0000    | 94.2495        | 0.2865    |
|       |      | 2   | 2.0000    | 31.4433        | 1.0475    |
|       |      | 3   | 2.0000    | 1.0902         | 1.0657    |
|       |      | 4   | 2.0000    | 1.0902         | 1.4549    |
|       |      | 5   | 1.0000    | 2.4015         | 4.4982    |
|       |      | 6   | 1.0000    | 25.6810        | 0.3640    |
| NLIS4 | H    | 1   | 2.0000    | 2.4412         | 0.1771    |
|       |      | 2   | 2.0000    | 0.8103         | 0.2067    |
|       |      | 3   | 1.0000    | 0.8212         | 0.0002    |
|       |      | 4   | 1.0000    | 4.8518         | 0.0438    |
|       | O    | 1   | 1.0000    | 17.9255        | 0.8747    |
|       |      | 2   | 1.0000    | 17.9255        | 0.6025    |
|       |      | 3   | 1.0000    | 2.5315         | 3.0516    |
|       |      | 4   | 1.0000    | 2.5315         | 2.4914    |
|       |      | 5   | 1.0000    | 2.5315         | 1.6443    |
|       |      | 6   | 1.0000    | 17.9255        | 0.1209    |
| MBIS  | H    | 1   | 1.0000    | 3.1501         | 0.0505    |
|       |      | 2   | 1.0000    | 3.1501         | 0.1140    |
|       | O    | 1   | 1.0000    | 17.9255        | 1.5981    |
|       |      | 2   | 1.0000    | 2.5315         | 7.1873    |
| GMBIS | H    | 1   | 1.0000    | 3.1501         | 0.4049    |
|       |      | 2   | 1.0000    | 2.5386         | 7.2135    |
|       | O    | 1   | 1.1720    | 20.9959        | 1.5678    |
|       |      | 2   | 1.0000    | 2.5386         | 7.2135    |
| GMBIS | H    | 1   | 1.0380    | 3.0337         | 0.4062    |
|       |      | 2   | 1.0000    | 2.5386         | 7.2135    |

## S2.8 H<sub>2</sub>O

Table S23: The basis info of molecule H<sub>2</sub>O.

| Model | Atom | $k$ | $n_{a,k}$ | $\alpha_{a,k}$ | $c_{a,k}$ |
|-------|------|-----|-----------|----------------|-----------|
| LISA1 | O    | 1   | 2.0000    | 220.1000       | 0.1982    |
|       |      | 2   | 2.0000    | 65.6600        | 0.6363    |
|       |      | 3   | 2.0000    | 25.9800        | 0.9825    |
|       |      | 4   | 2.0000    | 1.6850         | 2.9057    |
|       |      | 5   | 2.0000    | 0.6860         | 3.3739    |
|       |      | 6   | 2.0000    | 0.2311         | 0.7270    |
|       | H    | 1   | 2.0000    | 5.6720         | 0.0668    |
|       |      | 2   | 2.0000    | 1.5050         | 0.3172    |
|       |      | 3   | 2.0000    | 0.5308         | 0.1752    |
|       |      | 4   | 2.0000    | 0.2204         | 0.0290    |
| LISA2 | O    | 1   | 2.0000    | 220.1000       | 0.1982    |
|       |      | 2   | 2.0000    | 65.6600        | 0.6364    |
|       |      | 3   | 2.0000    | 25.9800        | 0.9823    |
|       |      | 4   | 2.0000    | 1.6850         | 2.9073    |
|       |      | 5   | 2.0000    | 0.6860         | 3.3686    |
|       |      | 6   | 2.0000    | 0.2311         | 0.7336    |
|       | H    | 1   | 2.0000    | 5.6720         | 0.0686    |
|       |      | 2   | 2.0000    | 1.5050         | 0.3063    |
|       |      | 3   | 2.0000    | 0.5308         | 0.1974    |
|       |      | 4   | 2.0000    | 0.2204         | 0.0001    |
|       |      | 5   | 1.0000    | 1.0000         | 0.0143    |
| LISA3 | O    | 1   | 2.0000    | 385.6603       | 0.0797    |
|       |      | 2   | 2.0000    | 143.8070       | 0.0346    |
|       |      | 3   | 2.0000    | 85.6482        | 0.5514    |
|       |      | 4   | 2.0000    | 33.0976        | 0.1071    |
|       |      | 5   | 2.0000    | 28.5587        | 1.0034    |
|       |      | 6   | 2.0000    | 2.8863         | 1.7867    |
|       |      | 7   | 2.0000    | 2.3338         | -2.8937   |
|       |      | 8   | 2.0000    | 1.9709         | 1.9272    |
|       |      | 9   | 2.0000    | 1.1642         | 4.0626    |

Continued on next page

Table S23: The basis info of molecule H<sub>2</sub>O.

|                        |       |     | $n_{a,k}$ | $\alpha_{a,k}$ | $c_{a,k}$ |        |
|------------------------|-------|-----|-----------|----------------|-----------|--------|
| Model                  | Atom  | $k$ |           |                |           |        |
| LISA4                  |       | 10  | 2.0000    | 0.4925         | 0.4192    |        |
|                        |       | 11  | 2.0000    | 0.3884         | 1.6069    |        |
|                        |       | 12  | 2.0000    | 0.1503         | 0.1428    |        |
|                        |       | H   | 1         | 2.0000         | 7.1896    | 0.0474 |
|                        |       | 2   | 2.0000    | 1.6120         | 0.3297    |        |
|                        |       | 3   | 2.0000    | 0.5023         | 0.2030    |        |
|                        |       | 4   | 2.0000    | 0.2097         | -0.0385   |        |
|                        |       | 5   | 2.0000    | 0.1683         | 0.0443    |        |
|                        | O     | 1   | 2.0000    | 385.6603       | 0.0802    |        |
|                        |       | 2   | 2.0000    | 143.8070       | 0.0291    |        |
|                        |       | 3   | 2.0000    | 85.6482        | 0.5650    |        |
|                        |       | 4   | 2.0000    | 33.0976        | 0.0000    |        |
|                        |       | 5   | 2.0000    | 28.5587        | 1.1132    |        |
|                        |       | 6   | 2.0000    | 2.8863         | 0.6602    |        |
|                        |       | 7   | 2.0000    | 2.3338         | 0.0000    |        |
| LISA5                  |       | 8   | 2.0000    | 1.9709         | 0.0000    |        |
|                        |       | 9   | 2.0000    | 1.1642         | 4.1916    |        |
|                        |       | 10  | 2.0000    | 0.4925         | 0.5244    |        |
|                        |       | 11  | 2.0000    | 0.3884         | 1.5145    |        |
|                        |       | 12  | 2.0000    | 0.1503         | 0.1496    |        |
|                        | H     | 1   | 2.0000    | 7.1896         | 0.0467    |        |
|                        |       | 2   | 2.0000    | 1.6120         | 0.3346    |        |
|                        |       | 3   | 2.0000    | 0.5023         | 0.1876    |        |
|                        |       | 4   | 2.0000    | 0.2097         | 0.0000    |        |
|                        |       | 5   | 2.0000    | 0.1683         | 0.0171    |        |
|                        | LISA5 | --  | --        | --             | --        | --     |
|                        | LISA6 | O   | 1         | 1.0000         | 17.9859   | 1.5342 |
|                        |       |     | 2         | 1.0000         | 2.8225    | 6.2438 |
|                        |       |     | 3         | 1.0000         | 1.4828    | 0.9999 |
|                        |       |     | 4         | 1.0000         | 1.2932    | 0.0000 |
| H                      |       | 1   | 1.0000    | 4.2476         | 0.0000    |        |
|                        |       | 2   | 1.0000    | 3.4951         | 0.3527    |        |
|                        |       | 3   | 1.0000    | 1.9499         | 0.2584    |        |
| Continued on next page |       |     |           |                |           |        |

Table S23: The basis info of molecule H<sub>2</sub>O.

| Model | Atom | $k$ | $n_{a,k}$ | $\alpha_{a,k}$ | $c_{a,k}$ |
|-------|------|-----|-----------|----------------|-----------|
| NLIS1 | O    | 4   | 1.0000    | 1.4845         | 0.0000    |
|       |      | 5   | 1.0000    | 1.2133         | 0.0000    |
|       |      | 1   | 2.0000    | 151.6262       | 0.4068    |
|       |      | 2   | 2.0000    | 34.3940        | 1.3158    |
|       |      | 3   | 2.0000    | 4.4745         | 0.4601    |
|       |      | 4   | 2.0000    | 1.1952         | 4.5183    |
|       |      | 5   | 2.0000    | 0.3960         | 2.0200    |
|       |      | 6   | 2.0000    | 0.1295         | 0.1087    |
|       | H    | 1   | 2.0000    | 13.3536        | 0.0130    |
|       |      | 2   | 2.0000    | 2.4263         | 0.2408    |
|       |      | 3   | 2.0000    | 0.7414         | 0.2864    |
|       |      | 4   | 2.0000    | 0.2329         | 0.0450    |
| NLIS2 | O    | 1   | 2.0000    | 433.3586       | 0.0684    |
|       |      | 2   | 2.0000    | 95.0906        | 0.5390    |
|       |      | 3   | 2.0000    | 30.4852        | 1.1243    |
|       |      | 4   | 2.0000    | 1.2643         | 1.4239    |
|       |      | 5   | 2.0000    | 1.2643         | 1.0292    |
|       |      | 6   | 1.0000    | 2.1794         | 4.6433    |
|       | H    | 1   | 2.0000    | 13.5046        | 0.0126    |
|       |      | 2   | 2.0000    | 2.4327         | 0.2381    |
|       |      | 3   | 2.0000    | 0.7298         | 0.2785    |
|       |      | 4   | 1.0000    | 1.4048         | 0.0567    |
| NLIS3 | O    | 1   | 2.0000    | 149.5745       | 0.4144    |
|       |      | 2   | 2.0000    | 34.1371        | 1.2971    |
|       |      | 3   | 2.0000    | 1.2748         | 0.9871    |
|       |      | 4   | 2.0000    | 1.2748         | 1.3488    |
|       |      | 5   | 1.0000    | 2.1989         | 3.6060    |
|       |      | 6   | 1.0000    | 2.1989         | 1.1738    |
|       | H    | 1   | 2.0000    | 2.2827         | 0.1723    |
|       |      | 2   | 2.0000    | 0.6965         | 0.2365    |
|       |      | 3   | 1.0000    | 1.3821         | 0.0554    |
|       |      | 4   | 1.0000    | 3.6933         | 0.1222    |
| NLIS4 | O    | 1   | 1.0000    | 17.6179        | 1.0087    |
|       |      |     |           |                |           |

Continued on next page

Table S23: The basis info of molecule H<sub>2</sub>O.

| Model | Atom | $k$ | $n_{a,k}$ | $\alpha_{a,k}$ | $c_{a,k}$ |
|-------|------|-----|-----------|----------------|-----------|
|       |      | 2   | 1.0000    | 17.6179        | 0.6343    |
|       |      | 3   | 1.0000    | 2.4347         | 3.5122    |
|       |      | 4   | 1.0000    | 2.4347         | 2.8430    |
|       |      | 5   | 1.0000    | 2.4347         | 0.1064    |
|       |      | 6   | 1.0000    | 2.4347         | 0.7383    |
|       | H    | 1   | 1.0000    | 1.2121         | 0.0451    |
|       |      | 2   | 1.0000    | 2.8241         | 0.0966    |
|       |      | 3   | 1.0000    | 2.8241         | 0.3191    |
|       |      | 4   | 1.0000    | 2.8241         | 0.1178    |
|       | MBIS | O   | 1         | 17.5482        | 1.6521    |
|       |      | 2   | 1.0000    | 2.4165         | 7.2060    |
|       | H    | 1   | 1.0000    | 2.6706         | 0.5710    |
| GMBIS | O    | 1   | 1.1720    | 20.5124        | 1.6188    |
|       |      | 2   | 1.0000    | 2.4218         | 7.2413    |
|       | H    | 1   | 1.0380    | 2.5633         | 0.5701    |



## S2.9 OH<sup>-</sup>

Table S24: The basis info of molecule OH<sup>-</sup>.

|       |      |     | $n_{a,k}$ | $\alpha_{a,k}$ | $c_{a,k}$ |
|-------|------|-----|-----------|----------------|-----------|
| Model | Atom | $k$ |           |                |           |
| LISA1 | O    | 1   | 2.0000    | 220.1000       | 0.1962    |
|       |      | 2   | 2.0000    | 65.6600        | 0.6486    |
|       |      | 3   | 2.0000    | 25.9800        | 0.9649    |
|       |      | 4   | 2.0000    | 1.6850         | 3.1076    |
|       |      | 5   | 2.0000    | 0.6860         | 2.5682    |
|       |      | 6   | 2.0000    | 0.2311         | 1.7648    |
|       | H    | 1   | 2.0000    | 5.6720         | 0.0518    |
|       |      | 2   | 2.0000    | 1.5050         | 0.4173    |
|       |      | 3   | 2.0000    | 0.5308         | 0.0000    |
|       |      | 4   | 2.0000    | 0.2204         | 0.2806    |
| LISA2 | O    | 1   | 2.0000    | 220.1000       | 0.1970    |
|       |      | 2   | 2.0000    | 65.6600        | 0.6443    |
|       |      | 3   | 2.0000    | 25.9800        | 0.9717    |
|       |      | 4   | 2.0000    | 1.6850         | 3.0335    |
|       |      | 5   | 2.0000    | 0.6860         | 2.7316    |
|       |      | 6   | 2.0000    | 0.2311         | 1.6084    |
|       | H    | 1   | 2.0000    | 5.6720         | 0.0577    |
|       |      | 2   | 2.0000    | 1.5050         | 0.3621    |
|       |      | 3   | 2.0000    | 0.5308         | 0.0924    |
|       |      | 4   | 2.0000    | 0.2204         | 0.0000    |
| LISA3 | O    | 1   | 2.0000    | 385.6603       | 0.0790    |
|       |      | 2   | 2.0000    | 143.8070       | 0.0426    |
|       |      | 3   | 2.0000    | 85.6482        | 0.5355    |
|       |      | 4   | 2.0000    | 33.0976        | 0.2019    |
|       |      | 5   | 2.0000    | 28.5587        | 0.9113    |
|       |      | 6   | 2.0000    | 2.8863         | 3.5834    |
|       |      | 7   | 2.0000    | 2.3338         | -9.4530   |
|       |      | 8   | 2.0000    | 1.9709         | 8.0688    |
|       |      | 9   | 2.0000    | 1.1642         | 1.9922    |

Continued on next page

Table S24: The basis info of molecule OH<sup>-</sup>.

| Model | Atom | <i>k</i> | <i>n<sub>a,k</sub></i> | <i>α<sub>a,k</sub></i> | <i>c<sub>a,k</sub></i> |
|-------|------|----------|------------------------|------------------------|------------------------|
|       |      |          |                        |                        |                        |
| LISA4 | H    | 10       | 2.0000                 | 0.4925                 | 2.0458                 |
|       |      | 11       | 2.0000                 | 0.3884                 | 0.3217                 |
|       |      | 12       | 2.0000                 | 0.1503                 | 0.9573                 |
|       |      | 1        | 2.0000                 | 7.1896                 | 0.0489                 |
|       |      | 2        | 2.0000                 | 1.6120                 | 0.3159                 |
|       |      | 3        | 2.0000                 | 0.5023                 | 0.3544                 |
|       |      | 4        | 2.0000                 | 0.2097                 | -0.3681                |
|       |      | 5        | 2.0000                 | 0.1683                 | 0.3624                 |
|       | O    | 1        | 2.0000                 | 385.6603               | 0.0801                 |
|       |      | 2        | 2.0000                 | 143.8070               | 0.0303                 |
|       |      | 3        | 2.0000                 | 85.6482                | 0.5641                 |
|       |      | 4        | 2.0000                 | 33.0976                | 0.0000                 |
|       |      | 5        | 2.0000                 | 28.5587                | 1.1163                 |
|       |      | 6        | 2.0000                 | 2.8863                 | 0.4108                 |
|       |      | 7        | 2.0000                 | 2.3338                 | 0.0000                 |
|       |      | 8        | 2.0000                 | 1.9709                 | 0.7511                 |
|       |      | 9        | 2.0000                 | 1.1642                 | 3.1718                 |
|       |      | 10       | 2.0000                 | 0.4925                 | 1.8028                 |
|       |      | 11       | 2.0000                 | 0.3884                 | 0.3810                 |
|       |      | 12       | 2.0000                 | 0.1503                 | 0.9804                 |
|       | H    | 1        | 2.0000                 | 7.1896                 | 0.0440                 |
|       |      | 2        | 2.0000                 | 1.6120                 | 0.3500                 |
|       |      | 3        | 2.0000                 | 0.5023                 | 0.2341                 |
|       |      | 4        | 2.0000                 | 0.2097                 | 0.0000                 |
|       |      | 5        | 2.0000                 | 0.1683                 | 0.0831                 |
| LISA5 | O    | 1        | 1.0000                 | 17.9859                | 1.5857                 |
|       |      | 2        | 1.0000                 | 2.8225                 | 5.1425                 |
|       |      | 3        | 1.0000                 | 1.4828                 | 2.5970                 |
|       |      | 4        | 1.0000                 | 1.2932                 | -0.0339                |
|       | H    | 1        | 1.0000                 | 4.2476                 | -0.3696                |
|       |      | 2        | 1.0000                 | 3.4951                 | 0.8090                 |
|       |      | 3        | 1.0000                 | 1.9499                 | 0.2643                 |
|       |      | 4        | 1.0000                 | 1.4845                 | -0.2312                |

Continued on next page

Table S24: The basis info of molecule OH<sup>-</sup>.

| Model | Atom | <i>k</i> | $n_{a,k}$ | $\alpha_{a,k}$ | $c_{a,k}$ |
|-------|------|----------|-----------|----------------|-----------|
| LISA6 | O    | 5        | 1.0000    | 1.2133         | 0.2362    |
|       |      | 1        | 1.0000    | 17.9859        | 1.5850    |
|       |      | 2        | 1.0000    | 2.8225         | 5.1557    |
|       |      | 3        | 1.0000    | 1.4828         | 2.5514    |
|       |      | 4        | 1.0000    | 1.2932         | 0.0000    |
|       | H    | 1        | 1.0000    | 4.2476         | 0.0000    |
|       |      | 2        | 1.0000    | 3.4951         | 0.2894    |
|       |      | 3        | 1.0000    | 1.9499         | 0.3582    |
|       |      | 4        | 1.0000    | 1.4845         | 0.0000    |
|       |      | 5        | 1.0000    | 1.2133         | 0.0602    |
| NLIS1 | O    | 1        | 2.0000    | 150.3495       | 0.4125    |
|       |      | 2        | 2.0000    | 34.1515        | 1.3179    |
|       |      | 3        | 2.0000    | 4.1532         | 0.4907    |
|       |      | 4        | 2.0000    | 1.2108         | 4.2813    |
|       |      | 5        | 2.0000    | 0.3692         | 2.2003    |
|       |      | 6        | 2.0000    | 0.1159         | 0.5892    |
|       | H    | 1        | 2.0000    | 13.0872        | 0.0139    |
|       |      | 2        | 2.0000    | 2.3750         | 0.2461    |
|       |      | 3        | 2.0000    | 0.6961         | 0.3526    |
|       |      | 4        | 2.0000    | 0.1769         | 0.0955    |
| NLIS2 | O    | 1        | 2.0000    | 330.8609       | 0.1108    |
|       |      | 2        | 2.0000    | 74.7193        | 0.7060    |
|       |      | 3        | 2.0000    | 25.5072        | 1.0067    |
|       |      | 4        | 2.0000    | 1.5450         | 3.1878    |
|       |      | 5        | 2.0000    | 0.6330         | 1.7848    |
|       |      | 6        | 1.0000    | 1.4293         | 2.4948    |
|       | H    | 1        | 2.0000    | 15.3732        | 0.0098    |
|       |      | 2        | 2.0000    | 2.6189         | 0.2055    |
|       |      | 3        | 2.0000    | 0.8074         | 0.2966    |
|       |      | 4        | 1.0000    | 1.4506         | 0.1972    |
| NLIS3 | O    | 1        | 2.0000    | 152.7157       | 0.4019    |
|       |      | 2        | 2.0000    | 34.7735        | 1.2962    |
|       |      | 3        | 2.0000    | 1.2743         | 0.7316    |

Continued on next page

Table S24: The basis info of molecule OH<sup>-</sup>.

| Model | Atom | $k$ | $n_{a,k}$ | $\alpha_{a,k}$ | $c_{a,k}$ |
|-------|------|-----|-----------|----------------|-----------|
|       |      |     |           |                |           |
| NLIS4 |      | 4   | 2.0000    | 1.2743         | 1.4575    |
|       |      | 5   | 1.0000    | 1.3793         | 2.0280    |
|       |      | 6   | 1.0000    | 2.4699         | 3.3754    |
|       | H    | 1   | 2.0000    | 3.4148         | 0.1551    |
|       |      | 2   | 2.0000    | 0.9511         | 0.3191    |
|       |      | 3   | 1.0000    | 1.5228         | 0.1566    |
|       |      | 4   | 1.0000    | 1.5228         | 0.0785    |
|       | O    | 1   | 1.0000    | 17.5946        | 1.1837    |
|       |      | 2   | 1.0000    | 17.5946        | 0.4637    |
|       |      | 3   | 1.0000    | 2.5151         | 3.6019    |
|       |      | 4   | 1.0000    | 1.2427         | 1.2941    |
|       |      | 5   | 1.0000    | 2.5151         | 1.6148    |
|       |      | 6   | 1.0000    | 2.5151         | 1.1367    |
| MBIS  | H    | 1   | 1.0000    | 1.4116         | 0.0945    |
|       |      | 2   | 1.0000    | 1.4116         | 0.0735    |
|       |      | 3   | 1.0000    | 2.7750         | 0.2850    |
|       |      | 4   | 1.0000    | 2.7750         | 0.2522    |
|       | O    | 1   | 1.0000    | 16.9652        | 1.7335    |
|       |      | 2   | 1.0000    | 2.2363         | 7.3739    |
|       | H    | 1   | 1.0000    | 1.4850         | 0.8924    |
| GMBIS | O    | 1   | 1.1720    | 19.8151        | 1.6908    |
|       |      | 2   | 1.0000    | 2.2479         | 7.4173    |
|       | H    | 1   | 1.0380    | 1.3616         | 0.8918    |

## S2.10 CS<sub>2</sub>

Table S25: The basis info of molecule CS<sub>2</sub>.

|       |      |     | $n_{a,k}$ | $\alpha_{a,k}$ | $c_{a,k}$ |
|-------|------|-----|-----------|----------------|-----------|
| Model | Atom | $k$ |           |                |           |
| LISA1 | C    | 1   | 2.0000    | 148.3000       | 0.1434    |
|       |      | 2   | 2.0000    | 42.1900        | 0.5599    |
|       |      | 3   | 2.0000    | 15.3300        | 1.1038    |
|       |      | 4   | 2.0000    | 6.1460         | 0.0006    |
|       |      | 5   | 2.0000    | 0.7846         | 2.9635    |
|       |      | 6   | 2.0000    | 0.2511         | 1.1564    |
|       | S    | 1   | 2.0000    | 528.7272       | 0.4850    |
|       |      | 2   | 2.0000    | 147.5558       | 1.1699    |
|       |      | 3   | 2.0000    | 17.6378        | 0.0000    |
|       |      | 4   | 2.0000    | 17.5077        | 0.0000    |
|       |      | 5   | 2.0000    | 15.1251        | 1.4826    |
|       |      | 6   | 2.0000    | 7.1494         | 6.0177    |
|       |      | 7   | 2.0000    | 0.5499         | 4.3316    |
|       |      | 8   | 2.0000    | 0.2713         | 2.4169    |
|       |      | 9   | 2.0000    | 0.1013         | 0.1327    |
| LISA2 | C    | 1   | 2.0000    | 148.3000       | 0.1434    |
|       |      | 2   | 2.0000    | 42.1900        | 0.5599    |
|       |      | 3   | 2.0000    | 15.3300        | 1.1038    |
|       |      | 4   | 2.0000    | 6.1460         | 0.0006    |
|       |      | 5   | 2.0000    | 0.7846         | 2.9635    |
|       |      | 6   | 2.0000    | 0.2511         | 1.1564    |
|       | S    | 1   | 2.0000    | 528.7272       | 0.4850    |
|       |      | 2   | 2.0000    | 147.5558       | 1.1699    |
|       |      | 3   | 2.0000    | 17.6378        | 0.0000    |
|       |      | 4   | 2.0000    | 17.5077        | 0.0000    |
|       |      | 5   | 2.0000    | 15.1251        | 1.4826    |
|       |      | 6   | 2.0000    | 7.1494         | 6.0177    |
|       |      | 7   | 2.0000    | 0.5499         | 4.3316    |
|       |      | 8   | 2.0000    | 0.2713         | 2.4169    |
|       |      | 9   | 2.0000    | 0.1013         | 0.1327    |

Continued on next page

Table S25: The basis info of molecule CS<sub>2</sub>.

| Model | Atom | $k$ | $n_{a,k}$ | $\alpha_{a,k}$ | $c_{a,k}$ |
|-------|------|-----|-----------|----------------|-----------|
| LISA3 | --   | --  | --        | --             | --        |
| LISA4 | C    | 1   | 2.0000    | 233.9861       | 0.0344    |
|       |      | 2   | 2.0000    | 191.1093       | 0.0535    |
|       |      | 3   | 2.0000    | 51.2230        | 0.2130    |
|       |      | 4   | 2.0000    | 42.7414        | 0.4238    |
|       |      | 5   | 2.0000    | 14.7443        | 1.0950    |
|       |      | 6   | 2.0000    | 0.8016         | 2.6051    |
|       |      | 7   | 2.0000    | 0.3994         | 0.8472    |
|       |      | 8   | 2.0000    | 0.3312         | 0.0000    |
|       |      | 9   | 2.0000    | 0.2759         | 0.0000    |
|       |      | 10  | 2.0000    | 0.2377         | 0.6141    |
|       |      | 11  | 2.0000    | 0.1169         | 0.0306    |
|       |      | 12  | 2.0000    | 0.0786         | 0.0000    |
|       |      | 13  | 2.0000    | 0.0696         | 0.0000    |
|       | S    | 1   | 2.0000    | 711.3601       | 0.3440    |
|       |      | 2   | 2.0000    | 162.3912       | 1.2819    |
|       |      | 3   | 2.0000    | 16.5222        | 1.3674    |
|       |      | 4   | 2.0000    | 7.1704         | 6.1622    |
|       |      | 5   | 2.0000    | 0.5595         | 4.0848    |
|       |      | 6   | 2.0000    | 0.3033         | 2.3091    |
|       |      | 7   | 2.0000    | 0.2619         | 0.0000    |
|       |      | 8   | 2.0000    | 0.1529         | 0.4883    |
|       |      | 9   | 2.0000    | 0.1258         | 0.0000    |
|       |      | 10  | 2.0000    | 0.1048         | 0.0000    |
|       |      | 11  | 2.0000    | 0.0707         | 0.0040    |
| LISA5 | --   | --  | --        | --             | --        |
| LISA6 | C    | 1   | 1.0000    | 13.0886        | 1.6443    |
|       |      | 2   | 1.0000    | 2.4356         | 0.0000    |
|       |      | 3   | 1.0000    | 1.9858         | 4.3633    |
|       |      | 4   | 1.0000    | 0.9936         | 0.0000    |
|       |      | 5   | 1.0000    | 0.8363         | 0.0000    |
|       | S    | 1   | 1.0000    | 42.2745        | 1.1975    |
|       |      | 2   | 1.0000    | 7.7340         | 7.5708    |

Continued on next page

Table S25: The basis info of molecule CS<sub>2</sub>.

| Model | Atom | $k$ | $n_{a,k}$ | $\alpha_{a,k}$ | $c_{a,k}$ |
|-------|------|-----|-----------|----------------|-----------|
| NLIS1 |      | 3   | 1.0000    | 2.0351         | 2.3446    |
|       |      | 4   | 1.0000    | 1.6193         | 4.8831    |
|       |      | 5   | 1.0000    | 0.8676         | 0.0000    |
|       | C    | 1   | 2.0000    | 187.8811       | 0.1050    |
|       |      | 2   | 2.0000    | 42.0786        | 0.6840    |
|       |      | 3   | 2.0000    | 13.9644        | 1.0500    |
|       |      | 4   | 2.0000    | 0.7113         | 1.4402    |
|       |      | 5   | 2.0000    | 0.7113         | 1.7914    |
|       |      | 6   | 2.0000    | 0.2294         | 0.8441    |
|       | S    | 1   | 2.0000    | 713.7267       | 0.3412    |
|       |      | 2   | 2.0000    | 162.8533       | 1.2856    |
|       |      | 3   | 2.0000    | 17.3250        | 1.1611    |
|       |      | 4   | 2.0000    | 7.2999         | 2.5491    |
|       |      | 5   | 2.0000    | 7.2999         | 2.2280    |
|       |      | 6   | 2.0000    | 7.2999         | 1.6064    |
|       |      | 7   | 2.0000    | 0.4925         | 2.0300    |
|       |      | 8   | 2.0000    | 0.4925         | 3.5477    |
|       |      | 9   | 2.0000    | 0.1890         | 1.2936    |
| NLIS2 | C    | 1   | 2.0000    | 226.2413       | 0.0756    |
|       |      | 2   | 2.0000    | 49.5984        | 0.5727    |
|       |      | 3   | 2.0000    | 15.7585        | 1.1314    |
|       |      | 4   | 2.0000    | 0.6829         | 1.1044    |
|       |      | 5   | 2.0000    | 0.6829         | 1.2437    |
|       |      | 6   | 1.0000    | 1.6813         | 1.8134    |
|       | S    | 1   | 2.0000    | 731.6134       | 0.3280    |
|       |      | 2   | 2.0000    | 166.4341       | 1.2791    |
|       |      | 3   | 2.0000    | 21.7915        | 0.7303    |
|       |      | 4   | 2.0000    | 7.7195         | 2.7182    |
|       |      | 5   | 2.0000    | 7.7195         | 2.3586    |
|       |      | 6   | 2.0000    | 7.7195         | 1.5797    |
|       |      | 7   | 2.0000    | 0.4468         | 1.7505    |
|       |      | 8   | 2.0000    | 0.4468         | 2.5220    |
|       |      | 9   | 1.0000    | 1.6030         | 2.7633    |

Continued on next page

Table S25: The basis info of molecule CS<sub>2</sub>.

| Model | Atom | $k$ | $n_{a,k}$ | $\alpha_{a,k}$ | $c_{a,k}$ |
|-------|------|-----|-----------|----------------|-----------|
|       |      |     |           |                |           |
| NLIS3 | C    | 1   | 2.0000    | 226.2413       | 0.0756    |
|       |      | 2   | 2.0000    | 49.5984        | 0.5727    |
|       |      | 3   | 2.0000    | 15.7585        | 1.1314    |
|       |      | 4   | 2.0000    | 0.6829         | 2.3481    |
|       |      | 5   | 1.0000    | 1.6813         | 1.1231    |
|       |      | 6   | 1.0000    | 1.6813         | 0.6904    |
|       | S    | 1   | 2.0000    | 731.6134       | 0.3280    |
|       |      | 2   | 2.0000    | 166.4341       | 1.2791    |
|       |      | 3   | 2.0000    | 21.7915        | 0.7303    |
|       |      | 4   | 2.0000    | 7.7195         | 2.8325    |
|       |      | 5   | 2.0000    | 7.7195         | 2.4358    |
|       |      | 6   | 2.0000    | 7.7195         | 1.3881    |
|       |      | 7   | 2.0000    | 0.4468         | 4.2725    |
|       |      | 8   | 1.0000    | 1.6030         | 2.4868    |
|       |      | 9   | 1.0000    | 1.6030         | 0.2765    |
| NLIS4 | C    | 1   | 1.0000    | 13.0446        | 0.9982    |
|       |      | 2   | 1.0000    | 13.0446        | 0.6552    |
|       |      | 3   | 1.0000    | 1.9614         | 1.8743    |
|       |      | 4   | 1.0000    | 1.9614         | 1.4096    |
|       |      | 5   | 1.0000    | 1.9614         | 0.3987    |
|       |      | 6   | 1.0000    | 1.9614         | 0.7075    |
|       | S    | 1   | 1.0000    | 42.4919        | 0.6557    |
|       |      | 2   | 1.0000    | 42.4919        | 0.5242    |
|       |      | 3   | 1.0000    | 7.8163         | 3.1693    |
|       |      | 4   | 1.0000    | 7.8163         | 2.7822    |
|       |      | 5   | 1.0000    | 7.8163         | 1.6167    |
|       |      | 6   | 1.0000    | 1.7574         | 3.8802    |
|       |      | 7   | 1.0000    | 1.7574         | 0.1228    |
|       |      | 8   | 1.0000    | 1.7574         | 2.3642    |
|       |      | 9   | 1.0000    | 1.7574         | 0.8627    |
| MBIS  | C    | 1   | 1.0000    | 13.0446        | 1.6534    |
|       |      | 2   | 1.0000    | 1.9614         | 4.3902    |
|       | S    | 1   | 1.0000    | 42.4919        | 1.1800    |

Continued on next page



Table S25: The basis info of molecule CS<sub>2</sub>.

| Model | Atom | $k$ | $n_{a,k}$ | $\alpha_{a,k}$ | $c_{a,k}$ |
|-------|------|-----|-----------|----------------|-----------|
|       |      |     |           |                |           |
| GMBIS |      | 2   | 1.0000    | 7.8163         | 7.5682    |
|       |      | 3   | 1.0000    | 1.7574         | 7.2299    |
|       | C    | 1   | 1.1380    | 14.1024        | 1.6308    |
|       |      | 2   | 1.0000    | 1.9709         | 4.3865    |
|       | S    | 1   | 1.0000    | 34.0031        | 1.8040    |
|       |      | 2   | 2.0000    | 8.8103         | 6.5731    |
|       |      | 3   | 1.0000    | 1.8004         | 7.6138    |
|       |      |     |           |                |           |

## S2.11 CCl<sub>4</sub>

Table S26: The basis info of molecule CCl<sub>4</sub>.

| Model | Atom | $k$ | $n_{a,k}$ | $\alpha_{a,k}$ | $c_{a,k}$ |
|-------|------|-----|-----------|----------------|-----------|
| LISA1 | C    | 1   | 2.0000    | 148.3000       | 0.1436    |
|       |      | 2   | 2.0000    | 42.1900        | 0.5550    |
|       |      | 3   | 2.0000    | 15.3300        | 1.1109    |
|       |      | 4   | 2.0000    | 6.1460         | 0.0000    |
|       |      | 5   | 2.0000    | 0.7846         | 2.8938    |
|       |      | 6   | 2.0000    | 0.2511         | 0.8483    |
|       | Cl   | 1   | 2.0000    | 622.3137       | 0.4570    |
|       |      | 2   | 2.0000    | 180.7931       | 1.0423    |
|       |      | 3   | 2.0000    | 98.9482        | 0.1670    |
|       |      | 4   | 2.0000    | 69.1275        | 0.0000    |
|       |      | 5   | 2.0000    | 20.2219        | 0.9027    |
|       |      | 6   | 2.0000    | 8.9831         | 6.4978    |
|       |      | 7   | 2.0000    | 0.6418         | 5.5218    |
|       |      | 8   | 2.0000    | 0.3052         | 2.2654    |
|       |      | 9   | 2.0000    | 0.1370         | 0.2580    |
| LISA2 | C    | 1   | 2.0000    | 148.3000       | 0.1436    |
|       |      | 2   | 2.0000    | 42.1900        | 0.5550    |
|       |      | 3   | 2.0000    | 15.3300        | 1.1109    |
|       |      | 4   | 2.0000    | 6.1460         | 0.0000    |
|       |      | 5   | 2.0000    | 0.7846         | 2.8938    |
|       |      | 6   | 2.0000    | 0.2511         | 0.8483    |
|       | Cl   | 1   | 2.0000    | 622.3137       | 0.4570    |
|       |      | 2   | 2.0000    | 180.7931       | 1.0423    |
|       |      | 3   | 2.0000    | 98.9482        | 0.1670    |
|       |      | 4   | 2.0000    | 69.1275        | 0.0000    |
|       |      | 5   | 2.0000    | 20.2219        | 0.9027    |
|       |      | 6   | 2.0000    | 8.9831         | 6.4978    |
|       |      | 7   | 2.0000    | 0.6418         | 5.5218    |
|       |      | 8   | 2.0000    | 0.3052         | 2.2654    |
|       |      | 9   | 2.0000    | 0.1370         | 0.2580    |

Continued on next page

Table S26: The basis info of molecule CCl<sub>4</sub>.

| Model | Atom | $k$ | $n_{a,k}$ | $\alpha_{a,k}$ | $c_{a,k}$ |
|-------|------|-----|-----------|----------------|-----------|
| LISA3 | --   | --  | --        | --             | --        |
| LISA4 | C    | 1   | 2.0000    | 233.9861       | 0.0331    |
|       |      | 2   | 2.0000    | 191.1093       | 0.0552    |
|       |      | 3   | 2.0000    | 51.2230        | 0.2062    |
|       |      | 4   | 2.0000    | 42.7414        | 0.4286    |
|       |      | 5   | 2.0000    | 14.7443        | 1.0963    |
|       |      | 6   | 2.0000    | 0.8016         | 2.5962    |
|       |      | 7   | 2.0000    | 0.3994         | 0.8164    |
|       |      | 8   | 2.0000    | 0.3312         | 0.0000    |
|       |      | 9   | 2.0000    | 0.2759         | 0.0000    |
|       |      | 10  | 2.0000    | 0.2377         | 0.0000    |
|       |      | 11  | 2.0000    | 0.1169         | 0.5785    |
|       |      | 12  | 2.0000    | 0.0786         | 0.0000    |
|       |      | 13  | 2.0000    | 0.0696         | 0.0000    |
|       | Cl   | 1   | 2.0000    | 833.6207       | 0.3255    |
|       |      | 2   | 2.0000    | 189.6607       | 1.2747    |
|       |      | 3   | 2.0000    | 23.4593        | 0.8598    |
|       |      | 4   | 2.0000    | 8.9937         | 6.6220    |
|       |      | 5   | 2.0000    | 0.7225         | 0.0000    |
|       |      | 6   | 2.0000    | 0.6118         | 6.1112    |
|       |      | 7   | 2.0000    | 0.3641         | 0.1607    |
|       |      | 8   | 2.0000    | 0.2698         | 1.0604    |
|       |      | 9   | 2.0000    | 0.2170         | 0.6079    |
|       |      | 10  | 2.0000    | 0.1261         | 0.0000    |
|       |      | 11  | 2.0000    | 0.0977         | 0.0249    |
| LISA5 | --   | --  | --        | --             | --        |
| LISA6 | C    | 1   | 1.0000    | 13.0886        | 1.6563    |
|       |      | 2   | 1.0000    | 2.4356         | 0.0000    |
|       |      | 3   | 1.0000    | 1.9858         | 4.0830    |
|       |      | 4   | 1.0000    | 0.9936         | 0.0000    |
|       |      | 5   | 1.0000    | 0.8363         | 0.0000    |
|       | Cl   | 1   | 1.0000    | 45.5731        | 1.1611    |
|       |      | 2   | 1.0000    | 8.5383         | 7.4146    |

Continued on next page

Table S26: The basis info of molecule CCl<sub>4</sub>.

| Model | Atom | $k$ | $n_{a,k}$ | $\alpha_{a,k}$ | $c_{a,k}$ |
|-------|------|-----|-----------|----------------|-----------|
| NLIS1 |      | 3   | 1.0000    | 2.0656         | 5.3572    |
|       |      | 4   | 1.0000    | 1.7037         | 3.1330    |
|       |      | 5   | 1.0000    | 1.0156         | 0.0000    |
|       | C    | 1   | 2.0000    | 185.5325       | 0.1070    |
|       |      | 2   | 2.0000    | 41.5480        | 0.6928    |
|       |      | 3   | 2.0000    | 13.7624        | 1.0468    |
|       |      | 4   | 2.0000    | 0.6792         | 1.3591    |
|       |      | 5   | 2.0000    | 0.6792         | 2.0176    |
|       |      | 6   | 2.0000    | 0.0938         | 0.5996    |
|       | Cl   | 1   | 2.0000    | 833.6614       | 0.3249    |
|       |      | 2   | 2.0000    | 189.7966       | 1.2757    |
|       |      | 3   | 2.0000    | 24.6873        | 0.7418    |
|       |      | 4   | 2.0000    | 9.1123         | 2.8227    |
|       |      | 5   | 2.0000    | 9.1123         | 2.3892    |
|       |      | 6   | 2.0000    | 9.1123         | 1.5246    |
|       |      | 7   | 2.0000    | 0.6005         | 2.7581    |
|       |      | 8   | 2.0000    | 0.6005         | 3.5928    |
|       |      | 9   | 2.0000    | 0.2417         | 1.6142    |
| NLIS2 | C    | 1   | 2.0000    | 199.2326       | 0.0944    |
|       |      | 2   | 2.0000    | 44.2867        | 0.6479    |
|       |      | 3   | 2.0000    | 14.4327        | 1.0849    |
|       |      | 4   | 2.0000    | 0.7090         | 1.3163    |
|       |      | 5   | 2.0000    | 0.7090         | 1.5736    |
|       |      | 6   | 1.0000    | 1.3001         | 0.9578    |
|       | Cl   | 1   | 2.0000    | 878.1608       | 0.2987    |
|       |      | 2   | 2.0000    | 198.9131       | 1.2548    |
|       |      | 3   | 2.0000    | 36.5260        | 0.4623    |
|       |      | 4   | 2.0000    | 9.5502         | 3.0187    |
|       |      | 5   | 2.0000    | 9.5502         | 2.5138    |
|       |      | 6   | 2.0000    | 9.5502         | 1.3605    |
|       |      | 7   | 2.0000    | 0.5481         | 2.2958    |
|       |      | 8   | 2.0000    | 0.5481         | 2.7750    |
|       |      | 9   | 1.0000    | 1.7019         | 3.1015    |

Continued on next page

Table S26: The basis info of molecule CCl<sub>4</sub>.

| Model | Atom | $k$ | $n_{a,k}$ | $\alpha_{a,k}$ | $c_{a,k}$ |
|-------|------|-----|-----------|----------------|-----------|
| NLIS3 | C    | 1   | 2.0000    | 199.3542       | 0.0943    |
|       |      | 2   | 2.0000    | 44.3107        | 0.6476    |
|       |      | 3   | 2.0000    | 14.4384        | 1.0852    |
|       |      | 4   | 2.0000    | 0.7094         | 2.8858    |
|       |      | 5   | 1.0000    | 1.3006         | 0.5723    |
|       |      | 6   | 1.0000    | 1.3006         | 0.3917    |
|       | Cl   | 1   | 2.0000    | 438.1667       | 0.2130    |
|       |      | 2   | 2.0000    | 155.6125       | 0.8614    |
|       |      | 3   | 2.0000    | 24.4414        | 0.5106    |
|       |      | 4   | 2.0000    | 9.4392         | 3.7313    |
|       |      | 5   | 2.0000    | 9.4392         | 3.0160    |
|       |      | 6   | 2.0000    | 0.5477         | 0.9012    |
|       |      | 7   | 2.0000    | 0.5477         | 4.1968    |
|       |      | 8   | 1.0000    | 1.6979         | 3.0653    |
|       |      | 9   | 1.0000    | 48.4404        | 0.5849    |
| NLIS4 | C    | 1   | 1.0000    | 12.8143        | 1.0126    |
|       |      | 2   | 1.0000    | 12.8143        | 0.6833    |
|       |      | 3   | 1.0000    | 1.8921         | 2.2325    |
|       |      | 4   | 1.0000    | 1.8921         | 0.5668    |
|       |      | 5   | 1.0000    | 1.8921         | 0.5200    |
|       |      | 6   | 1.0000    | 1.8921         | 0.8448    |
|       | Cl   | 1   | 1.0000    | 45.7557        | 1.1457    |
|       |      | 2   | 1.0000    | 8.5966         | 0.9403    |
|       |      | 3   | 1.0000    | 8.5966         | 2.9960    |
|       |      | 4   | 1.0000    | 8.5966         | 2.5503    |
|       |      | 5   | 1.0000    | 8.5966         | 0.9767    |
|       |      | 6   | 1.0000    | 1.9116         | 4.5001    |
|       |      | 7   | 1.0000    | 1.9116         | 0.0682    |
|       |      | 8   | 1.0000    | 1.9116         | 2.3851    |
|       |      | 9   | 1.0000    | 1.9116         | 1.4731    |
| MBIS  | C    | 1   | 1.0000    | 12.8143        | 1.6959    |
|       |      | 2   | 1.0000    | 1.8921         | 4.1642    |
|       | Cl   | 1   | 1.0000    | 45.7557        | 1.1457    |

Continued on next page

Table S26: The basis info of molecule CCl<sub>4</sub>.

| Model | Atom | $k$ | $n_{a,k}$ | $\alpha_{a,k}$ | $c_{a,k}$ |
|-------|------|-----|-----------|----------------|-----------|
|       |      |     |           |                |           |
| GMBIS |      | 2   | 1.0000    | 8.5966         | 7.4632    |
|       |      | 3   | 1.0000    | 1.9116         | 8.4265    |
|       |      |     |           |                |           |
|       | C    | 1   | 1.1380    | 13.8568        | 1.6668    |
|       |      | 2   | 1.0000    | 1.9162         | 4.1528    |
|       | Cl   | 1   | 1.1110    | 44.3630        | 1.7303    |
|       |      | 2   | 2.0000    | 10.7390        | 6.5100    |
|       |      | 3   | 1.0000    | 1.9525         | 8.8050    |

## S2.12 B<sub>8</sub>

Table S27: The basis info of molecule B<sub>8</sub>.

| Model | Atom | $k$ | $n_{a,k}$ | $\alpha_{a,k}$ | $c_{a,k}$ |
|-------|------|-----|-----------|----------------|-----------|
| LISA1 | B1   | 1   | 2.0000    | 98.2299        | 0.1467    |
|       |      | 2   | 2.0000    | 27.7169        | 0.6013    |
|       |      | 3   | 2.0000    | 9.7959         | 1.0725    |
|       |      | 4   | 2.0000    | 0.5004         | 2.6075    |
|       |      | 5   | 2.0000    | 0.1942         | 0.1609    |
|       |      | 6   | 2.0000    | 0.0618         | 0.0000    |
|       | B2   | 1   | 2.0000    | 98.2299        | 0.1477    |
|       |      | 2   | 2.0000    | 27.7169        | 0.6075    |
|       |      | 3   | 2.0000    | 9.7959         | 1.0708    |
|       |      | 4   | 2.0000    | 0.5004         | 2.4534    |
|       |      | 5   | 2.0000    | 0.1942         | 0.5492    |
|       |      | 6   | 2.0000    | 0.0618         | 0.0157    |
|       | B3   | 1   | 2.0000    | 98.2299        | 0.1471    |
|       |      | 2   | 2.0000    | 27.7169        | 0.6078    |
|       |      | 3   | 2.0000    | 9.7959         | 1.0675    |
|       |      | 4   | 2.0000    | 0.5004         | 2.4581    |
|       |      | 5   | 2.0000    | 0.1942         | 0.8078    |
|       |      | 6   | 2.0000    | 0.0618         | 0.0232    |
|       | B4   | 1   | 2.0000    | 98.2299        | 0.1470    |
|       |      | 2   | 2.0000    | 27.7169        | 0.6072    |
|       |      | 3   | 2.0000    | 9.7959         | 1.0675    |
|       |      | 4   | 2.0000    | 0.5004         | 2.4357    |
|       |      | 5   | 2.0000    | 0.1942         | 0.9537    |
|       |      | 6   | 2.0000    | 0.0618         | 0.0280    |
|       | B5   | 1   | 2.0000    | 98.2299        | 0.1475    |
|       |      | 2   | 2.0000    | 27.7169        | 0.6078    |
|       |      | 3   | 2.0000    | 9.7959         | 1.0694    |
|       |      | 4   | 2.0000    | 0.5004         | 2.4613    |
|       |      | 5   | 2.0000    | 0.1942         | 0.6288    |
|       |      | 6   | 2.0000    | 0.0618         | 0.0180    |

Continued on next page

Table S27: The basis info of molecule B<sub>8</sub>.

| Model | Atom | $k$ | $n_{a,k}$ | $\alpha_{a,k}$ | $c_{a,k}$ |
|-------|------|-----|-----------|----------------|-----------|
| LISA2 | B1   | 1   | 2.0000    | 98.2299        | 0.1467    |
|       |      | 2   | 2.0000    | 27.7169        | 0.6013    |
|       |      | 3   | 2.0000    | 9.7959         | 1.0725    |
|       |      | 4   | 2.0000    | 0.5004         | 2.6075    |
|       |      | 5   | 2.0000    | 0.1942         | 0.1609    |
|       |      | 6   | 2.0000    | 0.0618         | 0.0000    |
|       | B2   | 1   | 2.0000    | 98.2299        | 0.1477    |
|       |      | 2   | 2.0000    | 27.7169        | 0.6075    |
|       |      | 3   | 2.0000    | 9.7959         | 1.0708    |
|       |      | 4   | 2.0000    | 0.5004         | 2.4534    |
|       |      | 5   | 2.0000    | 0.1942         | 0.5492    |
|       |      | 6   | 2.0000    | 0.0618         | 0.0157    |
|       | B3   | 1   | 2.0000    | 98.2299        | 0.1471    |
|       |      | 2   | 2.0000    | 27.7169        | 0.6078    |
|       |      | 3   | 2.0000    | 9.7959         | 1.0675    |
|       |      | 4   | 2.0000    | 0.5004         | 2.4581    |
|       |      | 5   | 2.0000    | 0.1942         | 0.8078    |
|       |      | 6   | 2.0000    | 0.0618         | 0.0232    |
|       | B4   | 1   | 2.0000    | 98.2299        | 0.1470    |
|       |      | 2   | 2.0000    | 27.7169        | 0.6072    |
|       |      | 3   | 2.0000    | 9.7959         | 1.0675    |
|       |      | 4   | 2.0000    | 0.5004         | 2.4357    |
|       |      | 5   | 2.0000    | 0.1942         | 0.9537    |
|       |      | 6   | 2.0000    | 0.0618         | 0.0280    |
|       | B5   | 1   | 2.0000    | 98.2299        | 0.1475    |
|       |      | 2   | 2.0000    | 27.7169        | 0.6078    |
|       |      | 3   | 2.0000    | 9.7959         | 1.0694    |
|       |      | 4   | 2.0000    | 0.5004         | 2.4613    |
|       |      | 5   | 2.0000    | 0.1942         | 0.6288    |
|       |      | 6   | 2.0000    | 0.0618         | 0.0180    |
| LISA3 | --   | --  | --        | --             | --        |
| LISA4 | B1   | 1   | 2.0000    | 303.6041       | 0.0160    |
|       |      | 2   | 2.0000    | 148.4830       | 0.0000    |

Continued on next page



Table S27: The basis info of molecule B<sub>8</sub>.

| Model                  | Atom | $k$ | $n_{a,k}$ | $\alpha_{a,k}$ | $c_{a,k}$ |
|------------------------|------|-----|-----------|----------------|-----------|
|                        |      | 3   | 2.0000    | 130.1460       | 0.0353    |
|                        |      | 4   | 2.0000    | 65.3637        | 0.1144    |
|                        |      | 5   | 2.0000    | 32.6810        | 0.0000    |
|                        |      | 6   | 2.0000    | 29.0242        | 0.4694    |
|                        |      | 7   | 2.0000    | 21.7035        | 0.1381    |
|                        |      | 8   | 2.0000    | 9.5565         | 1.0584    |
|                        |      | 9   | 2.0000    | 0.5301         | 1.8405    |
|                        |      | 10  | 2.0000    | 0.3357         | 0.9674    |
|                        |      | 11  | 2.0000    | 0.2382         | 0.0000    |
|                        |      | 12  | 2.0000    | 0.1830         | 0.0000    |
|                        |      | 13  | 2.0000    | 0.1617         | 0.0000    |
|                        |      | 14  | 2.0000    | 0.0746         | 0.0000    |
|                        |      | 15  | 2.0000    | 0.0547         | 0.0000    |
|                        |      | 16  | 2.0000    | 0.0492         | 0.0000    |
|                        | B2   | 1   | 2.0000    | 303.6041       | 0.0170    |
|                        |      | 2   | 2.0000    | 148.4830       | 0.0000    |
|                        |      | 3   | 2.0000    | 130.1460       | 0.0296    |
|                        |      | 4   | 2.0000    | 65.3637        | 0.1332    |
|                        |      | 5   | 2.0000    | 32.6810        | 0.0000    |
|                        |      | 6   | 2.0000    | 29.0242        | 0.3957    |
|                        |      | 7   | 2.0000    | 21.7035        | 0.2271    |
|                        |      | 8   | 2.0000    | 9.5565         | 1.0256    |
|                        |      | 9   | 2.0000    | 0.5301         | 1.9374    |
|                        |      | 10  | 2.0000    | 0.3357         | 0.7437    |
|                        |      | 11  | 2.0000    | 0.2382         | 0.0000    |
|                        |      | 12  | 2.0000    | 0.1830         | 0.0000    |
|                        |      | 13  | 2.0000    | 0.1617         | 0.3093    |
|                        |      | 14  | 2.0000    | 0.0746         | 0.0140    |
|                        |      | 15  | 2.0000    | 0.0547         | 0.0000    |
|                        |      | 16  | 2.0000    | 0.0492         | 0.0000    |
|                        | B3   | 1   | 2.0000    | 303.6041       | 0.0165    |
|                        |      | 2   | 2.0000    | 148.4830       | 0.0000    |
|                        |      | 3   | 2.0000    | 130.1460       | 0.0330    |
| Continued on next page |      |     |           |                |           |

Table S27: The basis info of molecule B<sub>8</sub>.

| Model                  | Atom | $k$ | $n_{a,k}$ | $\alpha_{a,k}$ | $c_{a,k}$ |
|------------------------|------|-----|-----------|----------------|-----------|
|                        |      | 4   | 2.0000    | 65.3637        | 0.1229    |
|                        |      | 5   | 2.0000    | 32.6810        | 0.0000    |
|                        |      | 6   | 2.0000    | 29.0242        | 0.4370    |
|                        |      | 7   | 2.0000    | 21.7035        | 0.1801    |
|                        |      | 8   | 2.0000    | 9.5565         | 1.0415    |
|                        |      | 9   | 2.0000    | 0.5301         | 1.6955    |
|                        |      | 10  | 2.0000    | 0.3357         | 1.1809    |
|                        |      | 11  | 2.0000    | 0.2382         | 0.0000    |
|                        |      | 12  | 2.0000    | 0.1830         | 0.0000    |
|                        |      | 13  | 2.0000    | 0.1617         | 0.3665    |
|                        |      | 14  | 2.0000    | 0.0746         | 0.0271    |
|                        |      | 15  | 2.0000    | 0.0547         | 0.0053    |
|                        |      | 16  | 2.0000    | 0.0492         | 0.0000    |
|                        | B4   | 1   | 2.0000    | 303.6041       | 0.0161    |
|                        |      | 2   | 2.0000    | 148.4830       | 0.0000    |
|                        |      | 3   | 2.0000    | 130.1460       | 0.0354    |
|                        |      | 4   | 2.0000    | 65.3637        | 0.1158    |
|                        |      | 5   | 2.0000    | 32.6810        | 0.0000    |
|                        |      | 6   | 2.0000    | 29.0242        | 0.4650    |
|                        |      | 7   | 2.0000    | 21.7035        | 0.1487    |
|                        |      | 8   | 2.0000    | 9.5565         | 1.0521    |
|                        |      | 9   | 2.0000    | 0.5301         | 1.5606    |
|                        |      | 10  | 2.0000    | 0.3357         | 1.3888    |
|                        |      | 11  | 2.0000    | 0.2382         | 0.0000    |
|                        |      | 12  | 2.0000    | 0.1830         | 0.0000    |
|                        |      | 13  | 2.0000    | 0.1617         | 0.4116    |
|                        |      | 14  | 2.0000    | 0.0746         | 0.0276    |
|                        |      | 15  | 2.0000    | 0.0547         | 0.0120    |
|                        |      | 16  | 2.0000    | 0.0492         | 0.0000    |
|                        | B5   | 1   | 2.0000    | 303.6041       | 0.0169    |
|                        |      | 2   | 2.0000    | 148.4830       | 0.0000    |
|                        |      | 3   | 2.0000    | 130.1460       | 0.0305    |
|                        |      | 4   | 2.0000    | 65.3637        | 0.1303    |
| Continued on next page |      |     |           |                |           |

Table S27: The basis info of molecule B<sub>8</sub>.

| Model | Atom | $k$ | $n_{a,k}$ | $\alpha_{a,k}$ | $c_{a,k}$ |
|-------|------|-----|-----------|----------------|-----------|
|       |      | 5   | 2.0000    | 32.6810        | 0.0000    |
|       |      | 6   | 2.0000    | 29.0242        | 0.4076    |
|       |      | 7   | 2.0000    | 21.7035        | 0.2135    |
|       |      | 8   | 2.0000    | 9.5565         | 1.0303    |
|       |      | 9   | 2.0000    | 0.5301         | 1.8621    |
|       |      | 10  | 2.0000    | 0.3357         | 0.8894    |
|       |      | 11  | 2.0000    | 0.2382         | 0.0000    |
|       |      | 12  | 2.0000    | 0.1830         | 0.0000    |
|       |      | 13  | 2.0000    | 0.1617         | 0.3222    |
|       |      | 14  | 2.0000    | 0.0746         | 0.0212    |
|       |      | 15  | 2.0000    | 0.0547         | 0.0000    |
|       |      | 16  | 2.0000    | 0.0492         | 0.0000    |
| LISA5 | --   | --  | --        | --             | --        |
| LISA6 | B1   | 1   | 1.0000    | 10.5516        | 1.6802    |
|       |      | 2   | 1.0000    | 2.1001         | 0.0000    |
|       |      | 3   | 1.0000    | 1.8017         | 1.8385    |
|       |      | 4   | 1.0000    | 1.4928         | 1.4040    |
|       |      | 5   | 1.0000    | 0.8188         | 0.0000    |
|       |      | 6   | 1.0000    | 0.6970         | 0.0000    |
|       | B2   | 1   | 1.0000    | 10.5516        | 1.6605    |
|       |      | 2   | 1.0000    | 2.1001         | 0.0000    |
|       |      | 3   | 1.0000    | 1.8017         | 2.7628    |
|       |      | 4   | 1.0000    | 1.4928         | 0.3642    |
|       |      | 5   | 1.0000    | 0.8188         | 0.0000    |
|       |      | 6   | 1.0000    | 0.6970         | 0.0000    |
|       | B3   | 1   | 1.0000    | 10.5516        | 1.6672    |
|       |      | 2   | 1.0000    | 2.1001         | 0.0000    |
|       |      | 3   | 1.0000    | 1.8017         | 2.0700    |
|       |      | 4   | 1.0000    | 1.4928         | 1.3303    |
|       |      | 5   | 1.0000    | 0.8188         | 0.0000    |
|       |      | 6   | 1.0000    | 0.6970         | 0.0000    |
|       | B4   | 1   | 1.0000    | 10.5516        | 1.6725    |
|       |      | 2   | 1.0000    | 2.1001         | 0.0000    |

Continued on next page

Table S27: The basis info of molecule B<sub>8</sub>.

| Model                  | Atom  | $k$ | $n_{a,k}$ | $\alpha_{a,k}$ | $c_{a,k}$ |        |
|------------------------|-------|-----|-----------|----------------|-----------|--------|
| NLIS1                  |       | 3   | 1.0000    | 1.8017         | 1.6743    |        |
|                        |       | 4   | 1.0000    | 1.4928         | 1.8512    |        |
|                        |       | 5   | 1.0000    | 0.8188         | 0.0000    |        |
|                        |       | 6   | 1.0000    | 0.6970         | 0.0000    |        |
|                        | B5    | 1   | 1.0000    | 10.5516        | 1.6623    |        |
|                        |       | 2   | 1.0000    | 2.1001         | 0.0000    |        |
|                        |       | 3   | 1.0000    | 1.8017         | 2.5497    |        |
|                        |       | 4   | 1.0000    | 1.4928         | 0.6689    |        |
|                        |       | 5   | 1.0000    | 0.8188         | 0.0000    |        |
|                        |       | 6   | 1.0000    | 0.6970         | 0.0000    |        |
|                        | NLIS1 | B1  | 1         | 2.0000         | 130.8458  | 0.1007 |
|                        |       |     | 2         | 2.0000         | 29.0094   | 0.6747 |
|                        |       |     | 3         | 2.0000         | 9.3166    | 1.0705 |
|                        |       |     | 4         | 2.0000         | 0.4548    | 0.8374 |
|                        |       |     | 5         | 2.0000         | 0.4548    | 1.9335 |
|                        |       |     | 6         | 2.0000         | 0.0313    | 0.0161 |
|                        |       | B2  | 1         | 2.0000         | 134.3265  | 0.0968 |
|                        |       |     | 2         | 2.0000         | 29.7667   | 0.6595 |
| 3                      |       |     | 2.0000    | 9.5806         | 1.0813    |        |
| 4                      |       |     | 2.0000    | 0.4728         | 0.8523    |        |
| 5                      |       |     | 2.0000    | 0.4728         | 1.7700    |        |
| 6                      |       |     | 2.0000    | 0.1536         | 0.3755    |        |
| B3                     |       | 1   | 2.0000    | 131.8030       | 0.1000    |        |
|                        |       | 2   | 2.0000    | 29.2453        | 0.6712    |        |
|                        |       | 3   | 2.0000    | 9.4310         | 1.0713    |        |
|                        |       | 4   | 2.0000    | 0.4496         | 0.9306    |        |
|                        |       | 5   | 2.0000    | 0.4496         | 1.8439    |        |
|                        |       | 6   | 2.0000    | 0.1538         | 0.4883    |        |
| B4                     |       | 1   | 2.0000    | 130.5632       | 0.1016    |        |
|                        |       | 2   | 2.0000    | 28.9887        | 0.6771    |        |
|                        |       | 3   | 2.0000    | 9.3576         | 1.0663    |        |
|                        |       | 4   | 2.0000    | 0.4414         | 2.7992    |        |
|                        |       | 5   | 2.0000    | 0.1617         | 0.5739    |        |
| Continued on next page |       |     |           |                |           |        |

Table S27: The basis info of molecule B<sub>8</sub>.

| Model                  | Atom | $k$ | $n_{a,k}$ | $\alpha_{a,k}$ | $c_{a,k}$ |
|------------------------|------|-----|-----------|----------------|-----------|
| NLIS2                  | B5   | 6   | 2.0000    | 0.0521         | 0.0173    |
|                        |      | 1   | 2.0000    | 133.8175       | 0.0975    |
|                        |      | 2   | 2.0000    | 29.6592        | 0.6618    |
|                        |      | 3   | 2.0000    | 9.5463         | 1.0794    |
|                        |      | 4   | 2.0000    | 0.4663         | 0.8719    |
|                        |      | 5   | 2.0000    | 0.4663         | 1.7930    |
|                        |      | 6   | 2.0000    | 0.1566         | 0.4211    |
|                        | B1   | 1   | 2.0000    | 129.7095       | 0.1022    |
|                        |      | 2   | 2.0000    | 28.7813        | 0.6802    |
|                        |      | 3   | 2.0000    | 9.2609         | 1.0655    |
|                        |      | 4   | 2.0000    | 0.4507         | 1.1396    |
|                        |      | 5   | 2.0000    | 0.4507         | 1.6431    |
|                        |      | 6   | 1.0000    | 0.3472         | 0.0000    |
|                        | B2   | 1   | 2.0000    | 143.3705       | 0.0863    |
|                        |      | 2   | 2.0000    | 31.5827        | 0.6181    |
|                        |      | 3   | 2.0000    | 10.0436        | 1.1080    |
|                        |      | 4   | 2.0000    | 0.4598         | 0.9008    |
|                        |      | 5   | 2.0000    | 0.4598         | 1.3576    |
|                        |      | 6   | 1.0000    | 1.3939         | 0.7642    |
|                        | B3   | 1   | 2.0000    | 142.5177       | 0.0871    |
|                        |      | 2   | 2.0000    | 31.4047        | 0.6211    |
|                        |      | 3   | 2.0000    | 9.9872         | 1.1042    |
|                        |      | 4   | 2.0000    | 0.4307         | 0.9424    |
|                        |      | 5   | 2.0000    | 0.4307         | 1.4087    |
|                        |      | 6   | 1.0000    | 1.3687         | 0.9439    |
|                        | B4   | 1   | 2.0000    | 141.8609       | 0.0877    |
|                        |      | 2   | 2.0000    | 31.2720        | 0.6235    |
|                        |      | 3   | 2.0000    | 9.9510         | 1.1015    |
|                        |      | 4   | 2.0000    | 0.4162         | 0.9543    |
|                        |      | 5   | 2.0000    | 0.4162         | 1.4251    |
|                        |      | 6   | 1.0000    | 1.3583         | 1.0415    |
|                        | B5   | 1   | 2.0000    | 143.1316       | 0.0865    |
|                        |      | 2   | 2.0000    | 31.5321        | 0.6189    |
| Continued on next page |      |     |           |                |           |

Table S27: The basis info of molecule B<sub>8</sub>.

| Model | Atom | $k$ | $n_{a,k}$ | $\alpha_{a,k}$ | $c_{a,k}$ |
|-------|------|-----|-----------|----------------|-----------|
| NLIS3 |      | 3   | 2.0000    | 10.0265        | 1.1069    |
|       |      | 4   | 2.0000    | 0.4503         | 0.9163    |
|       |      | 5   | 2.0000    | 0.4503         | 1.3761    |
|       |      | 6   | 1.0000    | 1.3848         | 0.8213    |
|       | B1   | 1   | 2.0000    | 129.7095       | 0.1022    |
|       |      | 2   | 2.0000    | 28.7813        | 0.6802    |
|       |      | 3   | 2.0000    | 9.2609         | 1.0655    |
|       |      | 4   | 2.0000    | 0.4507         | 2.7827    |
|       |      | 5   | 1.0000    | 0.3473         | 0.0000    |
|       |      | 6   | 1.0000    | 0.3473         | 0.0000    |
|       | B2   | 1   | 2.0000    | 143.3705       | 0.0863    |
|       |      | 2   | 2.0000    | 31.5827        | 0.6181    |
|       |      | 3   | 2.0000    | 10.0436        | 1.1080    |
|       |      | 4   | 2.0000    | 0.4598         | 2.2585    |
|       |      | 5   | 1.0000    | 1.3939         | 0.4798    |
|       |      | 6   | 1.0000    | 1.3939         | 0.2844    |
|       | B3   | 1   | 2.0000    | 142.5178       | 0.0871    |
|       |      | 2   | 2.0000    | 31.4047        | 0.6211    |
|       |      | 3   | 2.0000    | 9.9872         | 1.1042    |
|       |      | 4   | 2.0000    | 0.4307         | 2.3511    |
|       |      | 5   | 1.0000    | 1.3687         | 0.5879    |
|       |      | 6   | 1.0000    | 1.3687         | 0.3559    |
|       | B4   | 1   | 2.0000    | 141.8610       | 0.0877    |
|       |      | 2   | 2.0000    | 31.2720        | 0.6235    |
|       |      | 3   | 2.0000    | 9.9510         | 1.1015    |
|       |      | 4   | 2.0000    | 0.4162         | 2.3794    |
|       |      | 5   | 1.0000    | 1.3583         | 0.6446    |
|       |      | 6   | 1.0000    | 1.3583         | 0.3970    |
|       | B5   | 1   | 2.0000    | 143.1317       | 0.0865    |
|       |      | 2   | 2.0000    | 31.5321        | 0.6189    |
|       |      | 3   | 2.0000    | 10.0265        | 1.1069    |
|       |      | 4   | 2.0000    | 0.4503         | 2.2924    |
|       |      | 5   | 1.0000    | 1.3848         | 0.5144    |

Continued on next page

Table S27: The basis info of molecule B<sub>8</sub>.

| Model | Atom | $k$ | $n_{a,k}$ | $\alpha_{a,k}$ | $c_{a,k}$ |
|-------|------|-----|-----------|----------------|-----------|
| NLIS4 | B1   | 6   | 1.0000    | 1.3848         | 0.3069    |
|       |      | 1   | 1.0000    | 10.5590        | 1.0427    |
|       |      | 2   | 1.0000    | 10.5590        | 0.6445    |
|       |      | 3   | 1.0000    | 1.6631         | 0.8299    |
|       |      | 4   | 1.0000    | 1.6631         | 0.6042    |
|       |      | 5   | 1.0000    | 1.6631         | 1.1688    |
|       | B2   | 6   | 1.0000    | 1.6631         | 0.5976    |
|       |      | 1   | 1.0000    | 10.6892        | 1.0333    |
|       |      | 2   | 1.0000    | 10.6892        | 0.6333    |
|       |      | 3   | 1.0000    | 1.7255         | 1.2268    |
|       |      | 4   | 1.0000    | 1.7255         | 1.2995    |
|       |      | 5   | 1.0000    | 0.3726         | 0.0005    |
|       | B3   | 6   | 1.0000    | 1.7255         | 0.6226    |
|       |      | 1   | 1.0000    | 10.6743        | 1.0359    |
|       |      | 2   | 1.0000    | 10.6743        | 0.6332    |
|       |      | 3   | 1.0000    | 1.6653         | 1.1407    |
|       |      | 4   | 1.0000    | 1.6653         | 1.2028    |
|       |      | 5   | 1.0000    | 1.6653         | 0.4775    |
|       | B4   | 6   | 1.0000    | 1.6653         | 0.5770    |
|       |      | 1   | 1.0000    | 10.6617        | 1.0379    |
|       |      | 2   | 1.0000    | 10.6617        | 0.6338    |
|       |      | 3   | 1.0000    | 1.6359         | 1.1920    |
|       |      | 4   | 1.0000    | 1.6359         | 1.2612    |
|       |      | 5   | 1.0000    | 1.6359         | 0.4521    |
|       | B5   | 6   | 1.0000    | 1.6359         | 0.6057    |
|       |      | 1   | 1.0000    | 10.6852        | 1.0341    |
|       |      | 2   | 1.0000    | 10.6852        | 0.6331    |
|       |      | 3   | 1.0000    | 1.7053         | 1.2618    |
|       |      | 4   | 1.0000    | 1.7053         | 1.3324    |
|       |      | 5   | 1.0000    | 0.3760         | 0.0003    |
| MBIS  | B1   | 6   | 1.0000    | 1.7053         | 0.6386    |
|       |      | 1   | 1.0000    | 10.5588        | 1.6872    |
|       |      | 2   | 1.0000    | 1.6631         | 3.1999    |

Continued on next page

Table S27: The basis info of molecule B<sub>8</sub>.

|       |      |     | $n_{a,k}$ | $\alpha_{a,k}$ | $c_{a,k}$ |
|-------|------|-----|-----------|----------------|-----------|
| Model | Atom | $k$ |           |                |           |
| GMBIS | B2   | 1   | 1.0000    | 10.6887        | 1.6667    |
|       |      | 2   | 1.0000    | 1.7252         | 3.1490    |
|       | B3   | 1   | 1.0000    | 10.6736        | 1.6693    |
|       |      | 2   | 1.0000    | 1.6649         | 3.3980    |
|       | B4   | 1   | 1.0000    | 10.6608        | 1.6719    |
|       |      | 2   | 1.0000    | 1.6355         | 3.5112    |
|       | B5   | 1   | 1.0000    | 10.6846        | 1.6673    |
|       |      | 2   | 1.0000    | 1.7050         | 3.2328    |
|       | B1   | 1   | 1.0690    | 10.8037        | 1.6735    |
|       |      | 2   | 1.0000    | 1.6705         | 3.2088    |
|       | B2   | 1   | 1.0690    | 10.9403        | 1.6543    |
|       |      | 2   | 1.0000    | 1.7297         | 3.1619    |
|       | B3   | 1   | 1.0690    | 10.9216        | 1.6572    |
|       |      | 2   | 1.0000    | 1.6688         | 3.4108    |
|       | B4   | 1   | 1.0690    | 10.9065        | 1.6599    |
|       |      | 2   | 1.0000    | 1.6391         | 3.5243    |
|       | B5   | 1   | 1.0690    | 10.9351        | 1.6550    |
|       |      | 2   | 1.0000    | 1.7093         | 3.2457    |



## S2.13 B<sub>8</sub> triplet

Table S28: The basis info of molecule B<sub>8</sub> triplet.

| Model | Atom | $k$ | $n_{a,k}$ | $\alpha_{a,k}$ | $c_{a,k}$ |
|-------|------|-----|-----------|----------------|-----------|
| LISA1 | B1   | 1   | 2.0000    | 98.2299        | 0.1468    |
|       |      | 2   | 2.0000    | 27.7169        | 0.6010    |
|       |      | 3   | 2.0000    | 9.7959         | 1.0731    |
|       |      | 4   | 2.0000    | 0.5004         | 2.5986    |
|       |      | 5   | 2.0000    | 0.1942         | 0.1938    |
|       |      | 6   | 2.0000    | 0.0618         | 0.0000    |
|       | B2   | 1   | 2.0000    | 98.2299        | 0.1473    |
|       |      | 2   | 2.0000    | 27.7169        | 0.6076    |
|       |      | 3   | 2.0000    | 9.7959         | 1.0684    |
|       |      | 4   | 2.0000    | 0.5004         | 2.4556    |
|       |      | 5   | 2.0000    | 0.1942         | 0.7570    |
|       |      | 6   | 2.0000    | 0.0618         | 0.0199    |
|       | B3   | 1   | 2.0000    | 98.2299        | 0.1473    |
|       |      | 2   | 2.0000    | 27.7169        | 0.6077    |
|       |      | 3   | 2.0000    | 9.7959         | 1.0684    |
|       |      | 4   | 2.0000    | 0.5004         | 2.4563    |
|       |      | 5   | 2.0000    | 0.1942         | 0.7555    |
|       |      | 6   | 2.0000    | 0.0618         | 0.0198    |
|       | B4   | 1   | 2.0000    | 98.2299        | 0.1472    |
|       |      | 2   | 2.0000    | 27.7169        | 0.6077    |
|       |      | 3   | 2.0000    | 9.7959         | 1.0684    |
|       |      | 4   | 2.0000    | 0.5004         | 2.4564    |
|       |      | 5   | 2.0000    | 0.1942         | 0.7556    |
|       |      | 6   | 2.0000    | 0.0618         | 0.0200    |
|       | B5   | 1   | 2.0000    | 98.2299        | 0.1473    |
|       |      | 2   | 2.0000    | 27.7169        | 0.6076    |
|       |      | 3   | 2.0000    | 9.7959         | 1.0684    |
|       |      | 4   | 2.0000    | 0.5004         | 2.4559    |
|       |      | 5   | 2.0000    | 0.1942         | 0.7564    |
|       |      | 6   | 2.0000    | 0.0618         | 0.0198    |

Continued on next page

Table S28: The basis info of molecule B<sub>8</sub> triplet.

| Model | Atom | $k$ | $n_{a,k}$ | $\alpha_{a,k}$ | $c_{a,k}$ |
|-------|------|-----|-----------|----------------|-----------|
| LISA2 | B1   | 1   | 2.0000    | 98.2299        | 0.1468    |
|       |      | 2   | 2.0000    | 27.7169        | 0.6010    |
|       |      | 3   | 2.0000    | 9.7959         | 1.0731    |
|       |      | 4   | 2.0000    | 0.5004         | 2.5986    |
|       |      | 5   | 2.0000    | 0.1942         | 0.1938    |
|       |      | 6   | 2.0000    | 0.0618         | 0.0000    |
|       | B2   | 1   | 2.0000    | 98.2299        | 0.1473    |
|       |      | 2   | 2.0000    | 27.7169        | 0.6076    |
|       |      | 3   | 2.0000    | 9.7959         | 1.0684    |
|       |      | 4   | 2.0000    | 0.5004         | 2.4556    |
|       |      | 5   | 2.0000    | 0.1942         | 0.7570    |
|       |      | 6   | 2.0000    | 0.0618         | 0.0199    |
|       | B3   | 1   | 2.0000    | 98.2299        | 0.1473    |
|       |      | 2   | 2.0000    | 27.7169        | 0.6077    |
|       |      | 3   | 2.0000    | 9.7959         | 1.0684    |
|       |      | 4   | 2.0000    | 0.5004         | 2.4563    |
|       |      | 5   | 2.0000    | 0.1942         | 0.7555    |
|       |      | 6   | 2.0000    | 0.0618         | 0.0198    |
|       | B4   | 1   | 2.0000    | 98.2299        | 0.1472    |
|       |      | 2   | 2.0000    | 27.7169        | 0.6077    |
|       |      | 3   | 2.0000    | 9.7959         | 1.0684    |
|       |      | 4   | 2.0000    | 0.5004         | 2.4564    |
|       |      | 5   | 2.0000    | 0.1942         | 0.7556    |
|       |      | 6   | 2.0000    | 0.0618         | 0.0200    |
|       | B5   | 1   | 2.0000    | 98.2299        | 0.1473    |
|       |      | 2   | 2.0000    | 27.7169        | 0.6076    |
|       |      | 3   | 2.0000    | 9.7959         | 1.0684    |
|       |      | 4   | 2.0000    | 0.5004         | 2.4559    |
|       |      | 5   | 2.0000    | 0.1942         | 0.7564    |
|       |      | 6   | 2.0000    | 0.0618         | 0.0198    |
| LISA3 | --   | --  | --        | --             | --        |
| LISA4 | B1   | 1   | 2.0000    | 303.6041       | 0.0159    |
|       |      | 2   | 2.0000    | 148.4830       | 0.0000    |

Continued on next page

Table S28: The basis info of molecule B<sub>8</sub> triplet.

| Model                  | Atom | $k$ | $n_{a,k}$ | $\alpha_{a,k}$ | $c_{a,k}$ |
|------------------------|------|-----|-----------|----------------|-----------|
|                        |      | 3   | 2.0000    | 130.1460       | 0.0361    |
|                        |      | 4   | 2.0000    | 65.3637        | 0.1121    |
|                        |      | 5   | 2.0000    | 32.6810        | 0.0000    |
|                        |      | 6   | 2.0000    | 29.0242        | 0.4786    |
|                        |      | 7   | 2.0000    | 21.7035        | 0.1282    |
|                        |      | 8   | 2.0000    | 9.5565         | 1.0615    |
|                        |      | 9   | 2.0000    | 0.5301         | 1.8108    |
|                        |      | 10  | 2.0000    | 0.3357         | 1.0139    |
|                        |      | 11  | 2.0000    | 0.2382         | 0.0000    |
|                        |      | 12  | 2.0000    | 0.1830         | 0.0000    |
|                        |      | 13  | 2.0000    | 0.1617         | 0.0000    |
|                        |      | 14  | 2.0000    | 0.0746         | 0.0000    |
|                        |      | 15  | 2.0000    | 0.0547         | 0.0000    |
|                        |      | 16  | 2.0000    | 0.0492         | 0.0000    |
|                        | B2   | 1   | 2.0000    | 303.6041       | 0.0165    |
|                        |      | 2   | 2.0000    | 148.4830       | 0.0000    |
|                        |      | 3   | 2.0000    | 130.1460       | 0.0327    |
|                        |      | 4   | 2.0000    | 65.3637        | 0.1237    |
|                        |      | 5   | 2.0000    | 32.6810        | 0.0000    |
|                        |      | 6   | 2.0000    | 29.0242        | 0.4335    |
|                        |      | 7   | 2.0000    | 21.7035        | 0.1843    |
|                        |      | 8   | 2.0000    | 9.5565         | 1.0400    |
|                        |      | 9   | 2.0000    | 0.5301         | 1.7320    |
|                        |      | 10  | 2.0000    | 0.3357         | 1.1108    |
|                        |      | 11  | 2.0000    | 0.2382         | 0.0000    |
|                        |      | 12  | 2.0000    | 0.1830         | 0.0000    |
|                        |      | 13  | 2.0000    | 0.1617         | 0.3448    |
|                        |      | 14  | 2.0000    | 0.0746         | 0.0311    |
|                        |      | 15  | 2.0000    | 0.0547         | 0.0000    |
|                        |      | 16  | 2.0000    | 0.0492         | 0.0000    |
|                        | B3   | 1   | 2.0000    | 303.6041       | 0.0165    |
|                        |      | 2   | 2.0000    | 148.4830       | 0.0000    |
|                        |      | 3   | 2.0000    | 130.1460       | 0.0327    |
| Continued on next page |      |     |           |                |           |

Table S28: The basis info of molecule B<sub>8</sub> triplet.

| Model                  | Atom | $k$ | $n_{a,k}$ | $\alpha_{a,k}$ | $c_{a,k}$ |
|------------------------|------|-----|-----------|----------------|-----------|
|                        |      | 4   | 2.0000    | 65.3637        | 0.1238    |
|                        |      | 5   | 2.0000    | 32.6810        | 0.0000    |
|                        |      | 6   | 2.0000    | 29.0242        | 0.4332    |
|                        |      | 7   | 2.0000    | 21.7035        | 0.1847    |
|                        |      | 8   | 2.0000    | 9.5565         | 1.0399    |
|                        |      | 9   | 2.0000    | 0.5301         | 1.7327    |
|                        |      | 10  | 2.0000    | 0.3357         | 1.1103    |
|                        |      | 11  | 2.0000    | 0.2382         | 0.0000    |
|                        |      | 12  | 2.0000    | 0.1830         | 0.0000    |
|                        |      | 13  | 2.0000    | 0.1617         | 0.3438    |
|                        |      | 14  | 2.0000    | 0.0746         | 0.0310    |
|                        |      | 15  | 2.0000    | 0.0547         | 0.0000    |
|                        |      | 16  | 2.0000    | 0.0492         | 0.0000    |
|                        | B4   | 1   | 2.0000    | 303.6041       | 0.0165    |
|                        |      | 2   | 2.0000    | 148.4830       | 0.0000    |
|                        |      | 3   | 2.0000    | 130.1460       | 0.0327    |
|                        |      | 4   | 2.0000    | 65.3637        | 0.1238    |
|                        |      | 5   | 2.0000    | 32.6810        | 0.0000    |
|                        |      | 6   | 2.0000    | 29.0242        | 0.4332    |
|                        |      | 7   | 2.0000    | 21.7035        | 0.1847    |
|                        |      | 8   | 2.0000    | 9.5565         | 1.0399    |
|                        |      | 9   | 2.0000    | 0.5301         | 1.7324    |
|                        |      | 10  | 2.0000    | 0.3357         | 1.1109    |
|                        |      | 11  | 2.0000    | 0.2382         | 0.0000    |
|                        |      | 12  | 2.0000    | 0.1830         | 0.0000    |
|                        |      | 13  | 2.0000    | 0.1617         | 0.3435    |
|                        |      | 14  | 2.0000    | 0.0746         | 0.0312    |
|                        |      | 15  | 2.0000    | 0.0547         | 0.0000    |
|                        |      | 16  | 2.0000    | 0.0492         | 0.0000    |
|                        | B5   | 1   | 2.0000    | 303.6041       | 0.0165    |
|                        |      | 2   | 2.0000    | 148.4830       | 0.0000    |
|                        |      | 3   | 2.0000    | 130.1460       | 0.0327    |
|                        |      | 4   | 2.0000    | 65.3637        | 0.1237    |
| Continued on next page |      |     |           |                |           |

Table S28: The basis info of molecule B<sub>8</sub> triplet.

| Model | Atom | $k$ | $n_{a,k}$ | $\alpha_{a,k}$ | $c_{a,k}$ |
|-------|------|-----|-----------|----------------|-----------|
|       |      | 5   | 2.0000    | 32.6810        | 0.0000    |
|       |      | 6   | 2.0000    | 29.0242        | 0.4335    |
|       |      | 7   | 2.0000    | 21.7035        | 0.1843    |
|       |      | 8   | 2.0000    | 9.5565         | 1.0400    |
|       |      | 9   | 2.0000    | 0.5301         | 1.7319    |
|       |      | 10  | 2.0000    | 0.3357         | 1.1112    |
|       |      | 11  | 2.0000    | 0.2382         | 0.0000    |
|       |      | 12  | 2.0000    | 0.1830         | 0.0000    |
|       |      | 13  | 2.0000    | 0.1617         | 0.3442    |
|       |      | 14  | 2.0000    | 0.0746         | 0.0310    |
|       |      | 15  | 2.0000    | 0.0547         | 0.0000    |
|       |      | 16  | 2.0000    | 0.0492         | 0.0000    |
| LISA5 | --   | --  | --        | --             | --        |
| LISA6 | B1   | 1   | 1.0000    | 10.5516        | 1.6810    |
|       |      | 2   | 1.0000    | 2.1001         | 0.0000    |
|       |      | 3   | 1.0000    | 1.8017         | 1.7753    |
|       |      | 4   | 1.0000    | 1.4928         | 1.4907    |
|       |      | 5   | 1.0000    | 0.8188         | 0.0000    |
|       |      | 6   | 1.0000    | 0.6970         | 0.0000    |
|       | B2   | 1   | 1.0000    | 10.5516        | 1.6653    |
|       |      | 2   | 1.0000    | 2.1001         | 0.0000    |
|       |      | 3   | 1.0000    | 1.8017         | 2.2333    |
|       |      | 4   | 1.0000    | 1.4928         | 1.1085    |
|       |      | 5   | 1.0000    | 0.8188         | 0.0000    |
|       |      | 6   | 1.0000    | 0.6970         | 0.0000    |
|       | B3   | 1   | 1.0000    | 10.5516        | 1.6654    |
|       |      | 2   | 1.0000    | 2.1001         | 0.0000    |
|       |      | 3   | 1.0000    | 1.8017         | 2.2305    |
|       |      | 4   | 1.0000    | 1.4928         | 1.1120    |
|       |      | 5   | 1.0000    | 0.8188         | 0.0000    |
|       |      | 6   | 1.0000    | 0.6970         | 0.0000    |
|       | B4   | 1   | 1.0000    | 10.5516        | 1.6655    |
|       |      | 2   | 1.0000    | 2.1001         | 0.0000    |

Continued on next page

Table S28: The basis info of molecule B<sub>8</sub> triplet.

|                        |       |        | $n_{a,k}$ | $\alpha_{a,k}$ | $c_{a,k}$ |        |
|------------------------|-------|--------|-----------|----------------|-----------|--------|
| Model                  | Atom  | $k$    |           |                |           |        |
|                        |       | 3      | 1.0000    | 1.8017         | 2.2245    |        |
|                        |       | 4      | 1.0000    | 1.4928         | 1.1192    |        |
|                        |       | 5      | 1.0000    | 0.8188         | 0.0000    |        |
|                        |       | 6      | 1.0000    | 0.6970         | 0.0000    |        |
|                        | B5    | 1      | 1.0000    | 10.5516        | 1.6653    |        |
|                        |       | 2      | 1.0000    | 2.1001         | 0.0000    |        |
|                        |       | 3      | 1.0000    | 1.8017         | 2.2317    |        |
|                        |       | 4      | 1.0000    | 1.4928         | 1.1105    |        |
|                        |       | 5      | 1.0000    | 0.8188         | 0.0000    |        |
|                        |       | 6      | 1.0000    | 0.6970         | 0.0000    |        |
|                        | NLIS1 | B1     | 1         | 2.0000         | 130.1658  | 0.1016 |
|                        |       |        | 2         | 2.0000         | 28.8740   | 0.6779 |
|                        |       |        | 3         | 2.0000         | 9.2846    | 1.0675 |
|                        |       |        | 4         | 2.0000         | 0.4525    | 0.8423 |
|                        |       |        | 5         | 2.0000         | 0.4525    | 1.9421 |
|                        |       |        | 6         | 2.0000         | 0.0313    | 0.0265 |
|                        |       | B2     | 1         | 2.0000         | 132.0783  | 0.0996 |
|                        |       |        | 2         | 2.0000         | 29.3038   | 0.6699 |
| 3                      |       |        | 2.0000    | 9.4499         | 1.0723    |        |
| 4                      |       |        | 2.0000    | 0.4541         | 0.8974    |        |
| 5                      |       |        | 2.0000    | 0.4541         | 1.8407    |        |
| 6                      |       |        | 2.0000    | 0.1551         | 0.4691    |        |
| B3                     |       | 1      | 2.0000    | 132.0885       | 0.0996    |        |
|                        |       | 2      | 2.0000    | 29.3058        | 0.6699    |        |
|                        |       | 3      | 2.0000    | 9.4503         | 1.0724    |        |
|                        |       | 4      | 2.0000    | 0.4541         | 0.8975    |        |
|                        |       | 5      | 2.0000    | 0.4541         | 1.8413    |        |
|                        |       | 6      | 2.0000    | 0.1550         | 0.4679    |        |
| B4                     | 1     | 2.0000 | 132.0841  | 0.0996         |           |        |
|                        | 2     | 2.0000 | 29.3049   | 0.6699         |           |        |
|                        | 3     | 2.0000 | 9.4501    | 1.0723         |           |        |
|                        | 4     | 2.0000 | 0.4540    | 0.8983         |           |        |
|                        | 5     | 2.0000 | 0.4540    | 1.8410         |           |        |
| Continued on next page |       |        |           |                |           |        |

Table S28: The basis info of molecule B<sub>8</sub> triplet.

| Model | Atom | $k$    | $n_{a,k}$ | $\alpha_{a,k}$ | $c_{a,k}$ |
|-------|------|--------|-----------|----------------|-----------|
| NLIS2 | B5   | 6      | 2.0000    | 0.1549         | 0.4674    |
|       |      | 1      | 2.0000    | 132.0757       | 0.0996    |
|       |      | 2      | 2.0000    | 29.3033        | 0.6699    |
|       |      | 3      | 2.0000    | 9.4497         | 1.0723    |
|       |      | 4      | 2.0000    | 0.4541         | 0.8970    |
|       |      | 5      | 2.0000    | 0.4541         | 1.8417    |
|       |      | 6      | 2.0000    | 0.1550         | 0.4684    |
|       | B1   | 1      | 2.0000    | 128.9698       | 0.1033    |
|       |      | 2      | 2.0000    | 28.6335        | 0.6838    |
|       |      | 3      | 2.0000    | 9.2256         | 1.0621    |
|       |      | 4      | 2.0000    | 0.4481         | 1.1461    |
|       |      | 5      | 2.0000    | 0.4481         | 1.6511    |
|       |      | 6      | 1.0000    | 0.3222         | 0.0000    |
|       |      | B2     | 1         | 2.0000         | 142.8877  |
| 2     |      |        | 2.0000    | 31.4808        | 0.6196    |
| 3     |      |        | 2.0000    | 10.0095        | 1.1053    |
| 4     |      |        | 2.0000    | 0.4354         | 0.9276    |
| 5     |      |        | 2.0000    | 0.4354         | 1.3892    |
| 6     |      |        | 1.0000    | 1.3828         | 0.9225    |
| B3    |      | 1      | 2.0000    | 142.8738       | 0.0867    |
|       |      | 2      | 2.0000    | 31.4779        | 0.6196    |
|       |      | 3      | 2.0000    | 10.0087        | 1.1053    |
|       |      | 4      | 2.0000    | 0.4355         | 0.9282    |
|       |      | 5      | 2.0000    | 0.4355         | 1.3901    |
|       | 6    | 1.0000 | 1.3827    | 0.9203         |           |
| B4    | 1    | 2.0000 | 142.8550  | 0.0867         |           |
|       | 2    | 2.0000 | 31.4742   | 0.6197         |           |
|       | 3    | 2.0000 | 10.0078   | 1.1053         |           |
|       | 4    | 2.0000 | 0.4355    | 0.9285         |           |
|       | 5    | 2.0000 | 0.4355    | 1.3905         |           |
|       | 6    | 1.0000 | 1.3824    | 0.9196         |           |
| B5    | 1    | 2.0000 | 142.8654  | 0.0867         |           |
|       | 2    | 2.0000 | 31.4764   | 0.6196         |           |

Continued on next page

Table S28: The basis info of molecule B<sub>8</sub> triplet.

|                        |      |        | $n_{a,k}$ | $\alpha_{a,k}$ | $c_{a,k}$ |
|------------------------|------|--------|-----------|----------------|-----------|
| Model                  | Atom | $k$    |           |                |           |
| NLIS3                  |      | 3      | 2.0000    | 10.0085        | 1.1053    |
|                        |      | 4      | 2.0000    | 0.4354         | 0.9279    |
|                        |      | 5      | 2.0000    | 0.4354         | 1.3897    |
|                        |      | 6      | 1.0000    | 1.3828         | 0.9215    |
|                        | B1   | 1      | 2.0000    | 128.9698       | 0.1033    |
|                        |      | 2      | 2.0000    | 28.6335        | 0.6838    |
|                        |      | 3      | 2.0000    | 9.2256         | 1.0621    |
|                        |      | 4      | 2.0000    | 0.4481         | 2.7972    |
|                        |      | 5      | 1.0000    | 0.3222         | 0.0000    |
|                        |      | 6      | 1.0000    | 0.3222         | 0.0000    |
|                        | B2   | 1      | 2.0000    | 142.8877       | 0.0867    |
|                        |      | 2      | 2.0000    | 31.4808        | 0.6196    |
|                        |      | 3      | 2.0000    | 10.0095        | 1.1053    |
|                        |      | 4      | 2.0000    | 0.4354         | 2.3168    |
|                        |      | 5      | 1.0000    | 1.3828         | 0.5745    |
|                        |      | 6      | 1.0000    | 1.3828         | 0.3480    |
|                        | B3   | 1      | 2.0000    | 142.8738       | 0.0867    |
|                        |      | 2      | 2.0000    | 31.4779        | 0.6196    |
|                        |      | 3      | 2.0000    | 10.0087        | 1.1053    |
|                        |      | 4      | 2.0000    | 0.4355         | 2.3183    |
|                        |      | 5      | 1.0000    | 1.3827         | 0.5740    |
|                        |      | 6      | 1.0000    | 1.3827         | 0.3463    |
|                        | B4   | 1      | 2.0000    | 142.8550       | 0.0867    |
|                        |      | 2      | 2.0000    | 31.4742        | 0.6197    |
| 3                      |      | 2.0000 | 10.0078   | 1.1053         |           |
| 4                      |      | 2.0000 | 0.4355    | 2.3190         |           |
| 5                      |      | 1.0000 | 1.3824    | 0.5737         |           |
| 6                      |      | 1.0000 | 1.3824    | 0.3458         |           |
| B5                     | 1    | 2.0000 | 142.8654  | 0.0867         |           |
|                        | 2    | 2.0000 | 31.4764   | 0.6196         |           |
|                        | 3    | 2.0000 | 10.0085   | 1.1053         |           |
|                        | 4    | 2.0000 | 0.4354    | 2.3177         |           |
|                        | 5    | 1.0000 | 1.3828    | 0.5740         |           |
| Continued on next page |      |        |           |                |           |



Table S28: The basis info of molecule B<sub>8</sub> triplet.

| Model | Atom | $k$ | $n_{a,k}$ | $\alpha_{a,k}$ | $c_{a,k}$ |
|-------|------|-----|-----------|----------------|-----------|
| NLIS4 | B1   | 6   | 1.0000    | 1.3828         | 0.3475    |
|       |      | 1   | 1.0000    | 10.5590        | 1.0428    |
|       |      | 2   | 1.0000    | 10.5590        | 0.6444    |
|       |      | 3   | 1.0000    | 1.6602         | 1.4320    |
|       |      | 4   | 1.0000    | 1.6602         | 0.5641    |
|       |      | 5   | 1.0000    | 1.6602         | 0.8168    |
|       | B2   | 6   | 1.0000    | 1.6602         | 0.4015    |
|       |      | 1   | 1.0000    | 10.6772        | 1.0354    |
|       |      | 2   | 1.0000    | 10.6772        | 0.6332    |
|       |      | 3   | 1.0000    | 1.6775         | 1.1153    |
|       |      | 4   | 1.0000    | 1.6775         | 1.1783    |
|       |      | 5   | 1.0000    | 1.6775         | 0.4867    |
|       | B3   | 6   | 1.0000    | 1.6775         | 0.5649    |
|       |      | 1   | 1.0000    | 10.6770        | 1.0354    |
|       |      | 2   | 1.0000    | 10.6770        | 0.6332    |
|       |      | 3   | 1.0000    | 1.6772         | 1.1157    |
|       |      | 4   | 1.0000    | 1.6772         | 1.1786    |
|       |      | 5   | 1.0000    | 1.6772         | 0.4865    |
|       | B4   | 6   | 1.0000    | 1.6772         | 0.5650    |
|       |      | 1   | 1.0000    | 10.6766        | 1.0355    |
|       |      | 2   | 1.0000    | 10.6766        | 0.6332    |
|       |      | 3   | 1.0000    | 1.6768         | 1.1156    |
|       |      | 4   | 1.0000    | 1.6768         | 1.1782    |
|       |      | 5   | 1.0000    | 1.6768         | 0.4879    |
|       | B5   | 6   | 1.0000    | 1.6768         | 0.5650    |
|       |      | 1   | 1.0000    | 10.6770        | 1.0354    |
|       |      | 2   | 1.0000    | 10.6770        | 0.6332    |
|       |      | 3   | 1.0000    | 1.6773         | 1.1153    |
|       |      | 4   | 1.0000    | 1.6773         | 1.1784    |
|       |      | 5   | 1.0000    | 1.6773         | 0.4869    |
| MBIS  | B1   | 6   | 1.0000    | 1.6773         | 0.5649    |
|       |      | 1   | 1.0000    | 10.5590        | 1.6872    |
|       |      | 2   | 1.0000    | 1.6602         | 3.2145    |

Continued on next page

Table S28: The basis info of molecule B<sub>8</sub> triplet.

|       |      |     | $n_{a,k}$ | $\alpha_{a,k}$ | $c_{a,k}$ |
|-------|------|-----|-----------|----------------|-----------|
| Model | Atom | $k$ |           |                |           |
| GMBIS | B2   | 1   | 1.0000    | 10.6772        | 1.6686    |
|       |      | 2   | 1.0000    | 1.6775         | 3.3451    |
|       | B3   | 1   | 1.0000    | 10.6770        | 1.6686    |
|       |      | 2   | 1.0000    | 1.6772         | 3.3459    |
|       | B4   | 1   | 1.0000    | 10.6766        | 1.6687    |
|       |      | 2   | 1.0000    | 1.6768         | 3.3467    |
|       | B5   | 1   | 1.0000    | 10.6770        | 1.6686    |
|       |      | 2   | 1.0000    | 1.6773         | 3.3455    |
|       | B1   | 1   | 1.0690    | 10.8038        | 1.6736    |
|       |      | 2   | 1.0000    | 1.6675         | 3.2234    |
|       | B2   | 1   | 1.0690    | 10.9259        | 1.6564    |
|       |      | 2   | 1.0000    | 1.6814         | 3.3581    |
|       | B3   | 1   | 1.0690    | 10.9257        | 1.6565    |
|       |      | 2   | 1.0000    | 1.6812         | 3.3586    |
|       | B4   | 1   | 1.0690    | 10.9252        | 1.6566    |
|       |      | 2   | 1.0000    | 1.6807         | 3.3596    |
|       | B5   | 1   | 1.0690    | 10.9257        | 1.6565    |
|       |      | 2   | 1.0000    | 1.6812         | 3.3584    |

## S2.14 B<sub>8</sub><sup>2-</sup>

Table S29: The basis info of molecule B<sub>8</sub><sup>2-</sup>.

| Model | Atom | <i>k</i> | $n_{a,k}$ | $\alpha_{a,k}$ | $c_{a,k}$ |
|-------|------|----------|-----------|----------------|-----------|
| LISA1 | B1   | 1        | 2.0000    | 98.2299        | 0.1490    |
|       |      | 2        | 2.0000    | 27.7169        | 0.5890    |
|       |      | 3        | 2.0000    | 9.7959         | 1.0939    |
|       |      | 4        | 2.0000    | 0.5004         | 2.3567    |
|       |      | 5        | 2.0000    | 0.1942         | 0.0000    |
|       |      | 6        | 2.0000    | 0.0618         | 0.0000    |
|       | B2   | 1        | 2.0000    | 98.2299        | 0.1478    |
|       |      | 2        | 2.0000    | 27.7169        | 0.6031    |
|       |      | 3        | 2.0000    | 9.7959         | 1.0743    |
|       |      | 4        | 2.0000    | 0.5004         | 2.3139    |
|       |      | 5        | 2.0000    | 0.1942         | 1.0452    |
|       |      | 6        | 2.0000    | 0.0618         | 0.2186    |
|       | B3   | 1        | 2.0000    | 98.2299        | 0.1478    |
|       |      | 2        | 2.0000    | 27.7169        | 0.6032    |
|       |      | 3        | 2.0000    | 9.7959         | 1.0743    |
|       |      | 4        | 2.0000    | 0.5004         | 2.3149    |
|       |      | 5        | 2.0000    | 0.1942         | 1.0430    |
|       |      | 6        | 2.0000    | 0.0618         | 0.2176    |
|       | B4   | 1        | 2.0000    | 98.2299        | 0.1478    |
|       |      | 2        | 2.0000    | 27.7169        | 0.6032    |
|       |      | 3        | 2.0000    | 9.7959         | 1.0742    |
|       |      | 4        | 2.0000    | 0.5004         | 2.3152    |
|       |      | 5        | 2.0000    | 0.1942         | 1.0428    |
|       |      | 6        | 2.0000    | 0.0618         | 0.2186    |
|       | B5   | 1        | 2.0000    | 98.2299        | 0.1478    |
|       |      | 2        | 2.0000    | 27.7169        | 0.6031    |
|       |      | 3        | 2.0000    | 9.7959         | 1.0743    |
|       |      | 4        | 2.0000    | 0.5004         | 2.3144    |
|       |      | 5        | 2.0000    | 0.1942         | 1.0443    |
|       |      | 6        | 2.0000    | 0.0618         | 0.2179    |

Continued on next page

Table S29: The basis info of molecule  $B_8^{2-}$ .

| Model | Atom | $k$ | $n_{a,k}$ | $\alpha_{a,k}$ | $c_{a,k}$ |
|-------|------|-----|-----------|----------------|-----------|
|       |      |     |           |                |           |
| LISA2 | B1   | 1   | 2.0000    | 98.2299        | 0.1490    |
|       |      | 2   | 2.0000    | 27.7169        | 0.5890    |
|       |      | 3   | 2.0000    | 9.7959         | 1.0939    |
|       |      | 4   | 2.0000    | 0.5004         | 2.3567    |
|       |      | 5   | 2.0000    | 0.1942         | 0.0000    |
|       |      | 6   | 2.0000    | 0.0618         | 0.0000    |
|       | B2   | 1   | 2.0000    | 98.2299        | 0.1478    |
|       |      | 2   | 2.0000    | 27.7169        | 0.6031    |
|       |      | 3   | 2.0000    | 9.7959         | 1.0743    |
|       |      | 4   | 2.0000    | 0.5004         | 2.3139    |
|       |      | 5   | 2.0000    | 0.1942         | 1.0452    |
|       |      | 6   | 2.0000    | 0.0618         | 0.2186    |
|       | B3   | 1   | 2.0000    | 98.2299        | 0.1478    |
|       |      | 2   | 2.0000    | 27.7169        | 0.6032    |
|       |      | 3   | 2.0000    | 9.7959         | 1.0743    |
|       |      | 4   | 2.0000    | 0.5004         | 2.3149    |
|       |      | 5   | 2.0000    | 0.1942         | 1.0430    |
|       |      | 6   | 2.0000    | 0.0618         | 0.2176    |
|       | B4   | 1   | 2.0000    | 98.2299        | 0.1478    |
|       |      | 2   | 2.0000    | 27.7169        | 0.6032    |
|       |      | 3   | 2.0000    | 9.7959         | 1.0742    |
|       |      | 4   | 2.0000    | 0.5004         | 2.3152    |
|       |      | 5   | 2.0000    | 0.1942         | 1.0428    |
|       |      | 6   | 2.0000    | 0.0618         | 0.2186    |
|       | B5   | 1   | 2.0000    | 98.2299        | 0.1478    |
|       |      | 2   | 2.0000    | 27.7169        | 0.6031    |
|       |      | 3   | 2.0000    | 9.7959         | 1.0743    |
|       |      | 4   | 2.0000    | 0.5004         | 2.3144    |
|       |      | 5   | 2.0000    | 0.1942         | 1.0443    |
|       |      | 6   | 2.0000    | 0.0618         | 0.2179    |
| LISA3 | --   | --  | --        | --             | --        |
| LISA4 | B1   | 1   | 2.0000    | 303.6041       | 0.0158    |
|       |      | 2   | 2.0000    | 148.4830       | 0.0000    |

Continued on next page

Table S29: The basis info of molecule  $B_8^{2-}$ .

| Model                  | Atom | $k$ | $n_{a,k}$ | $\alpha_{a,k}$ | $c_{a,k}$ |
|------------------------|------|-----|-----------|----------------|-----------|
|                        |      | 3   | 2.0000    | 130.1460       | 0.0368    |
|                        |      | 4   | 2.0000    | 65.3637        | 0.1100    |
|                        |      | 5   | 2.0000    | 32.6810        | 0.0000    |
|                        |      | 6   | 2.0000    | 29.0242        | 0.4866    |
|                        |      | 7   | 2.0000    | 21.7035        | 0.1191    |
|                        |      | 8   | 2.0000    | 9.5565         | 1.0655    |
|                        |      | 9   | 2.0000    | 0.5301         | 2.0559    |
|                        |      | 10  | 2.0000    | 0.3357         | 0.2709    |
|                        |      | 11  | 2.0000    | 0.2382         | 0.0000    |
|                        |      | 12  | 2.0000    | 0.1830         | 0.0000    |
|                        |      | 13  | 2.0000    | 0.1617         | 0.0000    |
|                        |      | 14  | 2.0000    | 0.0746         | 0.0000    |
|                        |      | 15  | 2.0000    | 0.0547         | 0.0000    |
|                        |      | 16  | 2.0000    | 0.0492         | 0.0000    |
|                        | B2   | 1   | 2.0000    | 303.6041       | 0.0156    |
|                        |      | 2   | 2.0000    | 148.4830       | 0.0000    |
|                        |      | 3   | 2.0000    | 130.1460       | 0.0391    |
|                        |      | 4   | 2.0000    | 65.3637        | 0.1050    |
|                        |      | 5   | 2.0000    | 32.6810        | 0.0000    |
|                        |      | 6   | 2.0000    | 29.0242        | 0.5071    |
|                        |      | 7   | 2.0000    | 21.7035        | 0.1033    |
|                        |      | 8   | 2.0000    | 9.5565         | 1.0667    |
|                        |      | 9   | 2.0000    | 0.5301         | 1.4553    |
|                        |      | 10  | 2.0000    | 0.3357         | 1.3997    |
|                        |      | 11  | 2.0000    | 0.2382         | 0.0000    |
|                        |      | 12  | 2.0000    | 0.1830         | 0.0000    |
|                        |      | 13  | 2.0000    | 0.1617         | 0.4885    |
|                        |      | 14  | 2.0000    | 0.0746         | 0.1267    |
|                        |      | 15  | 2.0000    | 0.0547         | 0.0000    |
|                        |      | 16  | 2.0000    | 0.0492         | 0.0996    |
|                        | B3   | 1   | 2.0000    | 303.6041       | 0.0156    |
|                        |      | 2   | 2.0000    | 148.4830       | 0.0000    |
|                        |      | 3   | 2.0000    | 130.1460       | 0.0391    |
| Continued on next page |      |     |           |                |           |

Table S29: The basis info of molecule  $B_8^{2-}$ .

| Model                  | Atom | $k$ | $n_{a,k}$ | $\alpha_{a,k}$ | $c_{a,k}$ |
|------------------------|------|-----|-----------|----------------|-----------|
|                        |      | 4   | 2.0000    | 65.3637        | 0.1051    |
|                        |      | 5   | 2.0000    | 32.6810        | 0.0000    |
|                        |      | 6   | 2.0000    | 29.0242        | 0.5070    |
|                        |      | 7   | 2.0000    | 21.7035        | 0.1033    |
|                        |      | 8   | 2.0000    | 9.5565         | 1.0667    |
|                        |      | 9   | 2.0000    | 0.5301         | 1.4546    |
|                        |      | 10  | 2.0000    | 0.3357         | 1.4021    |
|                        |      | 11  | 2.0000    | 0.2382         | 0.0000    |
|                        |      | 12  | 2.0000    | 0.1830         | 0.0000    |
|                        |      | 13  | 2.0000    | 0.1617         | 0.4849    |
|                        |      | 14  | 2.0000    | 0.0746         | 0.1288    |
|                        |      | 15  | 2.0000    | 0.0547         | 0.0000    |
|                        |      | 16  | 2.0000    | 0.0492         | 0.0977    |
|                        | B4   | 1   | 2.0000    | 303.6041       | 0.0156    |
|                        |      | 2   | 2.0000    | 148.4830       | 0.0000    |
|                        |      | 3   | 2.0000    | 130.1460       | 0.0391    |
|                        |      | 4   | 2.0000    | 65.3637        | 0.1050    |
|                        |      | 5   | 2.0000    | 32.6810        | 0.0000    |
|                        |      | 6   | 2.0000    | 29.0242        | 0.5071    |
|                        |      | 7   | 2.0000    | 21.7035        | 0.1033    |
|                        |      | 8   | 2.0000    | 9.5565         | 1.0667    |
|                        |      | 9   | 2.0000    | 0.5301         | 1.4542    |
|                        |      | 10  | 2.0000    | 0.3357         | 1.4029    |
|                        |      | 11  | 2.0000    | 0.2382         | 0.0000    |
|                        |      | 12  | 2.0000    | 0.1830         | 0.0000    |
|                        |      | 13  | 2.0000    | 0.1617         | 0.4847    |
|                        |      | 14  | 2.0000    | 0.0746         | 0.1280    |
|                        |      | 15  | 2.0000    | 0.0547         | 0.0000    |
|                        |      | 16  | 2.0000    | 0.0492         | 0.0989    |
|                        | B5   | 1   | 2.0000    | 303.6041       | 0.0156    |
|                        |      | 2   | 2.0000    | 148.4830       | 0.0000    |
|                        |      | 3   | 2.0000    | 130.1460       | 0.0391    |
|                        |      | 4   | 2.0000    | 65.3637        | 0.1050    |
| Continued on next page |      |     |           |                |           |

Table S29: The basis info of molecule  $B_8^{2-}$ .

|       |        |       | $n_{a,k}$ | $\alpha_{a,k}$ | $c_{a,k}$ |         |        |
|-------|--------|-------|-----------|----------------|-----------|---------|--------|
| Model | Atom   | $k$   |           |                |           |         |        |
|       |        | 5     | 2.0000    | 32.6810        | 0.0000    |         |        |
|       |        | 6     | 2.0000    | 29.0242        | 0.5072    |         |        |
|       |        | 7     | 2.0000    | 21.7035        | 0.1032    |         |        |
|       |        | 8     | 2.0000    | 9.5565         | 1.0668    |         |        |
|       |        | 9     | 2.0000    | 0.5301         | 1.4545    |         |        |
|       |        | 10    | 2.0000    | 0.3357         | 1.4019    |         |        |
|       |        | 11    | 2.0000    | 0.2382         | 0.0000    |         |        |
|       |        | 12    | 2.0000    | 0.1830         | 0.0000    |         |        |
|       |        | 13    | 2.0000    | 0.1617         | 0.4860    |         |        |
|       |        | 14    | 2.0000    | 0.0746         | 0.1283    |         |        |
|       |        | 15    | 2.0000    | 0.0547         | 0.0000    |         |        |
|       |        | 16    | 2.0000    | 0.0492         | 0.0983    |         |        |
|       |        | LISA5 | --        | --             | --        | --      | --     |
|       |        | LISA6 | B1        | 1              | 1.0000    | 10.5516 | 1.6901 |
|       |        |       |           | 2              | 1.0000    | 2.1001  | 0.0000 |
|       |        |       |           | 3              | 1.0000    | 1.8017  | 2.5162 |
| 4     | 1.0000 |       |           | 1.4928         | 0.0652    |         |        |
| 5     | 1.0000 |       |           | 0.8188         | 0.0000    |         |        |
| 6     | 1.0000 |       |           | 0.6970         | 0.0000    |         |        |
| B2    | 1      |       | 1.0000    | 10.5516        | 1.7093    |         |        |
|       | 2      |       | 1.0000    | 2.1001         | 0.0000    |         |        |
|       | 3      |       | 1.0000    | 1.8017         | 0.3726    |         |        |
|       | 4      |       | 1.0000    | 1.4928         | 3.2164    |         |        |
|       | 5      |       | 1.0000    | 0.8188         | 0.0000    |         |        |
|       | 6      |       | 1.0000    | 0.6970         | 0.0921    |         |        |
| B3    | 1      |       | 1.0000    | 10.5516        | 1.7095    |         |        |
|       | 2      |       | 1.0000    | 2.1001         | 0.0000    |         |        |
|       | 3      |       | 1.0000    | 1.8017         | 0.3635    |         |        |
|       | 4      |       | 1.0000    | 1.4928         | 3.2287    |         |        |
|       | 5      |       | 1.0000    | 0.8188         | 0.0000    |         |        |
|       | 6      |       | 1.0000    | 0.6970         | 0.0872    |         |        |
| B4    | 1      |       | 1.0000    | 10.5516        | 1.7096    |         |        |
|       | 2      |       | 1.0000    | 2.1001         | 0.0000    |         |        |

Continued on next page

Table S29: The basis info of molecule  $B_8^{2-}$ .

|                        |      |     | $n_{a,k}$ | $\alpha_{a,k}$ | $c_{a,k}$ |
|------------------------|------|-----|-----------|----------------|-----------|
| Model                  | Atom | $k$ |           |                |           |
|                        |      | 3   | 1.0000    | 1.8017         | 0.3617    |
|                        |      | 4   | 1.0000    | 1.4928         | 3.2298    |
|                        |      | 5   | 1.0000    | 0.8188         | 0.0000    |
|                        |      | 6   | 1.0000    | 0.6970         | 0.0918    |
|                        | B5   | 1   | 1.0000    | 10.5516        | 1.7095    |
|                        |      | 2   | 1.0000    | 2.1001         | 0.0000    |
|                        |      | 3   | 1.0000    | 1.8017         | 0.3660    |
|                        |      | 4   | 1.0000    | 1.4928         | 3.2251    |
|                        |      | 5   | 1.0000    | 0.8188         | 0.0000    |
|                        |      | 6   | 1.0000    | 0.6970         | 0.0888    |
| NLIS1                  | B1   | 1   | 2.0000    | 131.5279       | 0.0997    |
|                        |      | 2   | 2.0000    | 29.1443        | 0.6711    |
|                        |      | 3   | 2.0000    | 9.3480         | 1.0743    |
|                        |      | 4   | 2.0000    | 0.4948         | 0.7168    |
|                        |      | 5   | 2.0000    | 0.4948         | 1.6121    |
|                        |      | 6   | 2.0000    | 0.0275         | 0.0002    |
|                        | B2   | 1   | 2.0000    | 128.0611       | 0.1051    |
|                        |      | 2   | 2.0000    | 28.4838        | 0.6894    |
|                        |      | 3   | 2.0000    | 9.2331         | 1.0549    |
|                        |      | 4   | 2.0000    | 0.4369         | 2.7352    |
|                        |      | 5   | 2.0000    | 0.1470         | 0.6825    |
|                        |      | 6   | 2.0000    | 0.0499         | 0.1372    |
|                        | B3   | 1   | 2.0000    | 128.0521       | 0.1051    |
|                        |      | 2   | 2.0000    | 28.4819        | 0.6894    |
|                        |      | 3   | 2.0000    | 9.2326         | 1.0549    |
|                        |      | 4   | 2.0000    | 0.4367         | 2.7371    |
|                        |      | 5   | 2.0000    | 0.1467         | 0.6806    |
|                        |      | 6   | 2.0000    | 0.0500         | 0.1360    |
|                        | B4   | 1   | 2.0000    | 128.0478       | 0.1051    |
|                        |      | 2   | 2.0000    | 28.4810        | 0.6895    |
|                        |      | 3   | 2.0000    | 9.2324         | 1.0549    |
|                        |      | 4   | 2.0000    | 0.4367         | 2.7373    |
|                        |      | 5   | 2.0000    | 0.1468         | 0.6799    |
| Continued on next page |      |     |           |                |           |



Table S29: The basis info of molecule  $B_8^{2-}$ .

| Model | Atom | $k$    | $n_{a,k}$ | $\alpha_{a,k}$ | $c_{a,k}$ |
|-------|------|--------|-----------|----------------|-----------|
| NLIS2 | B5   | 6      | 2.0000    | 0.0499         | 0.1368    |
|       |      | 1      | 2.0000    | 128.0542       | 0.1051    |
|       |      | 2      | 2.0000    | 28.4824        | 0.6894    |
|       |      | 3      | 2.0000    | 9.2327         | 1.0549    |
|       |      | 4      | 2.0000    | 0.4368         | 2.7366    |
|       |      | 5      | 2.0000    | 0.1468         | 0.6812    |
|       |      | 6      | 2.0000    | 0.0499         | 0.1365    |
|       | B1   | 1      | 2.0000    | 130.7851       | 0.1007    |
|       |      | 2      | 2.0000    | 28.9956        | 0.6747    |
|       |      | 3      | 2.0000    | 9.3119         | 1.0711    |
|       |      | 4      | 2.0000    | 0.4924         | 0.9565    |
|       |      | 5      | 2.0000    | 0.4924         | 1.3792    |
|       |      | 6      | 1.0000    | 0.5298         | 0.0000    |
|       |      | B2     | 1         | 2.0000         | 131.0756  |
| 2     |      |        | 2.0000    | 29.1095        | 0.6733    |
| 3     |      |        | 2.0000    | 9.4103         | 1.0648    |
| 4     |      |        | 2.0000    | 0.4227         | 1.0330    |
| 5     |      |        | 2.0000    | 0.4227         | 1.5017    |
| 6     |      |        | 1.0000    | 1.0376         | 1.0298    |
| B3    |      | 1      | 2.0000    | 131.1082       | 0.1008    |
|       | 2    | 2.0000 | 29.1161   | 0.6731         |           |
|       | 3    | 2.0000 | 9.4119    | 1.0649         |           |
|       | 4    | 2.0000 | 0.4227    | 1.0327         |           |
|       | 5    | 2.0000 | 0.4227    | 1.5014         |           |
|       | 6    | 1.0000 | 1.0388    | 1.0289         |           |
| B4    | 1    | 2.0000 | 131.0574  | 0.1009         |           |
|       | 2    | 2.0000 | 29.1058   | 0.6734         |           |
|       | 3    | 2.0000 | 9.4093    | 1.0647         |           |
|       | 4    | 2.0000 | 0.4226    | 1.0339         |           |
|       | 5    | 2.0000 | 0.4226    | 1.5029         |           |
|       | 6    | 1.0000 | 1.0372    | 1.0267         |           |
| B5    | 1    | 2.0000 | 131.0984  | 0.1008         |           |
|       | 2    | 2.0000 | 29.1141   | 0.6731         |           |

Continued on next page

Table S29: The basis info of molecule  $B_8^{2-}$ .

|       |      |        | $n_{a,k}$ | $\alpha_{a,k}$ | $c_{a,k}$ |
|-------|------|--------|-----------|----------------|-----------|
| Model | Atom | $k$    |           |                |           |
| NLIS3 |      | 3      | 2.0000    | 9.4115         | 1.0649    |
|       |      | 4      | 2.0000    | 0.4227         | 1.0327    |
|       |      | 5      | 2.0000    | 0.4227         | 1.5014    |
|       |      | 6      | 1.0000    | 1.0384         | 1.0296    |
|       | B1   | 1      | 2.0000    | 130.7851       | 0.1007    |
|       |      | 2      | 2.0000    | 28.9956        | 0.6747    |
|       |      | 3      | 2.0000    | 9.3119         | 1.0711    |
|       |      | 4      | 2.0000    | 0.4924         | 2.3357    |
|       |      | 5      | 1.0000    | 0.5296         | 0.0000    |
|       |      | 6      | 1.0000    | 0.5296         | 0.0000    |
|       | B2   | 1      | 2.0000    | 131.0756       | 0.1008    |
|       |      | 2      | 2.0000    | 29.1095        | 0.6733    |
|       |      | 3      | 2.0000    | 9.4103         | 1.0648    |
|       |      | 4      | 2.0000    | 0.4227         | 2.5346    |
|       |      | 5      | 1.0000    | 1.0376         | 0.6582    |
|       |      | 6      | 1.0000    | 1.0376         | 0.3716    |
|       | B3   | 1      | 2.0000    | 131.1082       | 0.1008    |
|       |      | 2      | 2.0000    | 29.1161        | 0.6731    |
|       |      | 3      | 2.0000    | 9.4119         | 1.0649    |
|       |      | 4      | 2.0000    | 0.4227         | 2.5341    |
|       |      | 5      | 1.0000    | 1.0388         | 0.6581    |
|       |      | 6      | 1.0000    | 1.0388         | 0.3708    |
|       | B4   | 1      | 2.0000    | 131.0574       | 0.1009    |
|       |      | 2      | 2.0000    | 29.1058        | 0.6734    |
| 3     |      | 2.0000 | 9.4093    | 1.0647         |           |
| 4     |      | 2.0000 | 0.4226    | 2.5368         |           |
| 5     |      | 1.0000 | 1.0372    | 0.6554         |           |
| 6     |      | 1.0000 | 1.0372    | 0.3712         |           |
| B5    | 1    | 2.0000 | 131.0984  | 0.1008         |           |
|       | 2    | 2.0000 | 29.1141   | 0.6731         |           |
|       | 3    | 2.0000 | 9.4115    | 1.0649         |           |
|       | 4    | 2.0000 | 0.4227    | 2.5341         |           |
|       | 5    | 1.0000 | 1.0384    | 0.6571         |           |

Continued on next page

Table S29: The basis info of molecule  $B_8^{2-}$ .

| Model | Atom | $k$ | $n_{a,k}$ | $\alpha_{a,k}$ | $c_{a,k}$ |
|-------|------|-----|-----------|----------------|-----------|
| NLIS4 | B1   | 6   | 1.0000    | 1.0384         | 0.3725    |
|       |      | 1   | 1.0000    | 10.4181        | 1.0606    |
|       |      | 2   | 1.0000    | 10.4181        | 0.6568    |
|       |      | 3   | 1.0000    | 1.7014         | 1.3016    |
|       |      | 4   | 1.0000    | 1.7014         | 1.3845    |
|       |      | 5   | 1.0000    | 1.7014         | 0.0000    |
|       |      | 6   | 1.0000    | 1.7014         | 0.0000    |
|       | B2   | 1   | 1.0000    | 10.4891        | 1.0641    |
|       |      | 2   | 1.0000    | 10.4891        | 0.6471    |
|       |      | 3   | 1.0000    | 1.5343         | 1.4229    |
|       |      | 4   | 1.0000    | 1.5343         | 1.4561    |
|       |      | 5   | 1.0000    | 0.6282         | 0.0848    |
|       |      | 6   | 1.0000    | 1.5343         | 0.6971    |
|       | B3   | 1   | 1.0000    | 10.4888        | 1.0642    |
|       |      | 2   | 1.0000    | 10.4888        | 0.6471    |
|       |      | 3   | 1.0000    | 1.5337         | 1.4241    |
|       |      | 4   | 1.0000    | 1.5337         | 1.4572    |
|       |      | 5   | 1.0000    | 0.6282         | 0.0797    |
|       |      | 6   | 1.0000    | 1.5337         | 0.6975    |
|       | B4   | 1   | 1.0000    | 10.4885        | 1.0642    |
|       |      | 2   | 1.0000    | 10.4885        | 0.6472    |
|       |      | 3   | 1.0000    | 1.5336         | 1.4242    |
|       |      | 4   | 1.0000    | 1.5336         | 1.4569    |
|       |      | 5   | 1.0000    | 0.6282         | 0.0845    |
|       |      | 6   | 1.0000    | 1.5336         | 0.6972    |
|       | B5   | 1   | 1.0000    | 10.4888        | 1.0642    |
|       |      | 2   | 1.0000    | 10.4888        | 0.6471    |
|       |      | 3   | 1.0000    | 1.5339         | 1.4236    |
|       |      | 4   | 1.0000    | 1.5339         | 1.4568    |
|       |      | 5   | 1.0000    | 0.6282         | 0.0813    |
|       |      | 6   | 1.0000    | 1.5339         | 0.6974    |
| MBIS  | B1   | 1   | 1.0000    | 10.4203        | 1.7161    |
|       |      | 2   | 1.0000    | 1.7340         | 2.5721    |

Continued on next page

Table S29: The basis info of molecule  $B_8^{2-}$ .

|       |          |     | $n_{a,k}$ | $\alpha_{a,k}$ | $c_{a,k}$ |
|-------|----------|-----|-----------|----------------|-----------|
| Model | Atom     | $k$ |           |                |           |
|       | B2       | 1   | 1.0000    | 10.3893        | 1.7336    |
|       |          | 2   | 1.0000    | 1.4764         | 3.6538    |
|       | B3       | 1   | 1.0000    | 10.3896        | 1.7335    |
|       |          | 2   | 1.0000    | 1.4765         | 3.6537    |
|       | B4       | 1   | 1.0000    | 10.3886        | 1.7337    |
|       |          | 2   | 1.0000    | 1.4757         | 3.6560    |
|       | B5       | 1   | 1.0000    | 10.3895        | 1.7335    |
|       |          | 2   | 1.0000    | 1.4765         | 3.6537    |
|       | GMBIS B1 | 1   | 1.0690    | 10.6640        | 1.7000    |
|       |          | 2   | 1.0000    | 1.7476         | 2.5777    |
|       | B2       | 1   | 1.0690    | 10.6169        | 1.7203    |
|       |          | 2   | 1.0000    | 1.4800         | 3.6690    |
|       | B3       | 1   | 1.0690    | 10.6173        | 1.7202    |
|       |          | 2   | 1.0000    | 1.4803         | 3.6684    |
|       | B4       | 1   | 1.0690    | 10.6162        | 1.7204    |
|       |          | 2   | 1.0000    | 1.4794         | 3.6710    |
|       | B5       | 1   | 1.0690    | 10.6172        | 1.7202    |
|       |          | 2   | 1.0000    | 1.4802         | 3.6687    |

## S2.15 B<sub>9</sub><sup>-</sup>

Table S30: The basis info of molecule B<sub>9</sub><sup>-</sup>.

| Model | Atom | <i>k</i> | $n_{a,k}$ | $\alpha_{a,k}$ | $c_{a,k}$ |
|-------|------|----------|-----------|----------------|-----------|
| LISA1 | B1   | 1        | 2.0000    | 98.2299        | 0.1500    |
|       |      | 2        | 2.0000    | 27.7169        | 0.5839    |
|       |      | 3        | 2.0000    | 9.7959         | 1.1044    |
|       |      | 4        | 2.0000    | 0.5004         | 2.1350    |
|       |      | 5        | 2.0000    | 0.1942         | 0.5022    |
|       |      | 6        | 2.0000    | 0.0618         | 0.0001    |
|       | B2   | 1        | 2.0000    | 98.2299        | 0.1474    |
|       |      | 2        | 2.0000    | 27.7169        | 0.6076    |
|       |      | 3        | 2.0000    | 9.7959         | 1.0687    |
|       |      | 4        | 2.0000    | 0.5004         | 2.3863    |
|       |      | 5        | 2.0000    | 0.1942         | 0.9163    |
|       |      | 6        | 2.0000    | 0.0618         | 0.0708    |
|       | B3   | 1        | 2.0000    | 98.2299        | 0.1473    |
|       |      | 2        | 2.0000    | 27.7169        | 0.6077    |
|       |      | 3        | 2.0000    | 9.7959         | 1.0685    |
|       |      | 4        | 2.0000    | 0.5004         | 2.3883    |
|       |      | 5        | 2.0000    | 0.1942         | 0.9113    |
|       |      | 6        | 2.0000    | 0.0618         | 0.0605    |
| LISA2 | B1   | 1        | 2.0000    | 98.2299        | 0.1500    |
|       |      | 2        | 2.0000    | 27.7169        | 0.5839    |
|       |      | 3        | 2.0000    | 9.7959         | 1.1044    |
|       |      | 4        | 2.0000    | 0.5004         | 2.1351    |
|       |      | 5        | 2.0000    | 0.1942         | 0.5019    |
|       |      | 6        | 2.0000    | 0.0618         | 0.0005    |
|       | B2   | 1        | 2.0000    | 98.2299        | 0.1474    |
|       |      | 2        | 2.0000    | 27.7169        | 0.6076    |
|       |      | 3        | 2.0000    | 9.7959         | 1.0687    |
|       |      | 4        | 2.0000    | 0.5004         | 2.3863    |
|       |      | 5        | 2.0000    | 0.1942         | 0.9163    |
|       |      | 6        | 2.0000    | 0.0618         | 0.0708    |

Continued on next page

Table S30: The basis info of molecule  $\text{B}_9^-$ .

|       |      |     | $n_{a,k}$ | $\alpha_{a,k}$ | $c_{a,k}$ |
|-------|------|-----|-----------|----------------|-----------|
| Model | Atom | $k$ |           |                |           |
|       | B3   | 1   | 2.0000    | 98.2299        | 0.1473    |
|       |      | 2   | 2.0000    | 27.7169        | 0.6077    |
|       |      | 3   | 2.0000    | 9.7959         | 1.0685    |
|       |      | 4   | 2.0000    | 0.5004         | 2.3884    |
|       |      | 5   | 2.0000    | 0.1942         | 0.9112    |
|       |      | 6   | 2.0000    | 0.0618         | 0.0605    |
| LISA3 | --   | --  | --        | --             | --        |
| LISA4 | B1   | 1   | 2.0000    | 303.6041       | 0.0147    |
|       |      | 2   | 2.0000    | 148.4830       | 0.0000    |
|       |      | 3   | 2.0000    | 130.1460       | 0.0444    |
|       |      | 4   | 2.0000    | 65.3637        | 0.0866    |
|       |      | 5   | 2.0000    | 32.6810        | 0.0000    |
|       |      | 6   | 2.0000    | 29.0242        | 0.5913    |
|       |      | 7   | 2.0000    | 21.7035        | 0.0000    |
|       |      | 8   | 2.0000    | 9.5565         | 1.1117    |
|       |      | 9   | 2.0000    | 0.5301         | 1.5100    |
|       |      | 10  | 2.0000    | 0.3357         | 0.9510    |
|       |      | 11  | 2.0000    | 0.2382         | 0.0000    |
|       |      | 12  | 2.0000    | 0.1830         | 0.0000    |
|       |      | 13  | 2.0000    | 0.1617         | 0.1250    |
|       |      | 14  | 2.0000    | 0.0746         | 0.0283    |
|       |      | 15  | 2.0000    | 0.0547         | 0.0000    |
|       |      | 16  | 2.0000    | 0.0492         | 0.0000    |
|       | B2   | 1   | 2.0000    | 303.6041       | 0.0163    |
|       |      | 2   | 2.0000    | 148.4830       | 0.0000    |
|       |      | 3   | 2.0000    | 130.1460       | 0.0346    |
|       |      | 4   | 2.0000    | 65.3637        | 0.1184    |
|       |      | 5   | 2.0000    | 32.6810        | 0.0000    |
|       |      | 6   | 2.0000    | 29.0242        | 0.4547    |
|       |      | 7   | 2.0000    | 21.7035        | 0.1618    |
|       |      | 8   | 2.0000    | 9.5565         | 1.0471    |
|       |      | 9   | 2.0000    | 0.5301         | 1.5991    |
|       |      | 10  | 2.0000    | 0.3357         | 1.2585    |

Continued on next page

Table S30: The basis info of molecule  $\text{B}_9^-$ .

| Model | Atom | $k$ | $n_{a,k}$ | $\alpha_{a,k}$ | $c_{a,k}$ |
|-------|------|-----|-----------|----------------|-----------|
|       |      | 11  | 2.0000    | 0.2382         | 0.0000    |
|       |      | 12  | 2.0000    | 0.1830         | 0.0000    |
|       |      | 13  | 2.0000    | 0.1617         | 0.4216    |
|       |      | 14  | 2.0000    | 0.0746         | 0.0700    |
|       |      | 15  | 2.0000    | 0.0547         | 0.0000    |
|       |      | 16  | 2.0000    | 0.0492         | 0.0152    |
|       | B3   | 1   | 2.0000    | 303.6041       | 0.0163    |
|       |      | 2   | 2.0000    | 148.4830       | 0.0000    |
|       |      | 3   | 2.0000    | 130.1460       | 0.0346    |
|       |      | 4   | 2.0000    | 65.3637        | 0.1184    |
|       |      | 5   | 2.0000    | 32.6810        | 0.0000    |
|       |      | 6   | 2.0000    | 29.0242        | 0.4548    |
|       |      | 7   | 2.0000    | 21.7035        | 0.1617    |
|       |      | 8   | 2.0000    | 9.5565         | 1.0471    |
|       |      | 9   | 2.0000    | 0.5301         | 1.5971    |
|       |      | 10  | 2.0000    | 0.3357         | 1.2635    |
|       |      | 11  | 2.0000    | 0.2382         | 0.0000    |
|       |      | 12  | 2.0000    | 0.1830         | 0.0000    |
|       |      | 13  | 2.0000    | 0.1617         | 0.4174    |
|       |      | 14  | 2.0000    | 0.0746         | 0.0586    |
|       |      | 15  | 2.0000    | 0.0547         | 0.0000    |
|       |      | 16  | 2.0000    | 0.0492         | 0.0172    |
| LISA5 | --   | --  | --        | --             | --        |
| LISA6 | B1   | 1   | 1.0000    | 10.5516        | 1.7259    |
|       |      | 2   | 1.0000    | 2.1001         | 0.0000    |
|       |      | 3   | 1.0000    | 1.8017         | 0.8885    |
|       |      | 4   | 1.0000    | 1.4928         | 2.0251    |
|       |      | 5   | 1.0000    | 0.8188         | 0.0000    |
|       |      | 6   | 1.0000    | 0.6970         | 0.0000    |
|       | B2   | 1   | 1.0000    | 10.5516        | 1.6857    |
|       |      | 2   | 1.0000    | 2.1001         | 0.0000    |
|       |      | 3   | 1.0000    | 1.8017         | 1.3440    |
|       |      | 4   | 1.0000    | 1.4928         | 2.1360    |

Continued on next page

Table S30: The basis info of molecule  $\text{B}_9^-$ .

| Model                  | Atom  | $k$ | $n_{a,k}$ | $\alpha_{a,k}$ | $c_{a,k}$ |        |
|------------------------|-------|-----|-----------|----------------|-----------|--------|
|                        | B3    | 5   | 1.0000    | 0.8188         | 0.0000    |        |
|                        |       | 6   | 1.0000    | 0.6970         | 0.0066    |        |
|                        |       | 1   | 1.0000    | 10.5516        | 1.6855    |        |
|                        |       | 2   | 1.0000    | 2.1001         | 0.0000    |        |
|                        |       | 3   | 1.0000    | 1.8017         | 1.3525    |        |
|                        |       | 4   | 1.0000    | 1.4928         | 2.1268    |        |
|                        |       | 5   | 1.0000    | 0.8188         | 0.0000    |        |
|                        |       | 6   | 1.0000    | 0.6970         | 0.0005    |        |
|                        | NLIS1 | B1  | 1         | 2.0000         | 383.1538  | 0.0140 |
|                        |       |     | 2         | 2.0000         | 78.5847   | 0.1680 |
|                        |       |     | 3         | 2.0000         | 24.2408   | 0.7040 |
|                        |       |     | 4         | 2.0000         | 8.7030    | 0.9769 |
|                        |       |     | 5         | 2.0000         | 0.4674    | 2.2647 |
|                        |       |     | 6         | 2.0000         | 0.1861    | 0.3222 |
| B2                     |       | 1   | 2.0000    | 130.7020       | 0.1015    |        |
|                        |       | 2   | 2.0000    | 29.0288        | 0.6767    |        |
|                        |       | 3   | 2.0000    | 9.3844         | 1.0661    |        |
|                        |       | 4   | 2.0000    | 0.4448         | 2.7509    |        |
|                        |       | 5   | 2.0000    | 0.1509         | 0.5682    |        |
|                        |       | 6   | 2.0000    | 0.0499         | 0.0347    |        |
| B3                     |       | 1   | 2.0000    | 130.6887       | 0.1016    |        |
|                        |       | 2   | 2.0000    | 29.0261        | 0.6768    |        |
|                        |       | 3   | 2.0000    | 9.3837         | 1.0660    |        |
|                        |       | 4   | 2.0000    | 0.4447         | 2.7519    |        |
|                        |       | 5   | 2.0000    | 0.1516         | 0.5624    |        |
|                        |       | 6   | 2.0000    | 0.0496         | 0.0308    |        |
| NLIS2                  | B1    | 1   | 2.0000    | 125.5114       | 0.1082    |        |
|                        |       | 2   | 2.0000    | 27.9429        | 0.7000    |        |
|                        |       | 3   | 2.0000    | 9.0676         | 1.0462    |        |
|                        |       | 4   | 2.0000    | 0.4505         | 0.7804    |        |
|                        |       | 5   | 2.0000    | 0.4505         | 1.4263    |        |
|                        |       | 6   | 1.0000    | 1.2543         | 0.4103    |        |
|                        | B2    | 1   | 2.0000    | 138.5238       | 0.0916    |        |
| Continued on next page |       |     |           |                |           |        |



Table S30: The basis info of molecule  $\text{B}_9^-$ .

| Model | Atom | $k$ | $n_{a,k}$ | $\alpha_{a,k}$ | $c_{a,k}$ |
|-------|------|-----|-----------|----------------|-----------|
| NLIS3 |      | 2   | 2.0000    | 30.6174        | 0.6387    |
|       |      | 3   | 2.0000    | 9.8010         | 1.0916    |
|       |      | 4   | 2.0000    | 0.4293         | 0.9642    |
|       |      | 5   | 2.0000    | 0.4293         | 1.4292    |
|       |      | 6   | 1.0000    | 1.2468         | 0.9799    |
|       | B3   | 1   | 2.0000    | 138.4593       | 0.0917    |
|       |      | 2   | 2.0000    | 30.6048        | 0.6389    |
|       |      | 3   | 2.0000    | 9.7983         | 1.0913    |
|       |      | 4   | 2.0000    | 0.4287         | 0.9679    |
|       |      | 5   | 2.0000    | 0.4287         | 1.4326    |
|       |      | 6   | 1.0000    | 1.2530         | 0.9644    |
|       | B1   | 1   | 2.0000    | 125.5114       | 0.1082    |
|       |      | 2   | 2.0000    | 27.9429        | 0.7000    |
|       |      | 3   | 2.0000    | 9.0676         | 1.0462    |
|       |      | 4   | 2.0000    | 0.4505         | 2.2066    |
|       |      | 5   | 1.0000    | 1.2543         | 0.2372    |
|       |      | 6   | 1.0000    | 1.2543         | 0.1730    |
|       | B2   | 1   | 2.0000    | 138.5238       | 0.0916    |
|       |      | 2   | 2.0000    | 30.6174        | 0.6387    |
|       |      | 3   | 2.0000    | 9.8010         | 1.0916    |
|       |      | 4   | 2.0000    | 0.4293         | 2.3934    |
|       |      | 5   | 1.0000    | 1.2468         | 0.5941    |
|       |      | 6   | 1.0000    | 1.2468         | 0.3858    |
|       | B3   | 1   | 2.0000    | 138.4593       | 0.0917    |
|       |      | 2   | 2.0000    | 30.6048        | 0.6389    |
|       |      | 3   | 2.0000    | 9.7983         | 1.0913    |
|       |      | 4   | 2.0000    | 0.4287         | 2.4005    |
|       |      | 5   | 1.0000    | 1.2530         | 0.5870    |
|       |      | 6   | 1.0000    | 1.2530         | 0.3774    |
| NLIS4 | B1   | 1   | 1.0000    | 10.3320        | 1.0692    |
|       |      | 2   | 1.0000    | 10.3320        | 0.6736    |
|       |      | 3   | 1.0000    | 1.5860         | 0.6017    |
|       |      | 4   | 1.0000    | 1.5860         | 0.7739    |

Continued on next page

Table S30: The basis info of molecule  $\text{B}_9^-$ .

| Model | Atom | $k$ | $n_{a,k}$ | $\alpha_{a,k}$ | $c_{a,k}$ |
|-------|------|-----|-----------|----------------|-----------|
|       |      | 5   | 1.0000    | 1.5860         | 0.9078    |
|       |      | 6   | 1.0000    | 1.5860         | 0.5945    |
|       | B2   | 1   | 1.0000    | 10.5984        | 1.0490    |
|       |      | 2   | 1.0000    | 10.5984        | 0.6387    |
|       |      | 3   | 1.0000    | 1.6073         | 1.3728    |
|       |      | 4   | 1.0000    | 1.6073         | 1.4170    |
|       |      | 5   | 1.0000    | 0.5024         | 0.0092    |
|       |      | 6   | 1.0000    | 1.6073         | 0.6888    |
|       | B3   | 1   | 1.0000    | 10.5992        | 1.0489    |
|       |      | 2   | 1.0000    | 10.5992        | 0.6386    |
|       |      | 3   | 1.0000    | 1.6077         | 1.3719    |
|       |      | 4   | 1.0000    | 1.6077         | 1.4175    |
|       |      | 5   | 1.0000    | 0.5021         | 0.0008    |
|       |      | 6   | 1.0000    | 1.6077         | 0.6889    |
| MBIS  | B1   | 1   | 1.0000    | 10.3283        | 1.7436    |
|       |      | 2   | 1.0000    | 1.5867         | 2.8669    |
|       | B2   | 1   | 1.0000    | 10.5863        | 1.6904    |
|       |      | 2   | 1.0000    | 1.6007         | 3.4832    |
|       | B3   | 1   | 1.0000    | 10.5874        | 1.6902    |
|       |      | 2   | 1.0000    | 1.6016         | 3.4810    |
| GMBIS | B1   | 1   | 1.0690    | 10.5540        | 1.7288    |
|       |      | 2   | 1.0000    | 1.5961         | 2.8763    |
|       | B2   | 1   | 1.0690    | 10.8278        | 1.6780    |
|       |      | 2   | 1.0000    | 1.6044         | 3.4966    |
|       | B3   | 1   | 1.0690    | 10.8292        | 1.6777    |
|       |      | 2   | 1.0000    | 1.6056         | 3.4937    |

## S3 Partitioning results with different methods

### S3.1 $\text{CH}_3^+$

Table S31: The info of molecule  $\text{CH}_3^+$ .

| Prop.        | LISA1  | LISA2  | LISA3 | LISA4  | LISA5 | LISA6  | NLIS1  | NLIS2  | NLIS3  | NLIS4  | MBIS   | GMBIS  | ISA     |
|--------------|--------|--------|-------|--------|-------|--------|--------|--------|--------|--------|--------|--------|---------|
| $q_C$        | 0.4284 | 0.4262 | --    | 0.4135 | --    | 0.1929 | 0.3925 | 0.4010 | 0.4010 | 0.3486 | 0.3486 | 0.3516 | 0.3931  |
| $q_H$        | 0.1907 | 0.1914 | --    | 0.1956 | --    | 0.2691 | 0.2026 | 0.1997 | 0.1997 | 0.2172 | 0.2172 | 0.2161 | 0.2023  |
| $s_C^I$      | 0.1470 | 0.1471 | --    | 0.1519 | --    | 0.1840 | 0.1518 | 0.1512 | 0.1512 | 0.1549 | 0.1549 | 0.1534 | 0.1521  |
| $s_H^I$      | 0.0226 | 0.0226 | --    | 0.0212 | --    | 0.0193 | 0.0204 | 0.0207 | 0.0207 | 0.0239 | 0.0239 | 0.0241 | 0.0202  |
| $s_C^{II}$   | 0.0039 | 0.0038 | --    | 0.0014 | --    | 0.0774 | 0.0004 | 0.0009 | 0.0009 | 0.0636 | 0.0636 | 0.0553 | 0.0000  |
| $s_H^{II}$   | 0.0003 | 0.0003 | --    | 0.0006 | --    | 0.0173 | 0.0000 | 0.0000 | 0.0000 | 0.0057 | 0.0057 | 0.0045 | -0.0000 |
| $s_C^{I+II}$ | 0.1509 | 0.1510 | --    | 0.1533 | --    | 0.2615 | 0.1522 | 0.1521 | 0.1521 | 0.2184 | 0.2184 | 0.2087 | 0.1521  |
| $s_H^{I+II}$ | 0.0229 | 0.0229 | --    | 0.0217 | --    | 0.0366 | 0.0204 | 0.0208 | 0.0208 | 0.0296 | 0.0296 | 0.0285 | 0.0202  |
| $S$          | 0.2197 | 0.2196 | --    | 0.2185 | --    | 0.3713 | 0.2133 | 0.2143 | 0.2143 | 0.3070 | 0.3070 | 0.2943 | 0.2128  |
| $T$          | 1.3223 | 1.3219 | --    | 1.3056 | --    | 1.7994 | 1.2864 | 1.2868 | 1.2868 | 1.6860 | 1.6860 | 1.6111 | 1.2745  |

### S3.2 $\text{CH}_4$

Table S32: The info of molecule  $\text{CH}_4$ .

| Prop.        | LISA1   | LISA2   | LISA3 | LISA4   | LISA5 | LISA6   | NLIS1   | NLIS2   | NLIS3   | NLIS4   | MBIS    | GMBIS   | ISA     |
|--------------|---------|---------|-------|---------|-------|---------|---------|---------|---------|---------|---------|---------|---------|
| $q_C$        | -0.5877 | -0.5989 | --    | -0.5615 | --    | -0.5317 | -0.6022 | -0.5466 | -0.5466 | -0.7341 | -0.7364 | -0.7544 | -0.5880 |
| $q_H$        | 0.1466  | 0.1493  | --    | 0.1400  | --    | 0.1334  | 0.1502  | 0.1367  | 0.1367  | 0.1839  | 0.1845  | 0.1889  | 0.1470  |
| $s_C^I$      | 0.0174  | 0.0174  | --    | 0.0197  | --    | 0.0240  | 0.0198  | 0.0198  | 0.0198  | 0.0213  | 0.0214  | 0.0209  | 0.0200  |
| $s_H^I$      | 0.0062  | 0.0061  | --    | 0.0052  | --    | 0.0074  | 0.0047  | 0.0049  | 0.0049  | 0.0070  | 0.0070  | 0.0070  | 0.0045  |
| $s_C^{II}$   | 0.0066  | 0.0065  | --    | 0.0024  | --    | 0.0565  | 0.0004  | 0.0016  | 0.0016  | 0.0401  | 0.0402  | 0.0337  | 0.0000  |
| $s_H^{II}$   | 0.0004  | 0.0002  | --    | 0.0002  | --    | 0.0063  | 0.0001  | 0.0000  | 0.0000  | 0.0017  | 0.0017  | 0.0012  | -0.0000 |
| $s_C^{I+II}$ | 0.0241  | 0.0240  | --    | 0.0221  | --    | 0.0806  | 0.0202  | 0.0214  | 0.0214  | 0.0614  | 0.0616  | 0.0546  | 0.0200  |
| $s_H^{I+II}$ | 0.0066  | 0.0063  | --    | 0.0054  | --    | 0.0137  | 0.0048  | 0.0049  | 0.0049  | 0.0087  | 0.0087  | 0.0081  | 0.0045  |
| $S$          | 0.0504  | 0.0492  | --    | 0.0437  | --    | 0.1354  | 0.0395  | 0.0411  | 0.0411  | 0.0961  | 0.0962  | 0.0872  | 0.0382  |

Continued on next page

Table S32: The info of molecule CH<sub>4</sub>.

| Prop. | LISA1  | LISA2  | LISA3 | LISA4  | LISA5 | LISA6  | NLIS1  | NLIS2  | NLIS3  | NLIS4  | MBIS   | GMBIS  | ISA    |
|-------|--------|--------|-------|--------|-------|--------|--------|--------|--------|--------|--------|--------|--------|
| $T$   | 0.7556 | 0.7504 | ---   | 0.6890 | ---   | 1.3084 | 0.6512 | 0.6647 | 0.6647 | 1.1093 | 1.1093 | 1.0361 | 0.6274 |

### S3.3 CH<sub>3</sub><sup>-</sup>

Table S33: The info of molecule CH<sub>3</sub><sup>-</sup>.

| Prop.        | LISA1   | LISA2   | LISA3   | LISA4   | LISA5 | LISA6   | NLIS1   | NLIS2   | NLIS3   | NLIS4   | MBIS    | GMBIS   | ISA     |
|--------------|---------|---------|---------|---------|-------|---------|---------|---------|---------|---------|---------|---------|---------|
| $q_C$        | -1.0666 | -1.0520 | -1.6058 | -1.6218 | ---   | -1.4178 | -1.6922 | -1.6835 | -1.6811 | -1.6439 | -1.9200 | -1.9390 | -1.6884 |
| $q_H$        | 0.0220  | 0.0171  | 0.2017  | 0.2071  | ---   | 0.1398  | 0.2306  | 0.2277  | 0.2270  | 0.2151  | 0.3069  | 0.3132  | 0.2295  |
| $s_C^I$      | 0.1170  | 0.0466  | 0.0864  | 0.0891  | ---   | 0.0934  | 0.0890  | 0.0888  | 0.0888  | 0.0898  | 0.1039  | 0.1040  | 0.0872  |
| $s_H^I$      | 0.0335  | 0.0385  | 0.0055  | 0.0048  | ---   | 0.0081  | 0.0039  | 0.0040  | 0.0040  | 0.0060  | 0.0058  | 0.0056  | 0.0045  |
| $s_C^{II}$   | 0.1177  | 0.0058  | 0.0004  | 0.0019  | ---   | 0.0405  | 0.0003  | 0.0010  | 0.0009  | 0.0287  | 0.0902  | 0.0891  | 0.0000  |
| $s_H^{II}$   | 0.0638  | 0.0029  | -0.0013 | 0.0002  | ---   | 0.0046  | 0.0000  | 0.0000  | 0.0000  | 0.0015  | 0.0023  | 0.0018  | -0.0000 |
| $s_C^{I+II}$ | 0.2347  | 0.0525  | 0.0868  | 0.0910  | ---   | 0.1339  | 0.0893  | 0.0898  | 0.0896  | 0.1185  | 0.1941  | 0.1931  | 0.0872  |
| $s_H^{I+II}$ | 0.0972  | 0.0414  | 0.0042  | 0.0049  | ---   | 0.0127  | 0.0039  | 0.0040  | 0.0040  | 0.0075  | 0.0081  | 0.0074  | 0.0045  |
| $S$          | 0.5262  | 0.1766  | 0.0995  | 0.1058  | ---   | 0.1719  | 0.1011  | 0.1019  | 0.1017  | 0.1410  | 0.2184  | 0.2153  | 0.1006  |
| $T$          | 1.4150  | 0.9548  | 0.8025  | 0.8147  | ---   | 1.2883  | 0.7966  | 0.7926  | 0.7798  | 1.1183  | 1.2854  | 1.2586  | 0.7757  |

### S3.4 NH<sub>4</sub><sup>+</sup>

Table S34: The info of molecule NH<sub>4</sub><sup>+</sup>.

| Prop.      | LISA1   | LISA2   | LISA3 | LISA4   | LISA5 | LISA6   | NLIS1   | NLIS2   | NLIS3   | NLIS4   | MBIS    | GMBIS   | ISA     |
|------------|---------|---------|-------|---------|-------|---------|---------|---------|---------|---------|---------|---------|---------|
| $q_N$      | -0.7607 | -0.7652 | ---   | -0.7631 | ---   | -0.5890 | -0.7787 | -0.7599 | -0.7554 | -0.8766 | -0.8766 | -0.8731 | -0.7814 |
| $q_H$      | 0.4399  | 0.4410  | ---   | 0.4405  | ---   | 0.3976  | 0.4446  | 0.4402  | 0.4391  | 0.4695  | 0.4695  | 0.4686  | 0.4453  |
| $s_N^I$    | 0.0274  | 0.0274  | ---   | 0.0273  | ---   | 0.0261  | 0.0274  | 0.0273  | 0.0274  | 0.0309  | 0.0309  | 0.0296  | 0.0275  |
| $s_H^I$    | 0.0051  | 0.0051  | ---   | 0.0050  | ---   | 0.0092  | 0.0047  | 0.0049  | 0.0048  | 0.0062  | 0.0062  | 0.0063  | 0.0047  |
| $s_N^{II}$ | 0.0022  | 0.0023  | ---   | 0.0006  | ---   | 0.1012  | 0.0003  | 0.0033  | 0.0012  | 0.0577  | 0.0577  | 0.0491  | 0.0000  |
| $s_H^{II}$ | 0.0002  | 0.0001  | ---   | 0.0001  | ---   | 0.0063  | 0.0000  | 0.0000  | 0.0000  | 0.0021  | 0.0021  | 0.0016  | -0.0000 |

Continued on next page

Table S34: The info of molecule  $\text{NH}_4^+$ .

| Prop.                        | LISA1  | LISA2  | LISA3 | LISA4  | LISA5 | LISA6  | NLIS1  | NLIS2  | NLIS3  | NLIS4  | MBIS   | GMBIS  | ISA    |
|------------------------------|--------|--------|-------|--------|-------|--------|--------|--------|--------|--------|--------|--------|--------|
| $s_{\text{N}}^{\text{I+II}}$ | 0.0296 | 0.0296 | ---   | 0.0279 | ---   | 0.1273 | 0.0277 | 0.0306 | 0.0286 | 0.0885 | 0.0885 | 0.0788 | 0.0275 |
| $s_{\text{H}}^{\text{I+II}}$ | 0.0053 | 0.0052 | ---   | 0.0051 | ---   | 0.0156 | 0.0047 | 0.0049 | 0.0049 | 0.0083 | 0.0083 | 0.0079 | 0.0047 |
| $S$                          | 0.0507 | 0.0505 | ---   | 0.0484 | ---   | 0.1895 | 0.0466 | 0.0501 | 0.0480 | 0.1218 | 0.1218 | 0.1103 | 0.0462 |
| $T$                          | 0.7132 | 0.7127 | ---   | 0.7036 | ---   | 1.5185 | 0.6962 | 0.7641 | 0.6970 | 1.2353 | 1.2353 | 1.1519 | 0.6787 |

### S3.5 $\text{NH}_3$

Table S35: The info of molecule  $\text{NH}_3$ .

| Prop.                        | LISA1   | LISA2   | LISA3   | LISA4   | LISA5 | LISA6   | NLIS1   | NLIS2   | NLIS3   | NLIS4   | MBIS    | GMBIS   | ISA     |
|------------------------------|---------|---------|---------|---------|-------|---------|---------|---------|---------|---------|---------|---------|---------|
| $q_{\text{N}}$               | -0.9850 | -0.9923 | -1.0431 | -1.0403 | ---   | -0.7399 | -1.0427 | -1.0465 | -1.0446 | -1.0757 | -1.1086 | -1.1171 | -1.0435 |
| $q_{\text{H}}$               | 0.3283  | 0.3307  | 0.3476  | 0.3467  | ---   | 0.2469  | 0.3475  | 0.3488  | 0.3483  | 0.3588  | 0.3698  | 0.3726  | 0.3479  |
| $s_{\text{N}}^{\text{I}}$    | 0.0294  | 0.0270  | 0.0296  | 0.0296  | ---   | 0.0294  | 0.0294  | 0.0296  | 0.0296  | 0.0295  | 0.0312  | 0.0310  | 0.0294  |
| $s_{\text{H}}^{\text{I}}$    | 0.0066  | 0.0067  | 0.0046  | 0.0047  | ---   | 0.0103  | 0.0046  | 0.0046  | 0.0046  | 0.0059  | 0.0055  | 0.0054  | 0.0046  |
| $s_{\text{N}}^{\text{II}}$   | 0.0048  | 0.0030  | 0.0001  | 0.0004  | ---   | 0.0907  | 0.0009  | 0.0028  | 0.0028  | 0.0301  | 0.0326  | 0.0273  | 0.0000  |
| $s_{\text{H}}^{\text{II}}$   | 0.0014  | 0.0002  | 0.0001  | 0.0001  | ---   | 0.0040  | 0.0000  | 0.0000  | 0.0000  | 0.0008  | 0.0008  | 0.0006  | -0.0000 |
| $s_{\text{N}}^{\text{I+II}}$ | 0.0342  | 0.0300  | 0.0297  | 0.0300  | ---   | 0.1200  | 0.0303  | 0.0324  | 0.0324  | 0.0596  | 0.0638  | 0.0583  | 0.0294  |
| $s_{\text{H}}^{\text{I+II}}$ | 0.0079  | 0.0069  | 0.0047  | 0.0048  | ---   | 0.0143  | 0.0046  | 0.0046  | 0.0046  | 0.0068  | 0.0063  | 0.0060  | 0.0046  |
| $S$                          | 0.0581  | 0.0507  | 0.0439  | 0.0442  | ---   | 0.1629  | 0.0441  | 0.0463  | 0.0462  | 0.0799  | 0.0827  | 0.0763  | 0.0431  |
| $T$                          | 0.6852  | 0.6742  | 0.6350  | 0.6402  | ---   | 1.3721  | 0.6545  | 0.6987  | 0.6987  | 0.9798  | 0.9824  | 0.9146  | 0.6312  |

### S3.6 $\text{NH}_2^-$

Table S36: The info of molecule  $\text{NH}_2^-$ .

| Prop.                     | LISA1   | LISA2   | LISA3   | LISA4   | LISA5 | LISA6   | NLIS1   | NLIS2   | NLIS3   | NLIS4   | MBIS    | GMBIS   | ISA     |
|---------------------------|---------|---------|---------|---------|-------|---------|---------|---------|---------|---------|---------|---------|---------|
| $q_{\text{N}}$            | -1.1829 | -1.1727 | -1.5329 | -1.5478 | ---   | -1.4676 | -1.5320 | -1.5273 | -1.5288 | -1.5326 | -1.7434 | -1.7621 | -1.5274 |
| $q_{\text{H}}$            | 0.0915  | 0.0864  | 0.2665  | 0.2739  | ---   | 0.2337  | 0.2660  | 0.2637  | 0.2648  | 0.2662  | 0.3716  | 0.3810  | 0.2637  |
| $s_{\text{N}}^{\text{I}}$ | 0.0626  | 0.0291  | 0.0435  | 0.0445  | ---   | 0.0438  | 0.0426  | 0.0428  | 0.0431  | 0.0433  | 0.0562  | 0.0569  | 0.0426  |

Continued on next page

Table S36: The info of molecule  $\text{NH}_2^-$ .

| Prop.                        | LISA1  | LISA2  | LISA3  | LISA4  | LISA5 | LISA6  | NLIS1  | NLIS2  | NLIS3  | NLIS4  | MBIS   | GMBIS  | ISA     |
|------------------------------|--------|--------|--------|--------|-------|--------|--------|--------|--------|--------|--------|--------|---------|
| $s_{\text{H}}^{\text{I}}$    | 0.0248 | 0.0331 | 0.0043 | 0.0040 | ---   | 0.0062 | 0.0047 | 0.0046 | 0.0044 | 0.0056 | 0.0056 | 0.0054 | 0.0046  |
| $s_{\text{N}}^{\text{II}}$   | 0.0891 | 0.0108 | 0.0007 | 0.0019 | ---   | 0.0475 | 0.0009 | 0.0008 | 0.0029 | 0.0274 | 0.1251 | 0.1270 | 0.0000  |
| $s_{\text{H}}^{\text{II}}$   | 0.0500 | 0.0026 | 0.0001 | 0.0001 | ---   | 0.0025 | 0.0000 | 0.0000 | 0.0002 | 0.0006 | 0.0010 | 0.0007 | -0.0000 |
| $s_{\text{N}}^{\text{I+II}}$ | 0.1516 | 0.0398 | 0.0443 | 0.0464 | ---   | 0.0913 | 0.0435 | 0.0436 | 0.0460 | 0.0707 | 0.1813 | 0.1839 | 0.0426  |
| $s_{\text{H}}^{\text{I+II}}$ | 0.0749 | 0.0357 | 0.0044 | 0.0040 | ---   | 0.0087 | 0.0048 | 0.0046 | 0.0047 | 0.0062 | 0.0066 | 0.0061 | 0.0046  |
| $S$                          | 0.3013 | 0.1112 | 0.0531 | 0.0545 | ---   | 0.1088 | 0.0530 | 0.0529 | 0.0552 | 0.0832 | 0.1945 | 0.1961 | 0.0518  |
| $T$                          | 1.0504 | 0.7489 | 0.5975 | 0.6038 | ---   | 1.0727 | 0.6197 | 0.6089 | 0.6573 | 0.9088 | 1.2519 | 1.2583 | 0.5918  |

### S3.7 $\text{H}_3\text{O}^+$

Table S37: The info of molecule  $\text{H}_3\text{O}^+$ .

| Prop.                        | LISA1   | LISA2   | LISA3 | LISA4   | LISA5 | LISA6   | NLIS1   | NLIS2   | NLIS3   | NLIS4   | MBIS    | GMBIS   | ISA     |
|------------------------------|---------|---------|-------|---------|-------|---------|---------|---------|---------|---------|---------|---------|---------|
| $q_{\text{O}}$               | -0.6931 | -0.6920 | ---   | -0.7133 | ---   | -0.6333 | -0.7121 | -0.7161 | -0.7168 | -0.7854 | -0.7854 | -0.7813 | -0.7185 |
| $q_{\text{H}}$               | 0.5644  | 0.5641  | ---   | 0.5712  | ---   | 0.5444  | 0.5707  | 0.5720  | 0.5723  | 0.5951  | 0.5951  | 0.5938  | 0.5728  |
| $s_{\text{O}}^{\text{I}}$    | 0.0278  | 0.0278  | ---   | 0.0274  | ---   | 0.0248  | 0.0269  | 0.0271  | 0.0276  | 0.0305  | 0.0305  | 0.0298  | 0.0272  |
| $s_{\text{H}}^{\text{I}}$    | 0.0051  | 0.0051  | ---   | 0.0049  | ---   | 0.0081  | 0.0049  | 0.0048  | 0.0047  | 0.0047  | 0.0047  | 0.0048  | 0.0047  |
| $s_{\text{O}}^{\text{II}}$   | 0.0050  | 0.0048  | ---   | 0.0005  | ---   | 0.0972  | 0.0003  | 0.0021  | 0.0012  | 0.0362  | 0.0362  | 0.0293  | 0.0000  |
| $s_{\text{H}}^{\text{II}}$   | 0.0002  | 0.0002  | ---   | 0.0002  | ---   | 0.0041  | 0.0000  | 0.0000  | 0.0000  | 0.0010  | 0.0010  | 0.0007  | -0.0000 |
| $s_{\text{O}}^{\text{I+II}}$ | 0.0328  | 0.0326  | ---   | 0.0280  | ---   | 0.1220  | 0.0272  | 0.0292  | 0.0288  | 0.0667  | 0.0667  | 0.0591  | 0.0272  |
| $s_{\text{H}}^{\text{I+II}}$ | 0.0053  | 0.0053  | ---   | 0.0051  | ---   | 0.0122  | 0.0049  | 0.0048  | 0.0047  | 0.0057  | 0.0057  | 0.0055  | 0.0047  |
| $S$                          | 0.0488  | 0.0487  | ---   | 0.0432  | ---   | 0.1587  | 0.0419  | 0.0435  | 0.0429  | 0.0838  | 0.0838  | 0.0756  | 0.0412  |
| $T$                          | 0.6671  | 0.6671  | ---   | 0.6361  | ---   | 1.3446  | 0.6391  | 0.6835  | 0.6402  | 1.0034  | 1.0034  | 0.9277  | 0.6282  |

### S3.8 $\text{H}_2\text{O}$

Table S38: The info of molecule H<sub>2</sub>O.

| Prop.        | LISA1   | LISA2   | LISA3   | LISA4   | LISA5 | LISA6   | NLIS1   | NLIS2   | NLIS3   | NLIS4   | MBIS    | GMBIS   | ISA     |
|--------------|---------|---------|---------|---------|-------|---------|---------|---------|---------|---------|---------|---------|---------|
| $q_O$        | -0.8235 | -0.8264 | -0.8280 | -0.8278 | —     | -0.7780 | -0.8296 | -0.8282 | -0.8273 | -0.8428 | -0.8581 | -0.8600 | -0.8294 |
| $q_H$        | 0.4118  | 0.4133  | 0.4141  | 0.4140  | —     | 0.3889  | 0.4148  | 0.4141  | 0.4136  | 0.4213  | 0.4290  | 0.4299  | 0.4147  |
| $s_O^I$      | 0.0223  | 0.0224  | 0.0220  | 0.0220  | —     | 0.0204  | 0.0218  | 0.0217  | 0.0217  | 0.0229  | 0.0243  | 0.0243  | 0.0218  |
| $s_H^I$      | 0.0049  | 0.0049  | 0.0046  | 0.0046  | —     | 0.0074  | 0.0045  | 0.0047  | 0.0047  | 0.0053  | 0.0047  | 0.0047  | 0.0045  |
| $s_O^{II}$   | 0.0049  | 0.0032  | 0.0002  | 0.0004  | —     | 0.0756  | 0.0021  | 0.0005  | 0.0024  | 0.0231  | 0.0290  | 0.0249  | 0.0000  |
| $s_H^{II}$   | 0.0004  | 0.0002  | 0.0001  | 0.0002  | —     | 0.0033  | 0.0000  | 0.0000  | 0.0000  | 0.0004  | 0.0009  | 0.0009  | -0.0000 |
| $s_O^{I+II}$ | 0.0273  | 0.0256  | 0.0222  | 0.0223  | —     | 0.0960  | 0.0239  | 0.0223  | 0.0241  | 0.0460  | 0.0533  | 0.0493  | 0.0218  |
| $s_H^{I+II}$ | 0.0053  | 0.0051  | 0.0047  | 0.0048  | —     | 0.0107  | 0.0045  | 0.0047  | 0.0047  | 0.0056  | 0.0056  | 0.0056  | 0.0045  |
| $S$          | 0.0379  | 0.0358  | 0.0317  | 0.0318  | —     | 0.1174  | 0.0329  | 0.0317  | 0.0335  | 0.0573  | 0.0645  | 0.0605  | 0.0308  |
| $T$          | 0.5772  | 0.5746  | 0.5510  | 0.5510  | —     | 1.1509  | 0.5954  | 0.5504  | 0.5960  | 0.8243  | 0.8411  | 0.7780  | 0.5411  |

### S3.9 OH<sup>-</sup>

Table S39: The info of molecule OH<sup>-</sup>.

| Prop.        | LISA1   | LISA2   | LISA3   | LISA4   | LISA5   | LISA6   | NLIS1   | NLIS2   | NLIS3   | NLIS4   | MBIS    | GMBIS   | ISA     |
|--------------|---------|---------|---------|---------|---------|---------|---------|---------|---------|---------|---------|---------|---------|
| $q_O$        | -1.2503 | -1.1866 | -1.2864 | -1.2887 | -1.2913 | -1.2921 | -1.2919 | -1.2909 | -1.2906 | -1.2948 | -1.1075 | -1.1081 | -1.2912 |
| $q_H$        | 0.2503  | 0.1867  | 0.2865  | 0.2887  | 0.2913  | 0.2922  | 0.2919  | 0.2909  | 0.2906  | 0.2948  | 0.1076  | 0.1082  | 0.2912  |
| $s_O^I$      | 0.0248  | 0.0181  | 0.0199  | 0.0196  | 0.0189  | 0.0201  | 0.0194  | 0.0193  | 0.0194  | 0.0200  | 0.0564  | 0.0611  | 0.0193  |
| $s_H^I$      | 0.0063  | 0.0190  | 0.0031  | 0.0030  | 0.0045  | 0.0034  | 0.0027  | 0.0029  | 0.0028  | 0.0030  | 0.0273  | 0.0287  | 0.0027  |
| $s_O^{II}$   | 0.0541  | 0.0073  | 0.0036  | 0.0057  | 0.0359  | 0.0373  | 0.0022  | 0.0019  | 0.0032  | 0.0239  | 0.0554  | 0.0513  | 0.0000  |
| $s_H^{II}$   | 0.0116  | 0.0028  | 0.0005  | 0.0005  | 0.0002  | 0.0015  | 0.0000  | 0.0000  | 0.0002  | 0.0003  | 0.0440  | 0.0476  | -0.0000 |
| $s_O^{I+II}$ | 0.0789  | 0.0253  | 0.0235  | 0.0253  | 0.0548  | 0.0573  | 0.0215  | 0.0212  | 0.0227  | 0.0439  | 0.1119  | 0.1124  | 0.0193  |
| $s_H^{I+II}$ | 0.0180  | 0.0218  | 0.0036  | 0.0035  | 0.0047  | 0.0049  | 0.0027  | 0.0029  | 0.0030  | 0.0033  | 0.0713  | 0.0763  | 0.0027  |
| $S$          | 0.0969  | 0.0471  | 0.0272  | 0.0288  | 0.0595  | 0.0622  | 0.0243  | 0.0241  | 0.0256  | 0.0473  | 0.1832  | 0.1887  | 0.0220  |
| $T$          | 0.5650  | 0.4680  | 0.4036  | 0.4126  | 0.8142  | 0.8395  | 0.4407  | 0.4137  | 0.4458  | 0.7214  | 1.1868  | 1.1553  | 0.3822  |

### S3.10 CS<sub>2</sub>

Table S40: The info of molecule CS<sub>2</sub>.

| Prop.        | LISA1   | LISA2   | LISA3 | LISA4   | LISA5 | LISA6   | NLIS1   | NLIS2   | NLIS3   | NLIS4   | MBIS    | GMBIS   | ISA     |
|--------------|---------|---------|-------|---------|-------|---------|---------|---------|---------|---------|---------|---------|---------|
| $q_C$        | 0.0725  | 0.0725  | ---   | 0.0832  | ---   | -0.0077 | 0.0853  | 0.0588  | 0.0588  | -0.0436 | -0.0436 | -0.0173 | 0.0820  |
| $q_S$        | -0.0365 | -0.0365 | ---   | -0.0417 | ---   | 0.0040  | -0.0427 | -0.0295 | -0.0295 | 0.0219  | 0.0219  | 0.0091  | -0.0410 |
| $s_C^I$      | 0.0192  | 0.0192  | ---   | 0.0196  | ---   | 0.0420  | 0.0188  | 0.0206  | 0.0206  | 0.0400  | 0.0400  | 0.0334  | 0.0177  |
| $s_S^I$      | 0.0120  | 0.0120  | ---   | 0.0112  | ---   | 0.0132  | 0.0113  | 0.0120  | 0.0120  | 0.0114  | 0.0114  | 0.0114  | 0.0113  |
| $s_C^{II}$   | 0.0016  | 0.0016  | ---   | 0.0008  | ---   | 0.0372  | 0.0003  | 0.0010  | 0.0010  | 0.0339  | 0.0339  | 0.0271  | 0.0000  |
| $s_S^{II}$   | 0.0080  | 0.0080  | ---   | 0.0064  | ---   | 0.2310  | 0.0050  | 0.0100  | 0.0100  | 0.2164  | 0.2164  | 0.0658  | -0.0000 |
| $s_C^{I+II}$ | 0.0208  | 0.0208  | ---   | 0.0203  | ---   | 0.0792  | 0.0190  | 0.0216  | 0.0216  | 0.0739  | 0.0739  | 0.0605  | 0.0177  |
| $s_S^{I+II}$ | 0.0199  | 0.0199  | ---   | 0.0176  | ---   | 0.2442  | 0.0163  | 0.0220  | 0.0220  | 0.2278  | 0.2278  | 0.0772  | 0.0113  |
| $S$          | 0.0607  | 0.0607  | ---   | 0.0555  | ---   | 0.5676  | 0.0517  | 0.0656  | 0.0656  | 0.5295  | 0.5295  | 0.2149  | 0.0403  |
| $T$          | 1.1990  | 1.1990  | ---   | 1.2326  | ---   | 5.3416  | 1.1368  | 1.2892  | 1.2892  | 5.2280  | 5.2280  | 2.5295  | 0.8815  |

### S3.11 CCl<sub>4</sub>

Table S41: The info of molecule CCl<sub>4</sub>.

| Prop.           | LISA1   | LISA2   | LISA3 | LISA4   | LISA5 | LISA6   | NLIS1   | NLIS2   | NLIS3   | NLIS4   | MBIS    | GMBIS   | ISA     |
|-----------------|---------|---------|-------|---------|-------|---------|---------|---------|---------|---------|---------|---------|---------|
| $q_C$           | 0.4484  | 0.4484  | ---   | 0.1895  | ---   | 0.2607  | 0.1771  | 0.3250  | 0.3231  | 0.1399  | 0.1399  | 0.1803  | 0.1357  |
| $q_{Cl}$        | -0.1119 | -0.1119 | ---   | -0.0472 | ---   | -0.0658 | -0.0441 | -0.0811 | -0.0806 | -0.0354 | -0.0354 | -0.0452 | -0.0340 |
| $s_C^I$         | 0.0070  | 0.0070  | ---   | 0.0080  | ---   | 0.0243  | 0.0095  | 0.0079  | 0.0079  | 0.0272  | 0.0272  | 0.0218  | 0.0100  |
| $s_{Cl}^I$      | 0.0223  | 0.0223  | ---   | 0.0205  | ---   | 0.0285  | 0.0195  | 0.0222  | 0.0223  | 0.0273  | 0.0273  | 0.0257  | 0.0187  |
| $s_C^{II}$      | 0.0032  | 0.0032  | ---   | 0.0024  | ---   | 0.0319  | 0.0015  | 0.0017  | 0.0018  | 0.0238  | 0.0238  | 0.0201  | 0.0000  |
| $s_{Cl}^{II}$   | 0.0054  | 0.0054  | ---   | 0.0034  | ---   | 0.2401  | 0.0030  | 0.0073  | 0.0062  | 0.2271  | 0.2271  | 0.0715  | -0.0000 |
| $s_C^{I+II}$    | 0.0102  | 0.0102  | ---   | 0.0104  | ---   | 0.0562  | 0.0110  | 0.0097  | 0.0097  | 0.0510  | 0.0510  | 0.0419  | 0.0100  |
| $s_{Cl}^{I+II}$ | 0.0277  | 0.0277  | ---   | 0.0238  | ---   | 0.2686  | 0.0225  | 0.0296  | 0.0284  | 0.2544  | 0.2544  | 0.0972  | 0.0187  |
| $S$             | 0.1209  | 0.1209  | ---   | 0.1058  | ---   | 1.1306  | 0.1010  | 0.1279  | 0.1234  | 1.0687  | 1.0687  | 0.4307  | 0.0849  |
| $T$             | 2.4008  | 2.4008  | ---   | 2.4038  | ---   | 10.6275 | 2.2912  | 2.5363  | 2.2573  | 10.4201 | 10.4201 | 5.0401  | 1.8205  |

### S3.12 B<sub>8</sub>



Table S42: The info of molecule B<sub>8</sub>.

| Prop.           | LISA1   | LISA2   | LISA3 | LISA4   | LISA5 | LISA6   | NLIS1   | NLIS2   | NLIS3   | NLIS4   | MBIS    | GMBIS   | ISA     |
|-----------------|---------|---------|-------|---------|-------|---------|---------|---------|---------|---------|---------|---------|---------|
| $q_{B1}$        | 0.4110  | 0.4110  | ---   | 0.3605  | ---   | 0.0773  | 0.3671  | 0.3693  | 0.3693  | 0.1124  | 0.1129  | 0.1177  | 0.4074  |
| $q_{B2}$        | 0.1557  | 0.1557  | ---   | 0.1672  | ---   | 0.2125  | 0.1646  | 0.1650  | 0.1650  | 0.1839  | 0.1843  | 0.1838  | 0.1617  |
| $q_{B3}$        | -0.1116 | -0.1116 | ---   | -0.1062 | ---   | -0.0676 | -0.1054 | -0.1073 | -0.1073 | -0.0670 | -0.0672 | -0.0679 | -0.1135 |
| $q_{B4}$        | -0.2391 | -0.2391 | ---   | -0.2336 | ---   | -0.1981 | -0.2355 | -0.2336 | -0.2336 | -0.1827 | -0.1831 | -0.1842 | -0.2409 |
| $q_{B5}$        | 0.0673  | 0.0673  | ---   | 0.0761  | ---   | 0.1191  | 0.0754  | 0.0740  | 0.0740  | 0.0997  | 0.0999  | 0.0993  | 0.0700  |
| $s_{B1}^I$      | 0.0216  | 0.0216  | ---   | 0.0222  | ---   | 0.0491  | 0.0216  | 0.0218  | 0.0218  | 0.0468  | 0.0468  | 0.0459  | 0.0207  |
| $s_{B2}^I$      | 0.0709  | 0.0709  | ---   | 0.0701  | ---   | 0.0807  | 0.0696  | 0.0702  | 0.0702  | 0.0809  | 0.0808  | 0.0805  | 0.0692  |
| $s_{B3}^I$      | 0.0524  | 0.0524  | ---   | 0.0524  | ---   | 0.0625  | 0.0522  | 0.0527  | 0.0527  | 0.0615  | 0.0616  | 0.0613  | 0.0521  |
| $s_{B4}^I$      | 0.0499  | 0.0499  | ---   | 0.0502  | ---   | 0.0598  | 0.0501  | 0.0505  | 0.0505  | 0.0579  | 0.0580  | 0.0577  | 0.0500  |
| $s_{B5}^I$      | 0.0624  | 0.0624  | ---   | 0.0618  | ---   | 0.0722  | 0.0615  | 0.0621  | 0.0621  | 0.0722  | 0.0722  | 0.0719  | 0.0612  |
| $s_{B1}^{II}$   | 0.0025  | 0.0025  | ---   | 0.0012  | ---   | 0.0337  | 0.0007  | 0.0006  | 0.0006  | 0.0308  | 0.0308  | 0.0281  | 0.0000  |
| $s_{B2}^{II}$   | 0.0013  | 0.0013  | ---   | 0.0011  | ---   | 0.0427  | 0.0007  | 0.0013  | 0.0013  | 0.0381  | 0.0381  | 0.0348  | -0.0000 |
| $s_{B3}^{II}$   | 0.0019  | 0.0019  | ---   | 0.0011  | ---   | 0.0441  | 0.0006  | 0.0014  | 0.0014  | 0.0399  | 0.0399  | 0.0365  | -0.0000 |
| $s_{B4}^{II}$   | 0.0023  | 0.0023  | ---   | 0.0010  | ---   | 0.0439  | 0.0006  | 0.0014  | 0.0014  | 0.0403  | 0.0403  | 0.0370  | -0.0000 |
| $s_{B5}^{II}$   | 0.0015  | 0.0015  | ---   | 0.0011  | ---   | 0.0433  | 0.0007  | 0.0014  | 0.0014  | 0.0387  | 0.0387  | 0.0354  | -0.0000 |
| $s_{B1}^{I+II}$ | 0.0241  | 0.0241  | ---   | 0.0234  | ---   | 0.0828  | 0.0223  | 0.0224  | 0.0224  | 0.0776  | 0.0776  | 0.0741  | 0.0207  |
| $s_{B2}^{I+II}$ | 0.0722  | 0.0722  | ---   | 0.0712  | ---   | 0.1234  | 0.0703  | 0.0716  | 0.0716  | 0.1190  | 0.1189  | 0.1153  | 0.0692  |
| $s_{B3}^{I+II}$ | 0.0543  | 0.0543  | ---   | 0.0534  | ---   | 0.1065  | 0.0528  | 0.0541  | 0.0541  | 0.1014  | 0.1015  | 0.0978  | 0.0521  |
| $s_{B4}^{I+II}$ | 0.0521  | 0.0521  | ---   | 0.0512  | ---   | 0.1037  | 0.0507  | 0.0519  | 0.0519  | 0.0982  | 0.0983  | 0.0947  | 0.0500  |
| $s_{B5}^{I+II}$ | 0.0638  | 0.0638  | ---   | 0.0629  | ---   | 0.1155  | 0.0621  | 0.0634  | 0.0634  | 0.1109  | 0.1109  | 0.1072  | 0.0612  |
| $S$             | 0.4368  | 0.4368  | ---   | 0.4297  | ---   | 0.8577  | 0.4239  | 0.4330  | 0.4330  | 0.8177  | 0.8179  | 0.7889  | 0.4164  |
| $T$             | 3.9614  | 3.9614  | ---   | 3.8811  | ---   | 6.0854  | 3.9164  | 3.9600  | 3.9600  | 6.0359  | 6.0358  | 5.7869  | 3.7466  |

### S3.13 B<sub>8</sub> triplet

Table S43: The info of molecule B<sub>8</sub> triplet.

| Prop.    | LISA1   | LISA2   | LISA3 | LISA4   | LISA5 | LISA6   | NLIS1   | NLIS2   | NLIS3   | NLIS4   | MBIS    | GMBIS   | ISA     |
|----------|---------|---------|-------|---------|-------|---------|---------|---------|---------|---------|---------|---------|---------|
| $q_{B1}$ | 0.3868  | 0.3868  | ---   | 0.3428  | ---   | 0.0530  | 0.3421  | 0.3536  | 0.3536  | 0.0983  | 0.0983  | 0.1030  | 0.3920  |
| $q_{B2}$ | -0.0559 | -0.0559 | ---   | -0.0495 | ---   | -0.0072 | -0.0491 | -0.0509 | -0.0509 | -0.0137 | -0.0137 | -0.0145 | -0.0562 |
| $q_{B3}$ | -0.0548 | -0.0548 | ---   | -0.0486 | ---   | -0.0078 | -0.0486 | -0.0502 | -0.0502 | -0.0145 | -0.0145 | -0.0151 | -0.0559 |
| $q_{B4}$ | -0.0552 | -0.0552 | ---   | -0.0488 | ---   | -0.0091 | -0.0486 | -0.0503 | -0.0503 | -0.0155 | -0.0155 | -0.0162 | -0.0559 |

Continued on next page

Table S43: The info of molecule B<sub>8</sub> triplet.

| Prop.           | LISA1   | LISA2   | LISA3 | LISA4   | LISA5 | LISA6   | NLIS1   | NLIS2   | NLIS3   | NLIS4   | MBIS    | GMBIS   | ISA     |
|-----------------|---------|---------|-------|---------|-------|---------|---------|---------|---------|---------|---------|---------|---------|
| $q_{B5}$        | -0.0555 | -0.0555 | ---   | -0.0491 | ---   | -0.0075 | -0.0489 | -0.0508 | -0.0508 | -0.0141 | -0.0141 | -0.0149 | -0.0561 |
| $s_{B1}^I$      | 0.0204  | 0.0204  | ---   | 0.0210  | ---   | 0.0470  | 0.0205  | 0.0207  | 0.0207  | 0.0441  | 0.0441  | 0.0433  | 0.0195  |
| $s_{B2}^I$      | 0.0518  | 0.0518  | ---   | 0.0516  | ---   | 0.0619  | 0.0514  | 0.0519  | 0.0519  | 0.0611  | 0.0611  | 0.0607  | 0.0512  |
| $s_{B3}^I$      | 0.0518  | 0.0518  | ---   | 0.0516  | ---   | 0.0619  | 0.0514  | 0.0519  | 0.0519  | 0.0611  | 0.0611  | 0.0608  | 0.0512  |
| $s_{B4}^I$      | 0.0518  | 0.0518  | ---   | 0.0517  | ---   | 0.0620  | 0.0514  | 0.0520  | 0.0520  | 0.0611  | 0.0611  | 0.0609  | 0.0512  |
| $s_{B5}^I$      | 0.0518  | 0.0518  | ---   | 0.0516  | ---   | 0.0618  | 0.0514  | 0.0519  | 0.0519  | 0.0610  | 0.0610  | 0.0607  | 0.0512  |
| $s_{B1}^{II}$   | 0.0024  | 0.0024  | ---   | 0.0011  | ---   | 0.0335  | 0.0008  | 0.0005  | 0.0005  | 0.0308  | 0.0308  | 0.0281  | 0.0000  |
| $s_{B2}^{II}$   | 0.0017  | 0.0017  | ---   | 0.0011  | ---   | 0.0440  | 0.0006  | 0.0014  | 0.0014  | 0.0395  | 0.0395  | 0.0362  | -0.0000 |
| $s_{B3}^{II}$   | 0.0017  | 0.0017  | ---   | 0.0011  | ---   | 0.0440  | 0.0006  | 0.0014  | 0.0014  | 0.0395  | 0.0395  | 0.0362  | -0.0000 |
| $s_{B4}^{II}$   | 0.0017  | 0.0017  | ---   | 0.0011  | ---   | 0.0439  | 0.0006  | 0.0014  | 0.0014  | 0.0394  | 0.0394  | 0.0361  | -0.0000 |
| $s_{B5}^{II}$   | 0.0017  | 0.0017  | ---   | 0.0011  | ---   | 0.0440  | 0.0006  | 0.0014  | 0.0014  | 0.0395  | 0.0395  | 0.0362  | -0.0000 |
| $s_{B1}^{I+II}$ | 0.0228  | 0.0228  | ---   | 0.0221  | ---   | 0.0805  | 0.0213  | 0.0212  | 0.0212  | 0.0749  | 0.0749  | 0.0714  | 0.0195  |
| $s_{B2}^{I+II}$ | 0.0535  | 0.0535  | ---   | 0.0527  | ---   | 0.1059  | 0.0520  | 0.0533  | 0.0533  | 0.1006  | 0.1006  | 0.0969  | 0.0512  |
| $s_{B3}^{I+II}$ | 0.0535  | 0.0535  | ---   | 0.0527  | ---   | 0.1059  | 0.0520  | 0.0533  | 0.0533  | 0.1006  | 0.1006  | 0.0970  | 0.0512  |
| $s_{B4}^{I+II}$ | 0.0536  | 0.0536  | ---   | 0.0527  | ---   | 0.1059  | 0.0520  | 0.0534  | 0.0534  | 0.1006  | 0.1006  | 0.0970  | 0.0512  |
| $s_{B5}^{I+II}$ | 0.0535  | 0.0535  | ---   | 0.0527  | ---   | 0.1058  | 0.0520  | 0.0533  | 0.0533  | 0.1005  | 0.1005  | 0.0968  | 0.0512  |
| $S$             | 0.3974  | 0.3974  | ---   | 0.3910  | ---   | 0.8215  | 0.3854  | 0.3945  | 0.3945  | 0.7789  | 0.7789  | 0.7499  | 0.3780  |
| $T$             | 3.8255  | 3.8255  | ---   | 3.7647  | ---   | 6.0165  | 3.7955  | 3.8515  | 3.8515  | 5.9711  | 5.9711  | 5.7223  | 3.6098  |

### S3.14 B<sub>8</sub><sup>2-</sup>

Table S44: The info of molecule B<sub>8</sub><sup>2-</sup>.

| Prop.      | LISA1   | LISA2   | LISA3 | LISA4   | LISA5 | LISA6   | NLIS1   | NLIS2   | NLIS3   | NLIS4   | MBIS    | GMBIS   | ISA     |
|------------|---------|---------|-------|---------|-------|---------|---------|---------|---------|---------|---------|---------|---------|
| $q_{B1}$   | 0.8114  | 0.8114  | ---   | 0.8396  | ---   | 0.7284  | 0.8258  | 0.8178  | 0.8178  | 0.5966  | 0.7118  | 0.7223  | 0.7469  |
| $q_{B2}$   | -0.4029 | -0.4029 | ---   | -0.4067 | ---   | -0.3904 | -0.4043 | -0.4033 | -0.4033 | -0.3721 | -0.3874 | -0.3893 | -0.3930 |
| $q_{B3}$   | -0.4007 | -0.4007 | ---   | -0.4048 | ---   | -0.3889 | -0.4031 | -0.4018 | -0.4018 | -0.3697 | -0.3873 | -0.3886 | -0.3921 |
| $q_{B4}$   | -0.4017 | -0.4017 | ---   | -0.4056 | ---   | -0.3928 | -0.4034 | -0.4024 | -0.4024 | -0.3741 | -0.3897 | -0.3914 | -0.3924 |
| $q_{B5}$   | -0.4018 | -0.4018 | ---   | -0.4057 | ---   | -0.3893 | -0.4037 | -0.4026 | -0.4026 | -0.3704 | -0.3872 | -0.3889 | -0.3925 |
| $s_{B1}^I$ | 0.0166  | 0.0166  | ---   | 0.0148  | ---   | 0.0290  | 0.0144  | 0.0142  | 0.0142  | 0.0324  | 0.0314  | 0.0305  | 0.0186  |
| $s_{B2}^I$ | 0.0382  | 0.0382  | ---   | 0.0381  | ---   | 0.0475  | 0.0379  | 0.0383  | 0.0383  | 0.0467  | 0.0517  | 0.0515  | 0.0366  |
| $s_{B3}^I$ | 0.0381  | 0.0381  | ---   | 0.0381  | ---   | 0.0475  | 0.0379  | 0.0383  | 0.0383  | 0.0466  | 0.0518  | 0.0515  | 0.0366  |

Continued on next page

Table S44: The info of molecule  $B_8^{2-}$ .

| Prop.           | LISA1  | LISA2  | LISA3 | LISA4  | LISA5 | LISA6  | NLIS1  | NLIS2  | NLIS3  | NLIS4  | MBIS   | GMBIS  | ISA     |
|-----------------|--------|--------|-------|--------|-------|--------|--------|--------|--------|--------|--------|--------|---------|
| $s_{B4}^I$      | 0.0382 | 0.0382 | ---   | 0.0382 | ---   | 0.0476 | 0.0379 | 0.0383 | 0.0383 | 0.0467 | 0.0518 | 0.0516 | 0.0366  |
| $s_{B5}^I$      | 0.0381 | 0.0381 | ---   | 0.0381 | ---   | 0.0474 | 0.0379 | 0.0383 | 0.0383 | 0.0465 | 0.0517 | 0.0514 | 0.0366  |
| $s_{B1}^{II}$   | 0.0012 | 0.0012 | ---   | 0.0010 | ---   | 0.0225 | 0.0006 | 0.0006 | 0.0006 | 0.0186 | 0.0186 | 0.0166 | -0.0000 |
| $s_{B2}^{II}$   | 0.0019 | 0.0019 | ---   | 0.0007 | ---   | 0.0276 | 0.0005 | 0.0007 | 0.0007 | 0.0268 | 0.0322 | 0.0298 | 0.0000  |
| $s_{B3}^{II}$   | 0.0020 | 0.0020 | ---   | 0.0007 | ---   | 0.0276 | 0.0004 | 0.0007 | 0.0007 | 0.0267 | 0.0321 | 0.0298 | 0.0000  |
| $s_{B4}^{II}$   | 0.0020 | 0.0020 | ---   | 0.0007 | ---   | 0.0276 | 0.0004 | 0.0007 | 0.0007 | 0.0267 | 0.0321 | 0.0298 | 0.0000  |
| $s_{B5}^{II}$   | 0.0020 | 0.0020 | ---   | 0.0007 | ---   | 0.0276 | 0.0005 | 0.0007 | 0.0007 | 0.0267 | 0.0321 | 0.0298 | 0.0000  |
| $s_{B1}^{I+II}$ | 0.0178 | 0.0178 | ---   | 0.0157 | ---   | 0.0515 | 0.0151 | 0.0148 | 0.0148 | 0.0510 | 0.0500 | 0.0472 | 0.0186  |
| $s_{B2}^{I+II}$ | 0.0401 | 0.0401 | ---   | 0.0389 | ---   | 0.0752 | 0.0383 | 0.0390 | 0.0390 | 0.0735 | 0.0839 | 0.0813 | 0.0366  |
| $s_{B3}^{I+II}$ | 0.0401 | 0.0401 | ---   | 0.0389 | ---   | 0.0751 | 0.0383 | 0.0389 | 0.0389 | 0.0733 | 0.0839 | 0.0813 | 0.0366  |
| $s_{B4}^{I+II}$ | 0.0401 | 0.0401 | ---   | 0.0389 | ---   | 0.0752 | 0.0383 | 0.0390 | 0.0390 | 0.0734 | 0.0839 | 0.0813 | 0.0366  |
| $s_{B5}^{I+II}$ | 0.0401 | 0.0401 | ---   | 0.0389 | ---   | 0.0750 | 0.0383 | 0.0389 | 0.0389 | 0.0732 | 0.0838 | 0.0812 | 0.0366  |
| $S$             | 0.2986 | 0.2986 | ---   | 0.2879 | ---   | 0.5772 | 0.2833 | 0.2876 | 0.2876 | 0.5644 | 0.6371 | 0.6159 | 0.2748  |
| $T$             | 3.3840 | 3.3840 | ---   | 3.2935 | ---   | 5.2987 | 3.3231 | 3.3431 | 3.3431 | 5.1486 | 5.2966 | 5.0607 | 3.1150  |

### S3.15 $B_9^-$

Table S45: The info of molecule  $B_9^-$ .

| Prop.           | LISA1   | LISA2   | LISA3 | LISA4   | LISA5 | LISA6   | NLIS1   | NLIS2   | NLIS3   | NLIS4   | MBIS    | GMBIS   | ISA     |
|-----------------|---------|---------|-------|---------|-------|---------|---------|---------|---------|---------|---------|---------|---------|
| $q_{B1}$        | 0.5243  | 0.5241  | ---   | 0.5371  | ---   | 0.3605  | 0.5503  | 0.5287  | 0.5287  | 0.3793  | 0.3895  | 0.3949  | 0.4969  |
| $q_{B2}$        | -0.1970 | -0.1970 | ---   | -0.1973 | ---   | -0.1723 | -0.1982 | -0.1952 | -0.1952 | -0.1756 | -0.1736 | -0.1746 | -0.1875 |
| $q_{B3}$        | -0.1837 | -0.1837 | ---   | -0.1867 | ---   | -0.1653 | -0.1894 | -0.1868 | -0.1868 | -0.1667 | -0.1711 | -0.1714 | -0.1864 |
| $s_{B1}^I$      | 0.0153  | 0.0153  | ---   | 0.0139  | ---   | 0.0319  | 0.0135  | 0.0135  | 0.0135  | 0.0291  | 0.0291  | 0.0284  | 0.0155  |
| $s_{B2}^I$      | 0.0473  | 0.0473  | ---   | 0.0473  | ---   | 0.0574  | 0.0471  | 0.0476  | 0.0476  | 0.0564  | 0.0566  | 0.0563  | 0.0465  |
| $s_{B3}^I$      | 0.0472  | 0.0472  | ---   | 0.0473  | ---   | 0.0570  | 0.0471  | 0.0475  | 0.0475  | 0.0558  | 0.0565  | 0.0561  | 0.0465  |
| $s_{B1}^{II}$   | 0.0016  | 0.0016  | ---   | 0.0007  | ---   | 0.0197  | 0.0003  | 0.0005  | 0.0005  | 0.0178  | 0.0178  | 0.0159  | 0.0000  |
| $s_{B2}^{II}$   | 0.0018  | 0.0018  | ---   | 0.0009  | ---   | 0.0356  | 0.0005  | 0.0010  | 0.0010  | 0.0327  | 0.0328  | 0.0298  | 0.0000  |
| $s_{B3}^{II}$   | 0.0018  | 0.0018  | ---   | 0.0009  | ---   | 0.0355  | 0.0005  | 0.0010  | 0.0010  | 0.0326  | 0.0329  | 0.0299  | -0.0000 |
| $s_{B1}^{I+II}$ | 0.0169  | 0.0169  | ---   | 0.0147  | ---   | 0.0516  | 0.0138  | 0.0141  | 0.0141  | 0.0468  | 0.0469  | 0.0443  | 0.0155  |
| $s_{B2}^{I+II}$ | 0.0491  | 0.0491  | ---   | 0.0482  | ---   | 0.0930  | 0.0476  | 0.0485  | 0.0485  | 0.0891  | 0.0894  | 0.0860  | 0.0465  |
| $s_{B3}^{I+II}$ | 0.0490  | 0.0490  | ---   | 0.0482  | ---   | 0.0926  | 0.0476  | 0.0485  | 0.0485  | 0.0883  | 0.0894  | 0.0860  | 0.0465  |

Continued on next page

Table S45: The info of molecule  $B_9^-$ .

| Prop. | LISA1  | LISA2  | LISA3 | LISA4  | LISA5 | LISA6  | NLIS1  | NLIS2  | NLIS3  | NLIS4  | MBIS   | GMBIS  | ISA    |
|-------|--------|--------|-------|--------|-------|--------|--------|--------|--------|--------|--------|--------|--------|
| $S$   | 0.4091 | 0.4091 | ---   | 0.4003 | ---   | 0.7939 | 0.3948 | 0.4023 | 0.4023 | 0.7566 | 0.7622 | 0.7324 | 0.3874 |
| $T$   | 4.0940 | 4.0940 | ---   | 3.9727 | ---   | 6.3577 | 3.9920 | 4.0403 | 4.0403 | 6.2327 | 6.2388 | 5.9626 | 3.8250 |

## S4 Raidal density and entropy of selected atoms

### S4.1 $CH_3^+$

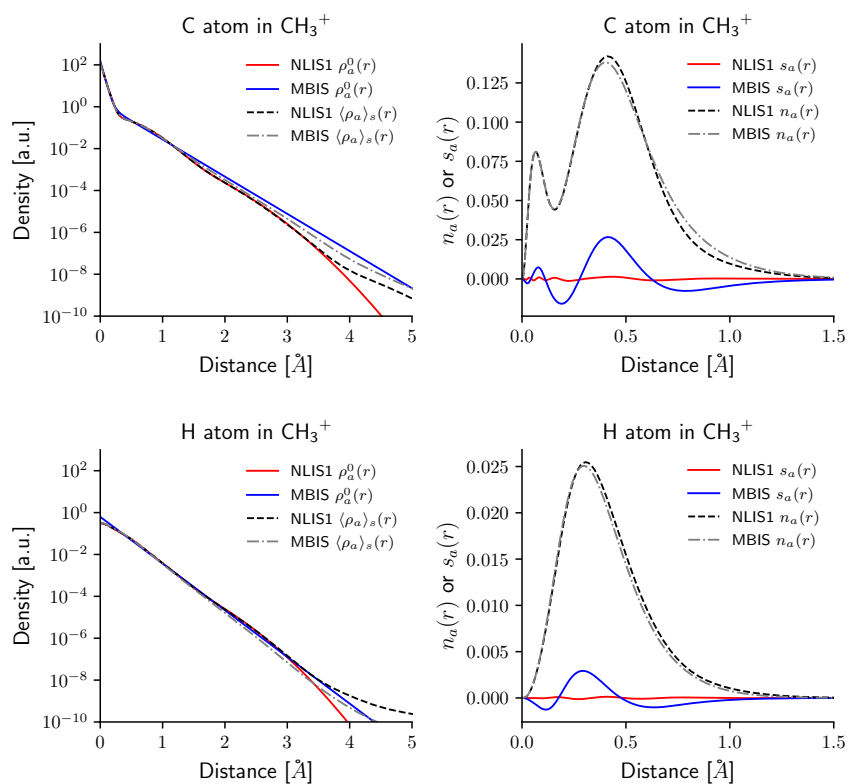

Figure S1: Comparison between the NLIS1 and MBIS methods for  $CH_3^+$ .  $\rho_a^0(r)$  and  $\langle \rho_a \rangle_s(r)$  for different atoms (left), and  $s_a(r)$  and  $n_a(r)$  for different atoms (right).

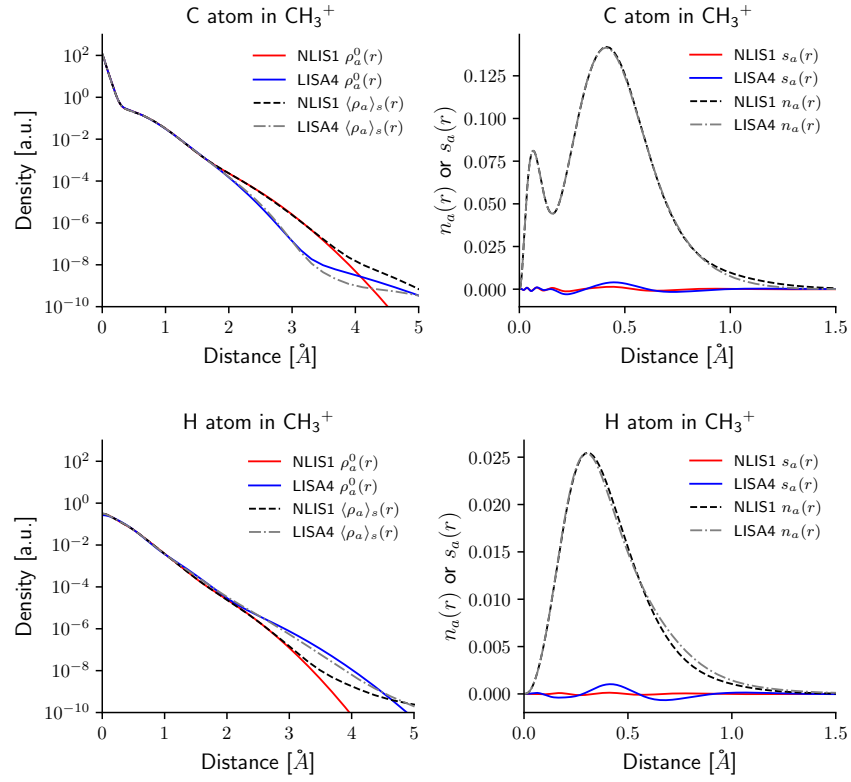

Figure S2: Comparison between the NLIS1 and LISA4 methods for  $\text{CH}_3^+$ .  $\rho_a^0(r)$  and  $\langle \rho_a \rangle_s(r)$  for different atoms (left), and  $s_a(r)$  and  $n_a(r)$  for different atoms (right).

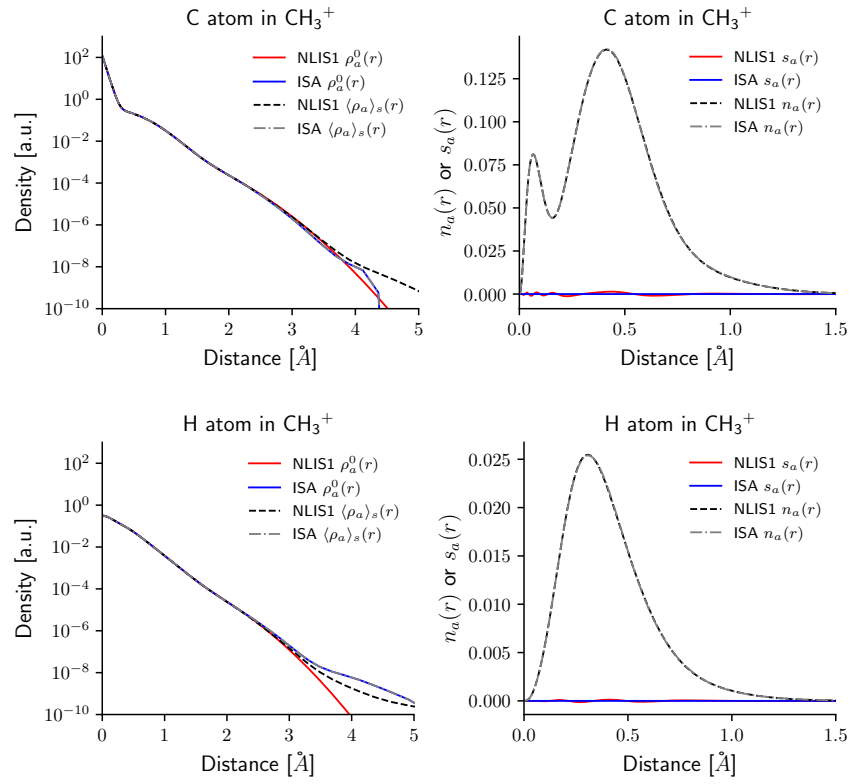

Figure S3: Comparison between the NLIS1 and ISA methods for  $\text{CH}_3^+$ .  $\rho_a^0(r)$  and  $\langle \rho_a \rangle_s(r)$  for different atoms (left), and  $s_a(r)$  and  $n_a(r)$  for different atoms (right).

## S4.2 CH<sub>4</sub>

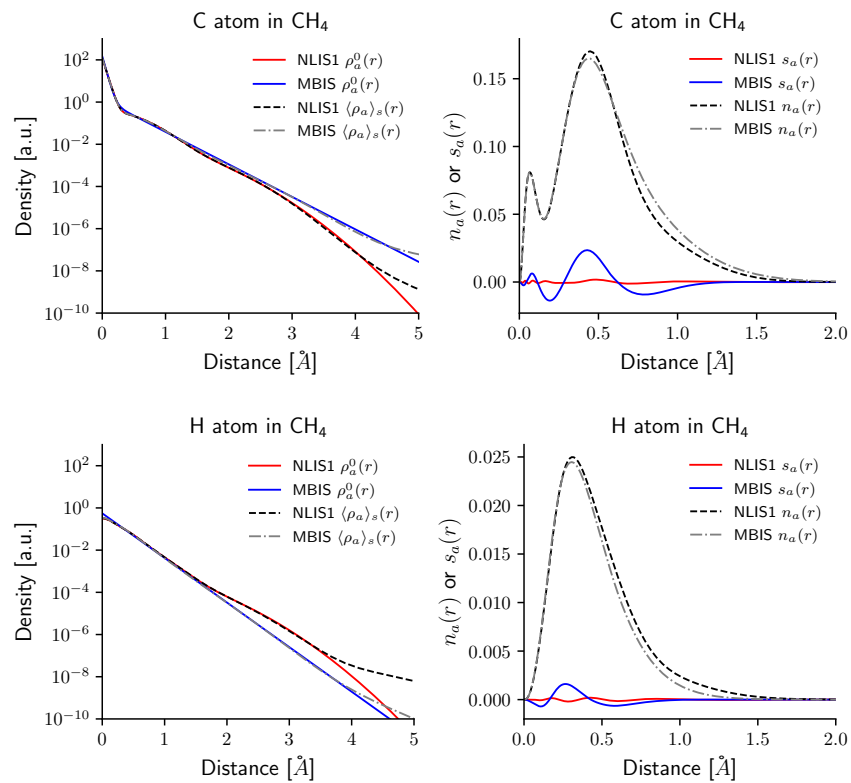

Figure S4: Comparison between the NLIS1 and MBIS methods for CH<sub>4</sub>.  $\rho_a^0(r)$  and  $\langle \rho_a \rangle_s(r)$  for different atoms (left), and  $s_a(r)$  and  $n_a(r)$  for different atoms (right).

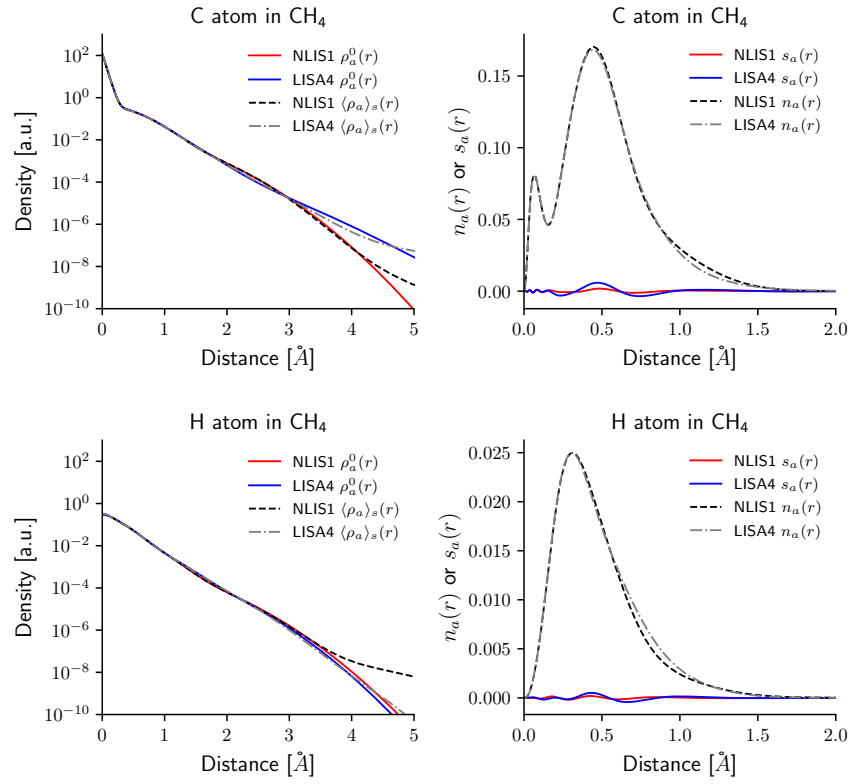

Figure S5: Comparison between the NLIS1 and LISA4 methods for CH<sub>4</sub>.  $\rho_a^0(r)$  and  $\langle \rho_a \rangle_s(r)$  for different atoms (left), and  $s_a(r)$  and  $n_a(r)$  for different atoms (right).



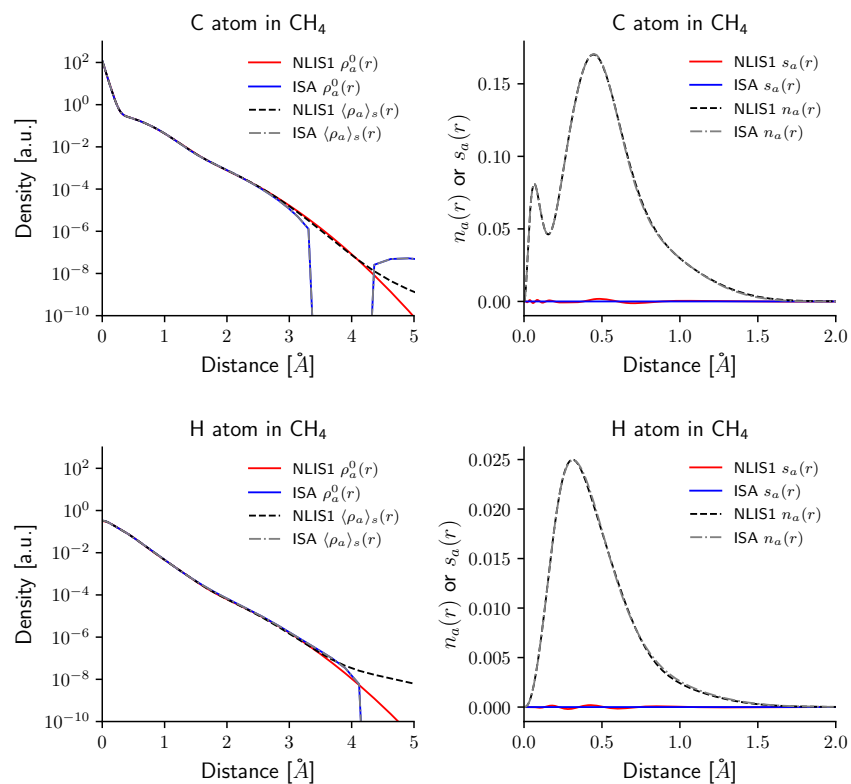

Figure S6: Comparison between the NLIS1 and ISA methods for CH<sub>4</sub>.  $\rho_a^0(r)$  and  $\langle \rho_a \rangle_s(r)$  for different atoms (left), and  $s_a(r)$  and  $n_a(r)$  for different atoms (right).

### S4.3 CH<sub>3</sub><sup>-</sup>

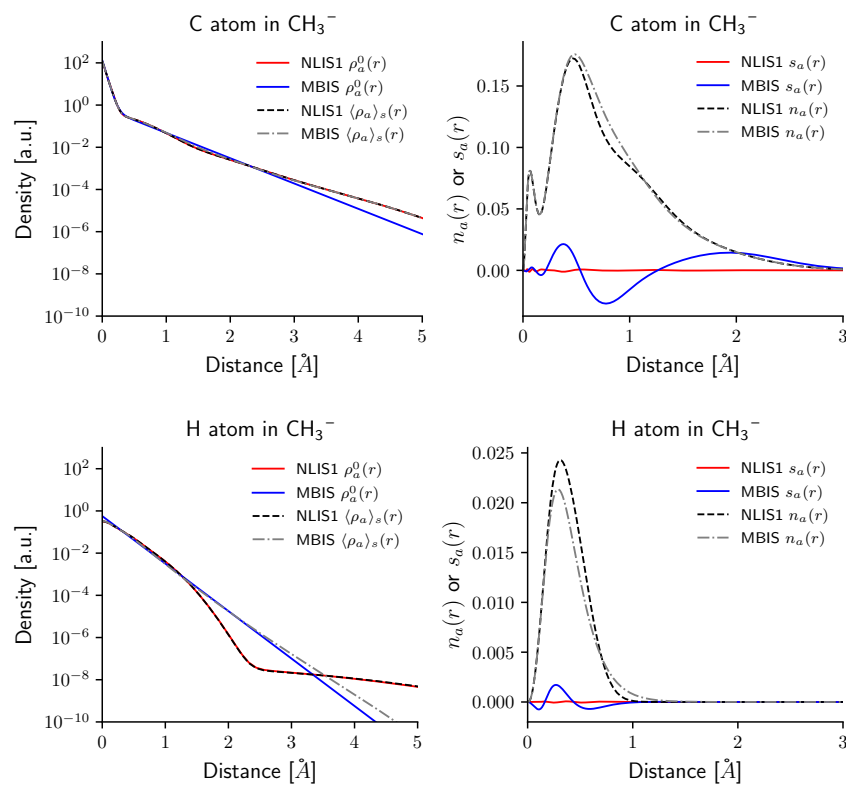

Figure S7: Comparison between the NLIS1 and MBIS methods for CH<sub>3</sub><sup>-</sup>.  $\rho_a^0(r)$  and  $\langle \rho_a \rangle_s(r)$  for different atoms (left), and  $s_a(r)$  and  $n_a(r)$  for different atoms (right).

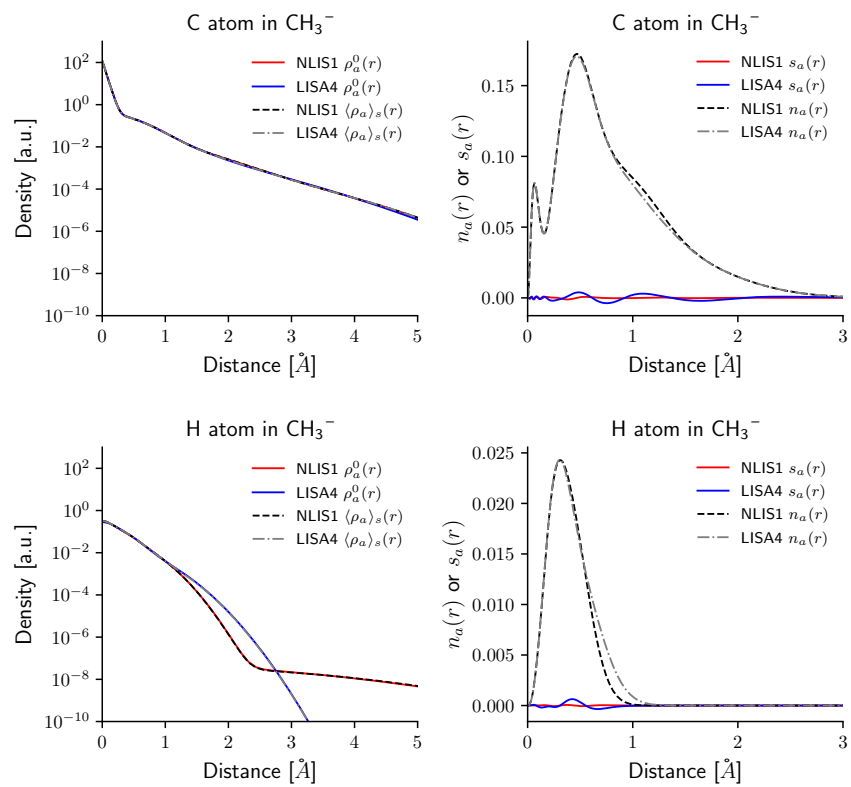

Figure S8: Comparison between the NLIS1 and LISA4 methods for  $\text{CH}_3^-$ .  $\rho_a^0(r)$  and  $\langle \rho_a \rangle_s(r)$  for different atoms (left), and  $s_a(r)$  and  $n_a(r)$  for different atoms (right).

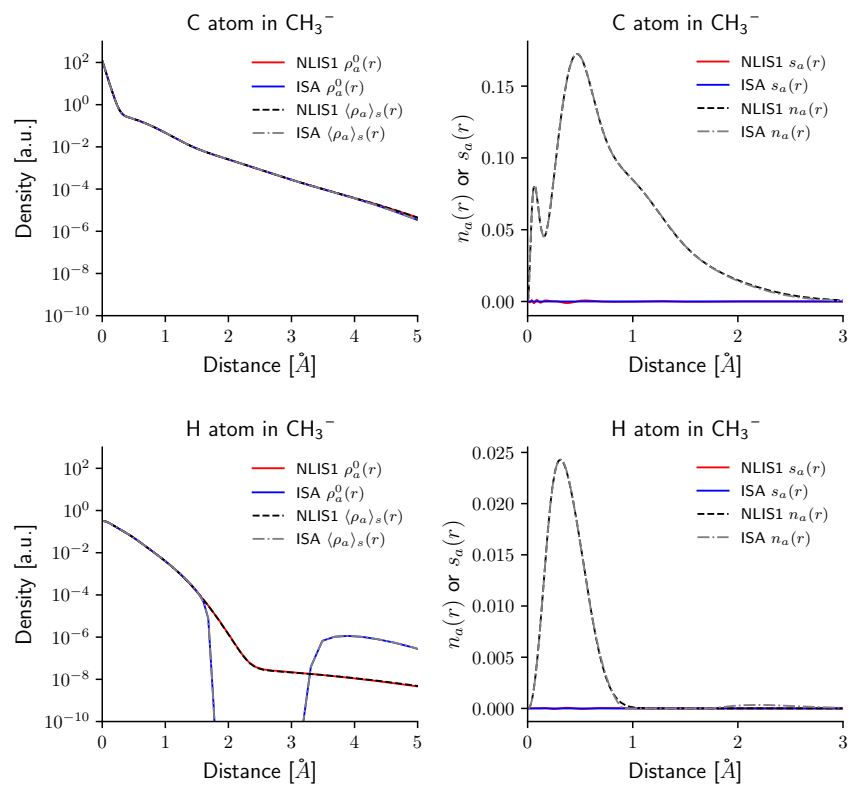

Figure S9: Comparison between the NLIS1 and ISA methods for  $\text{CH}_3^-$ .  $\rho_a^0(r)$  and  $\langle \rho_a \rangle_s(r)$  for different atoms (left), and  $s_a(r)$  and  $n_a(r)$  for different atoms (right).

## S4.4 $\text{NH}_4^+$

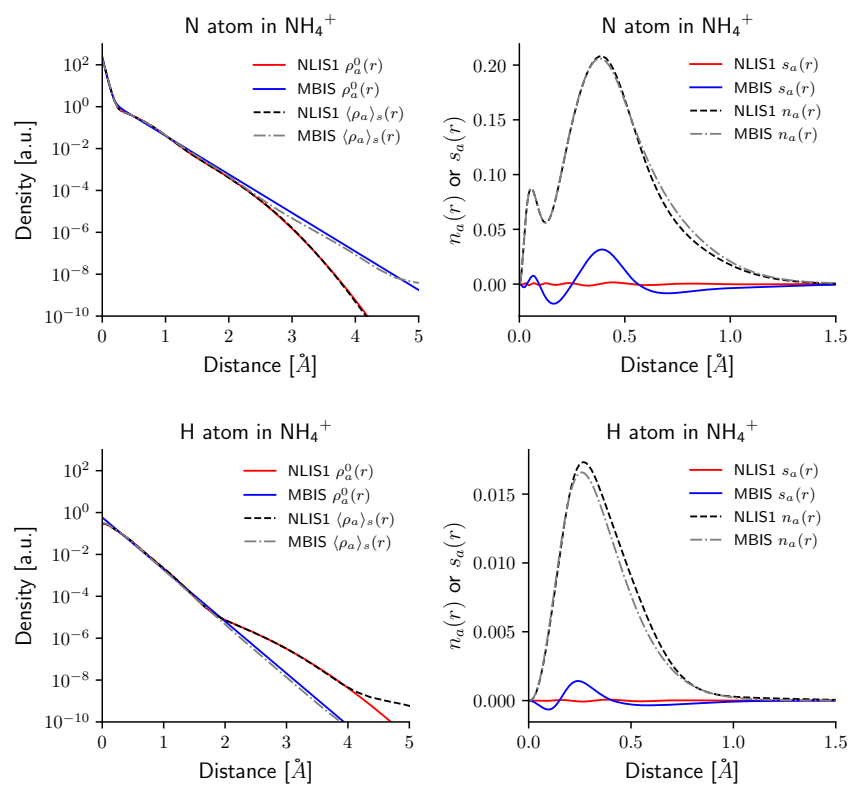

Figure S10: Comparison between the NLIS1 and MBIS methods for  $\text{NH}_4^+$ .  $\rho_a^0(r)$  and  $\langle \rho_a \rangle_s(r)$  for different atoms (left), and  $s_a(r)$  and  $n_a(r)$  for different atoms (right).

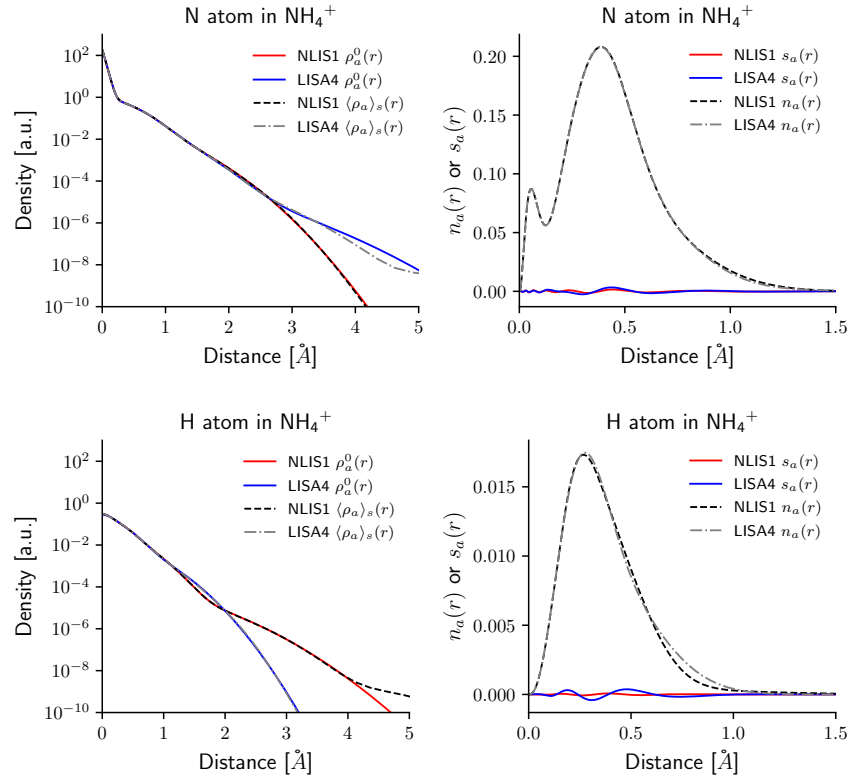

Figure S11: Comparison between the NLIS1 and LISA4 methods for  $\text{NH}_4^+$ .  $\rho_a^0(r)$  and  $\langle \rho_a \rangle_s(r)$  for different atoms (left), and  $s_a(r)$  and  $n_a(r)$  for different atoms (right).

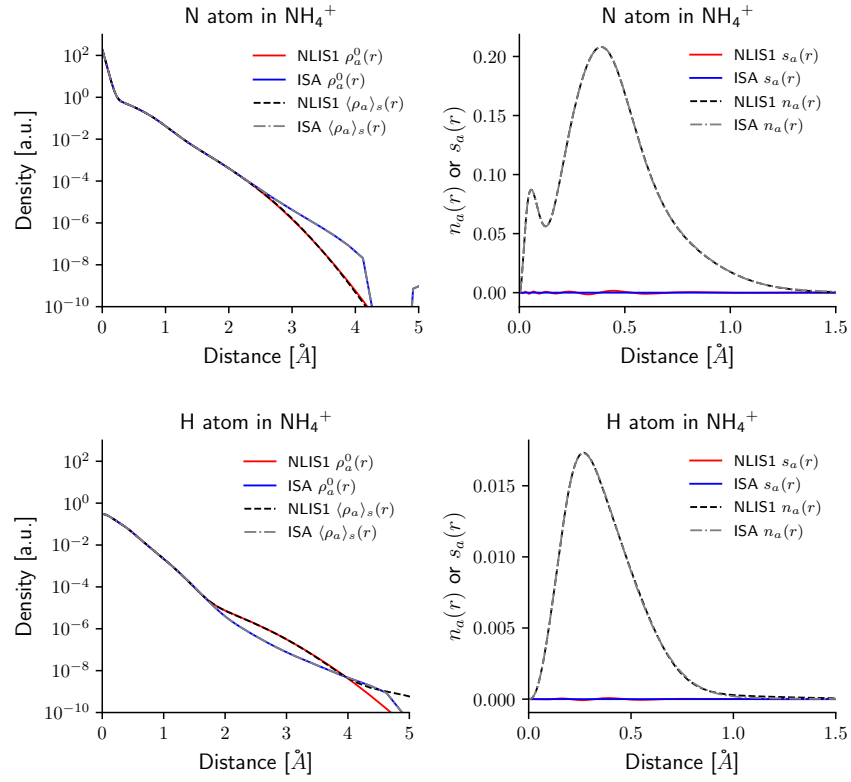

Figure S12: Comparison between the NLIS1 and ISA methods for  $\text{NH}_4^+$ .  $\rho_a^0(r)$  and  $\langle \rho_a \rangle_s(r)$  for different atoms (left), and  $s_a(r)$  and  $n_a(r)$  for different atoms (right).

## S4.5 NH<sub>3</sub>

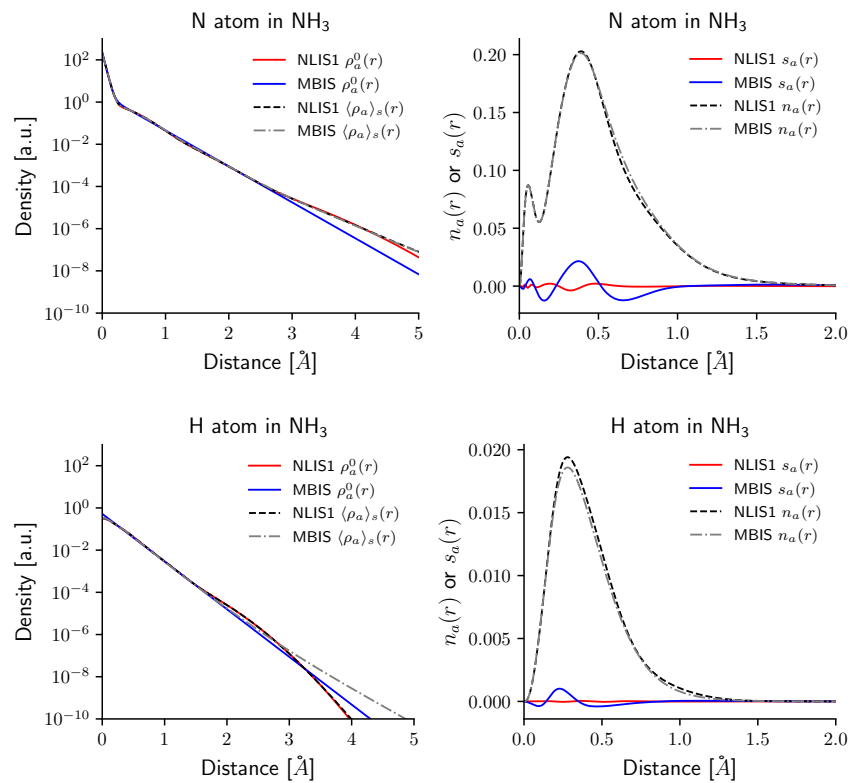

Figure S13: Comparison between the NLIS1 and MBIS methods for NH<sub>3</sub>.  $\rho_a^0(r)$  and  $\langle \rho_a \rangle_s(r)$  for different atoms (left), and  $s_a(r)$  and  $n_a(r)$  for different atoms (right).



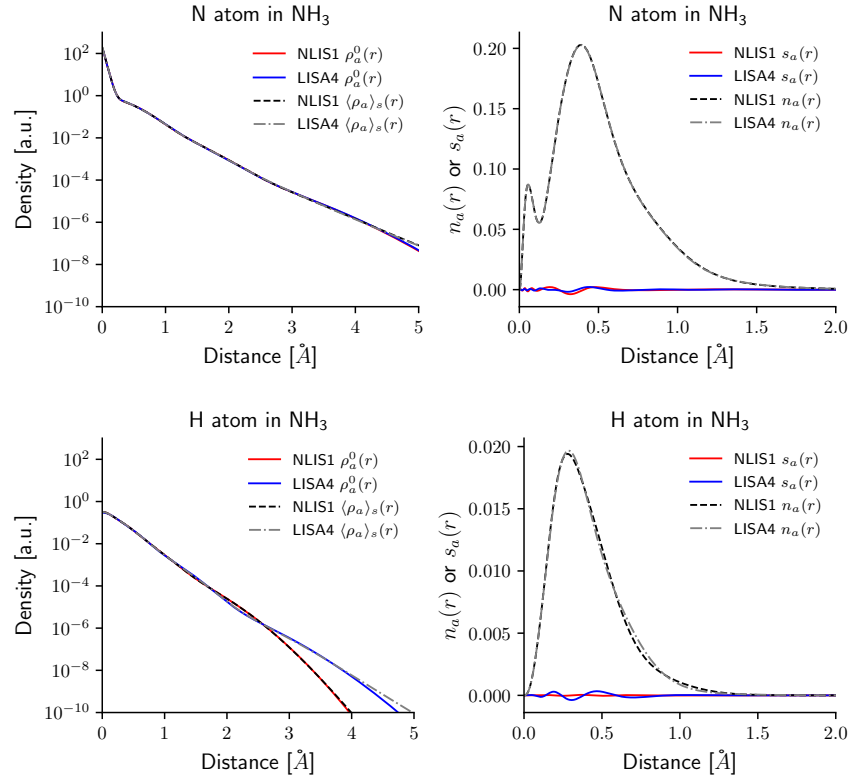

Figure S14: Comparison between the NLIS1 and LISA4 methods for NH<sub>3</sub>.  $\rho_a^0(r)$  and  $\langle \rho_a \rangle_s(r)$  for different atoms (left), and  $s_a(r)$  and  $n_a(r)$  for different atoms (right).

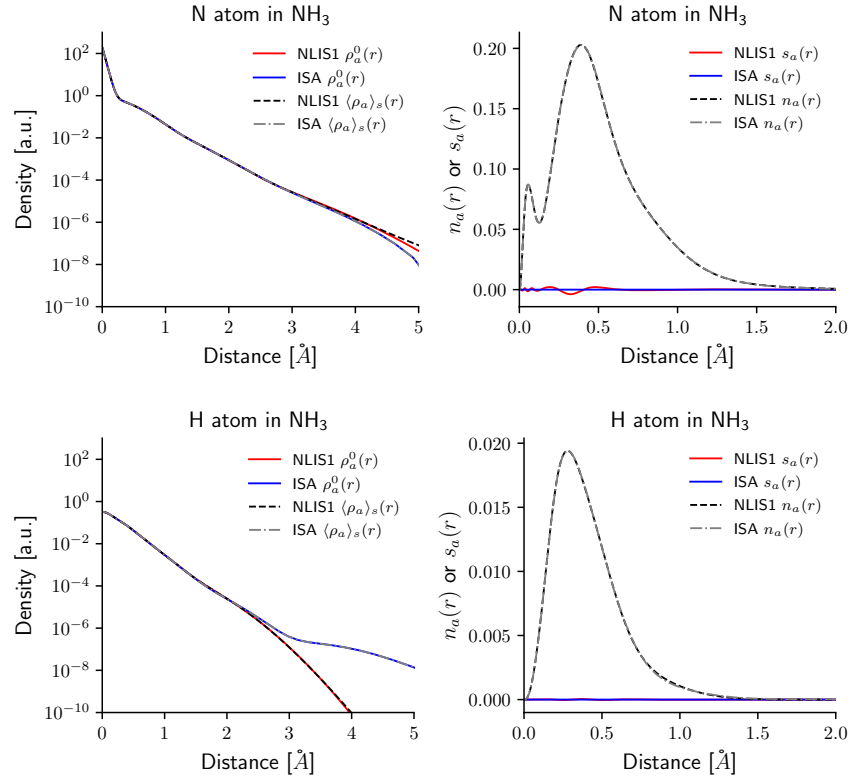

Figure S15: Comparison between the NLIS1 and ISA methods for NH<sub>3</sub>.  $\rho_a^0(r)$  and  $\langle \rho_a \rangle_s(r)$  for different atoms (left), and  $s_a(r)$  and  $n_a(r)$  for different atoms (right).

## S4.6 $\text{NH}_2^-$

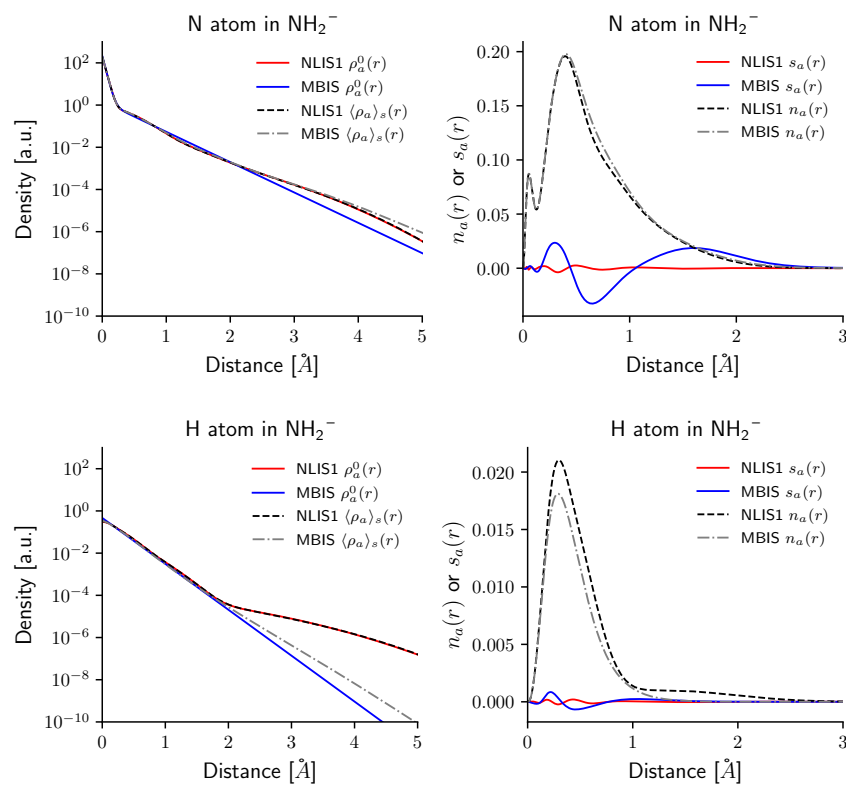

Figure S16: Comparison between the NLIS1 and MBIS methods for  $\text{NH}_2^-$ .  $\rho_a^0(r)$  and  $\langle \rho_a \rangle_s(r)$  for different atoms (left), and  $s_a(r)$  and  $n_a(r)$  for different atoms (right).

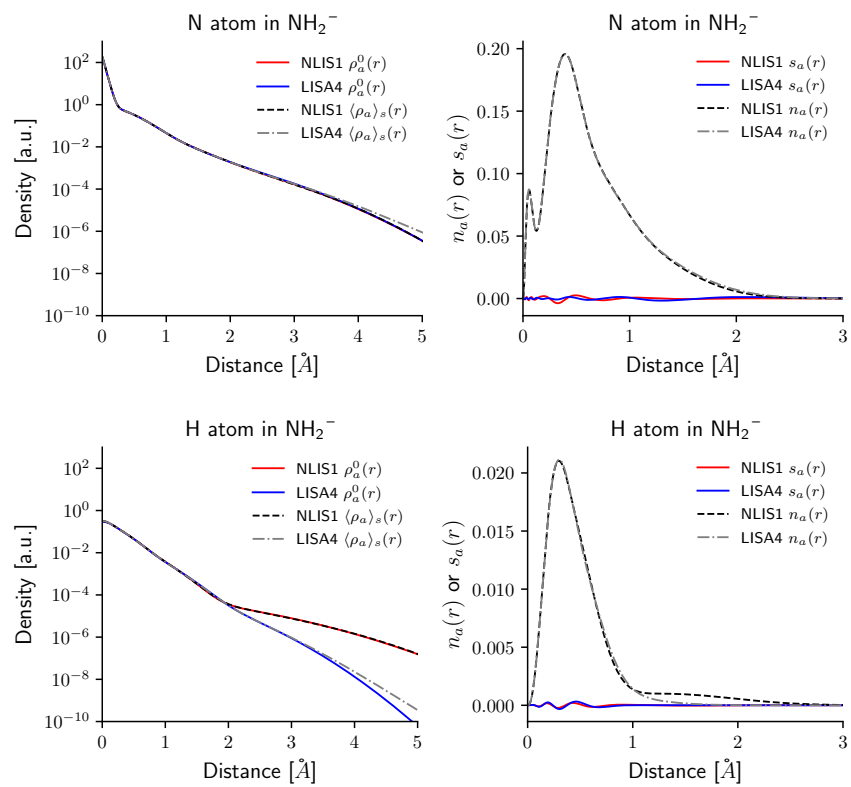

Figure S17: Comparison between the NLIS1 and LISA4 methods for  $\text{NH}_2^-$ .  $\rho_a^0(r)$  and  $\langle \rho_a \rangle_s(r)$  for different atoms (left), and  $s_a(r)$  and  $n_a(r)$  for different atoms (right).

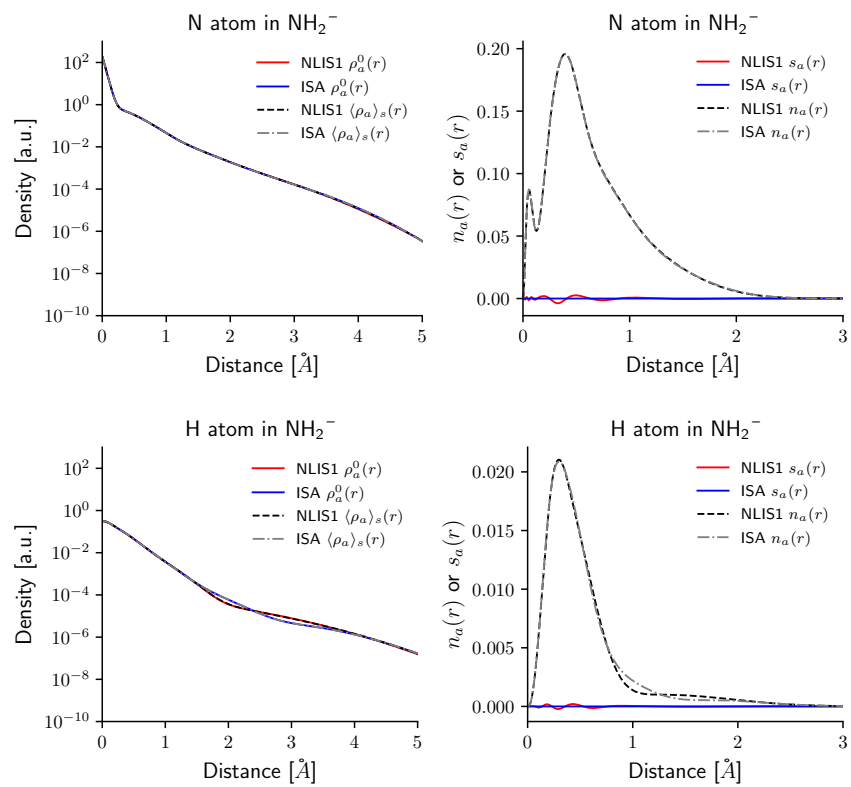

Figure S18: Comparison between the NLIS1 and ISA methods for  $\text{NH}_2^-$ .  $\rho_a^0(r)$  and  $\langle \rho_a \rangle_s(r)$  for different atoms (left), and  $s_a(r)$  and  $n_a(r)$  for different atoms (right).

## S4.7 $\text{H}_3\text{O}^+$

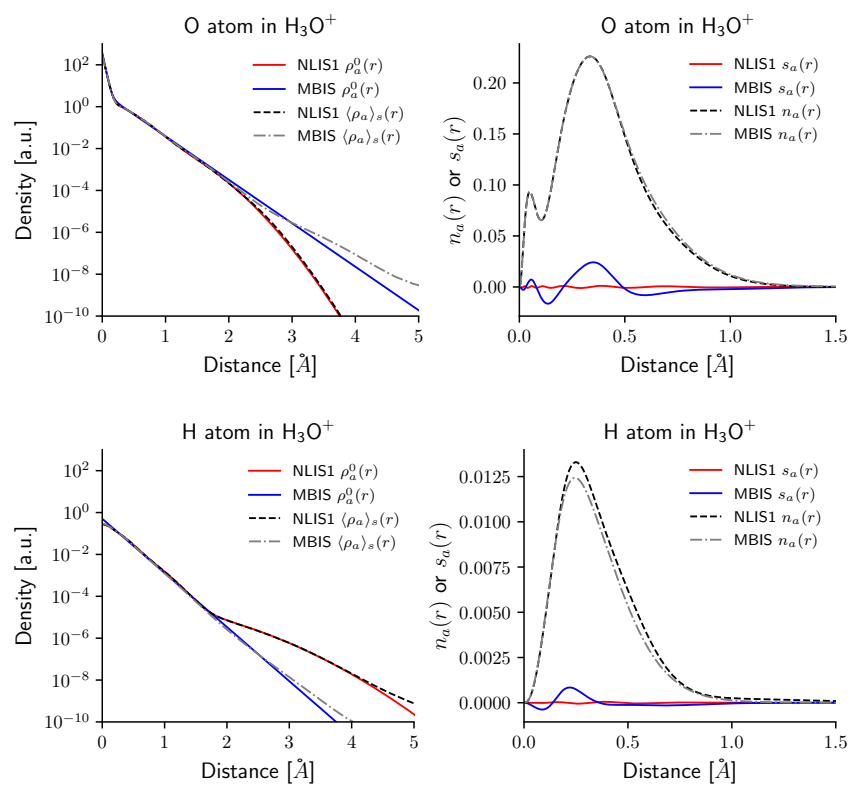

Figure S19: Comparison between the NLIS1 and MBIS methods for  $\text{H}_3\text{O}^+$ .  $\rho_a^0(r)$  and  $\langle \rho_a \rangle_s(r)$  for different atoms (left), and  $s_a(r)$  and  $n_a(r)$  for different atoms (right).

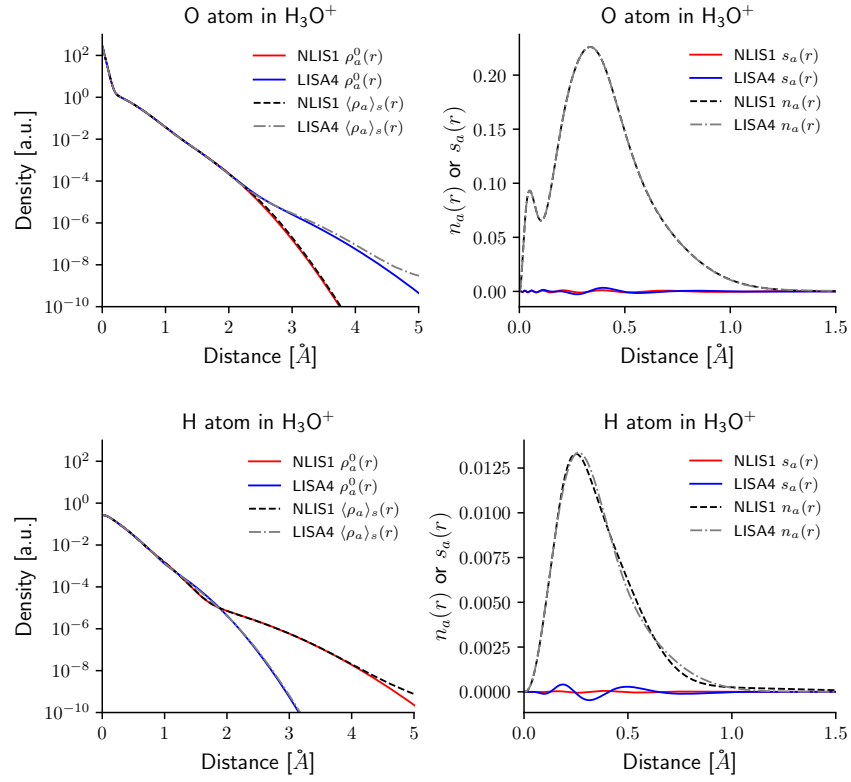

Figure S20: Comparison between the NLIS1 and LISA4 methods for  $\text{H}_3\text{O}^+$ .  $\rho_a^0(r)$  and  $\langle\rho_a\rangle_s(r)$  for different atoms (left), and  $s_a(r)$  and  $n_a(r)$  for different atoms (right).

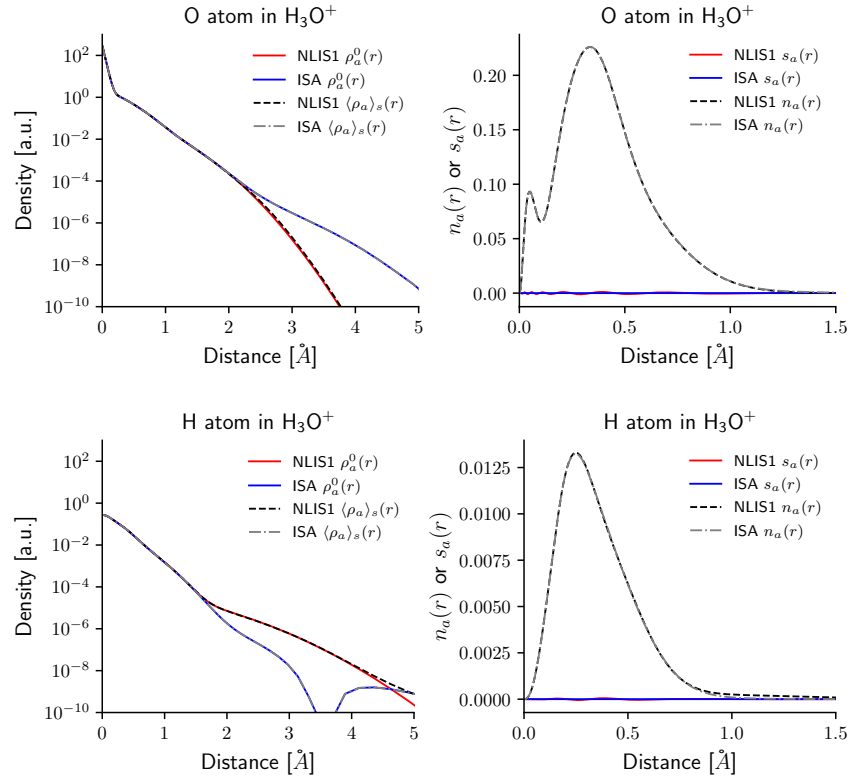

Figure S21: Comparison between the NLIS1 and ISA methods for  $\text{H}_3\text{O}^+$ .  $\rho_a^0(r)$  and  $\langle\rho_a\rangle_s(r)$  for different atoms (left), and  $s_a(r)$  and  $n_a(r)$  for different atoms (right).



## S4.8 H<sub>2</sub>O

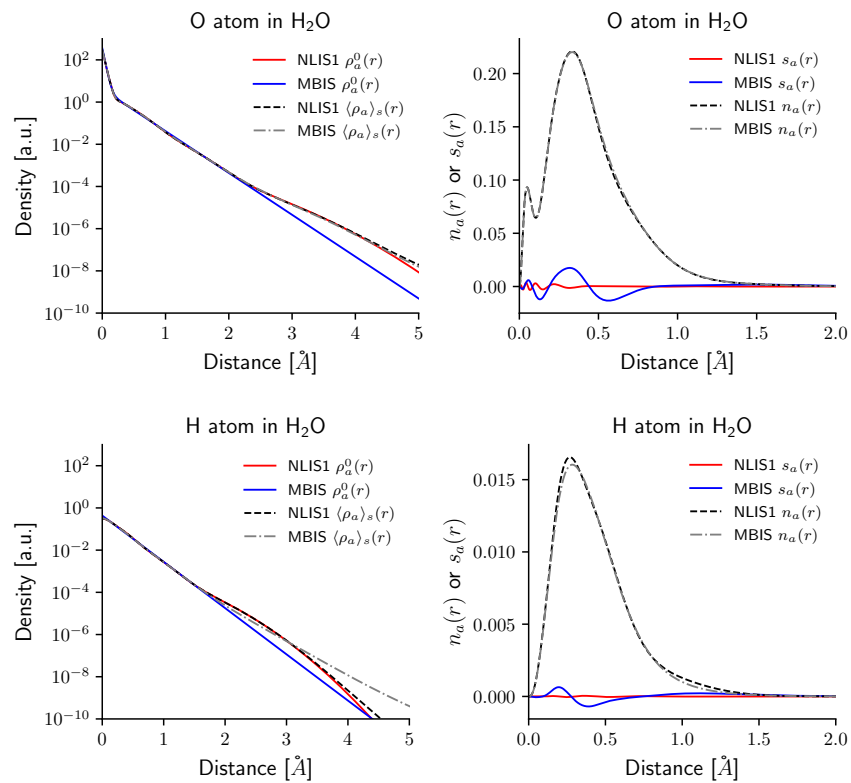

Figure S22: Comparison between the NLIS1 and MBIS methods for H<sub>2</sub>O.  $\rho_a^0(r)$  and  $\langle \rho_a \rangle_s(r)$  for different atoms (left), and  $s_a(r)$  and  $n_a(r)$  for different atoms (right).

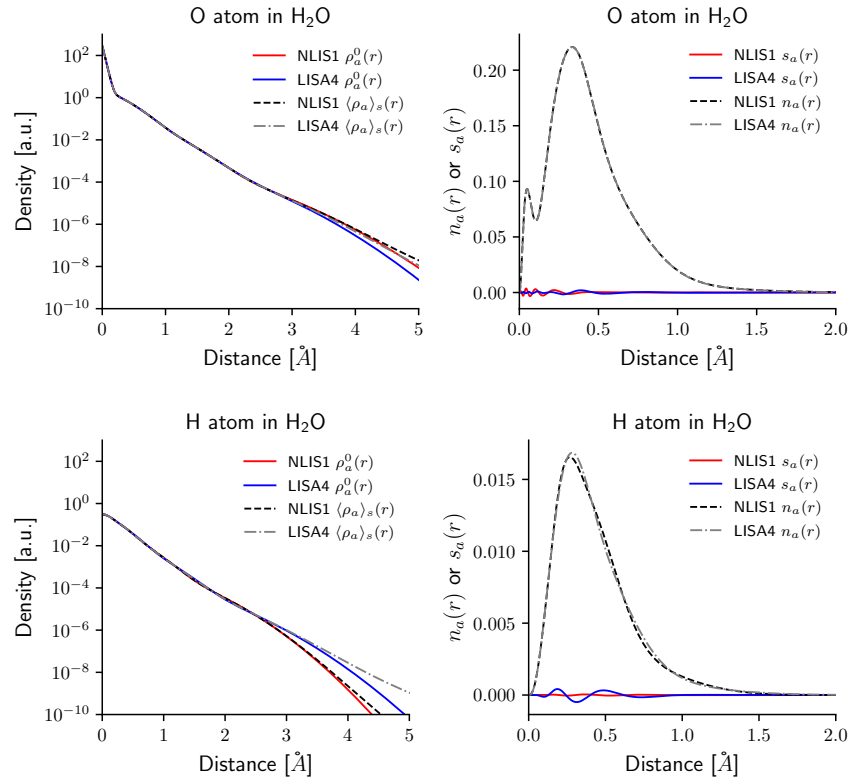

Figure S23: Comparison between the NLIS1 and LISA4 methods for H<sub>2</sub>O.  $\rho_a^0(r)$  and  $\langle \rho_a \rangle_s(r)$  for different atoms (left), and  $s_a(r)$  and  $n_a(r)$  for different atoms (right).

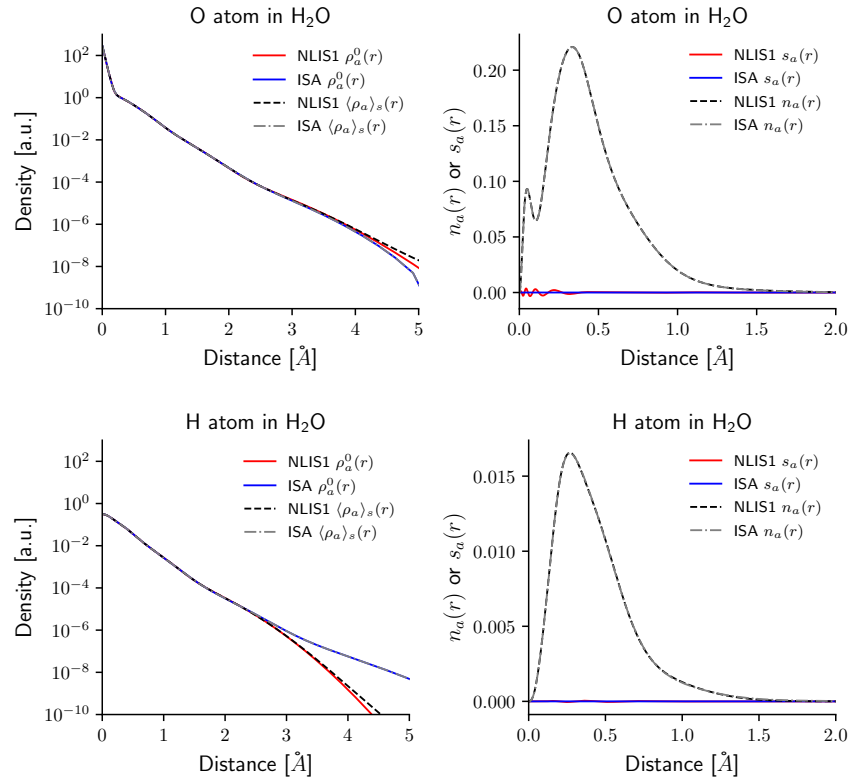

Figure S24: Comparison between the NLIS1 and ISA methods for H<sub>2</sub>O.  $\rho_a^0(r)$  and  $\langle \rho_a \rangle_s(r)$  for different atoms (left), and  $s_a(r)$  and  $n_a(r)$  for different atoms (right).

## S4.9 OH<sup>-</sup>

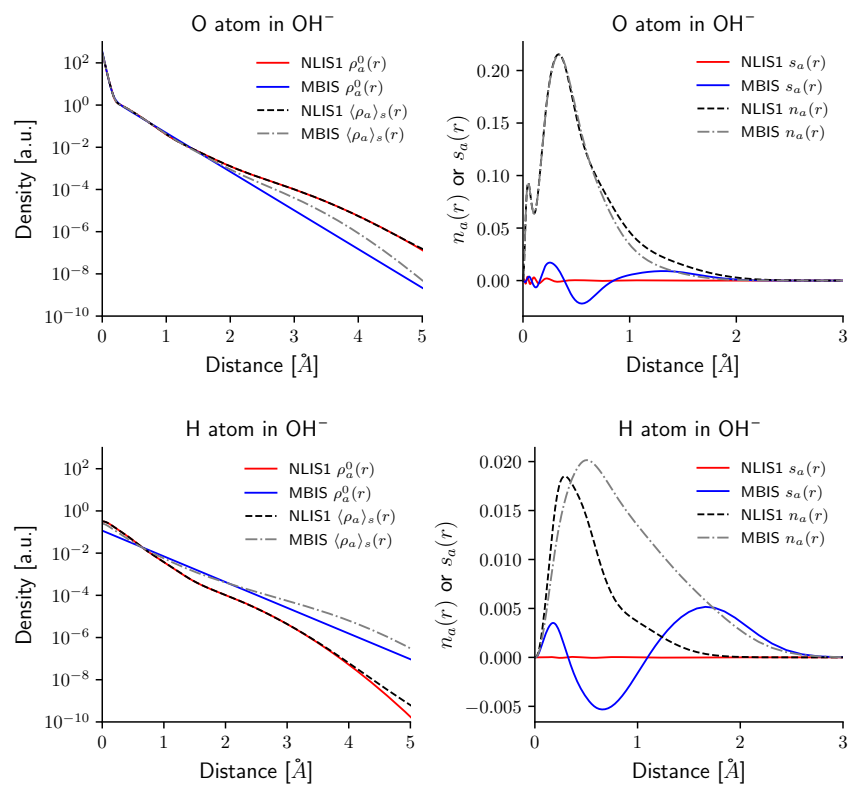

Figure S25: Comparison between the NLIS1 and MBIS methods for OH<sup>-</sup>.  $\rho_a^0(r)$  and  $\langle \rho_a \rangle_s(r)$  for different atoms (left), and  $s_a(r)$  and  $n_a(r)$  for different atoms (right).

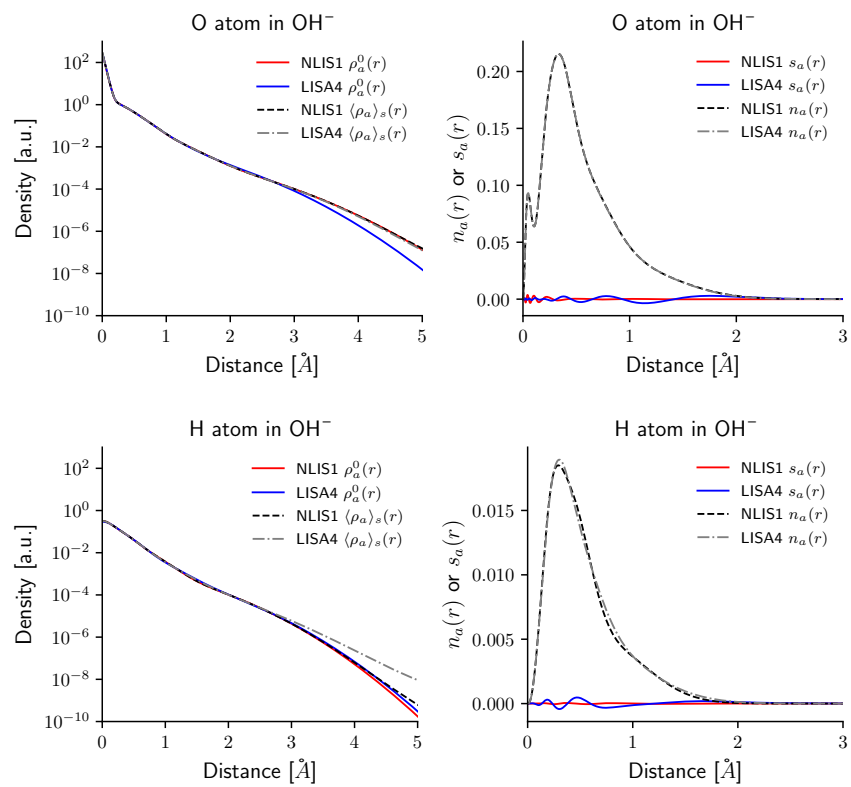

Figure S26: Comparison between the NLIS1 and LISA4 methods for  $\text{OH}^-$ .  $\rho_a^0(r)$  and  $\langle \rho_a \rangle_s(r)$  for different atoms (left), and  $s_a(r)$  and  $n_a(r)$  for different atoms (right).

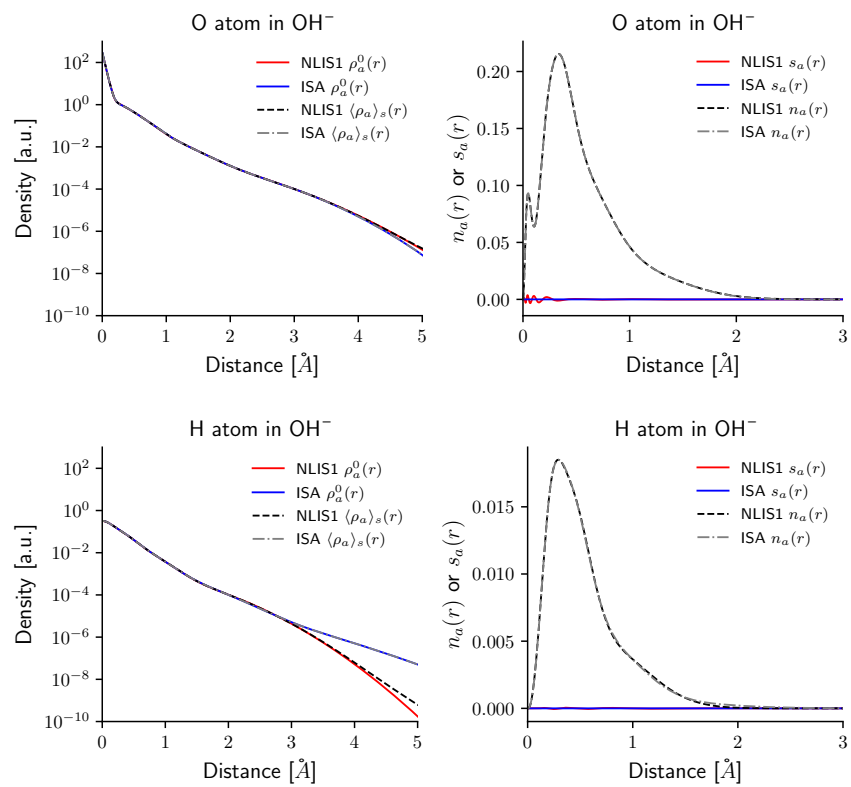

Figure S27: Comparison between the NLIS1 and ISA methods for  $\text{OH}^-$ .  $\rho_a^0(r)$  and  $\langle \rho_a \rangle_s(r)$  for different atoms (left), and  $s_a(r)$  and  $n_a(r)$  for different atoms (right).

## S4.10 CS<sub>2</sub>

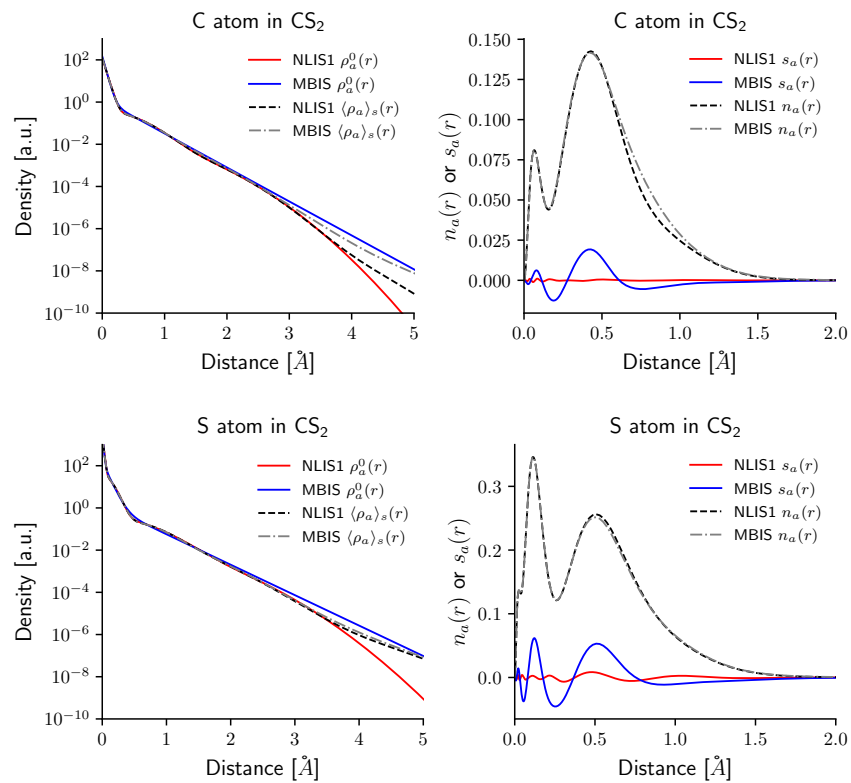

Figure S28: Comparison between the NLIS1 and MBIS methods for CS<sub>2</sub>.  $\rho_a^0(r)$  and  $\langle \rho_a \rangle_s(r)$  for different atoms (left), and  $s_a(r)$  and  $n_a(r)$  for different atoms (right).

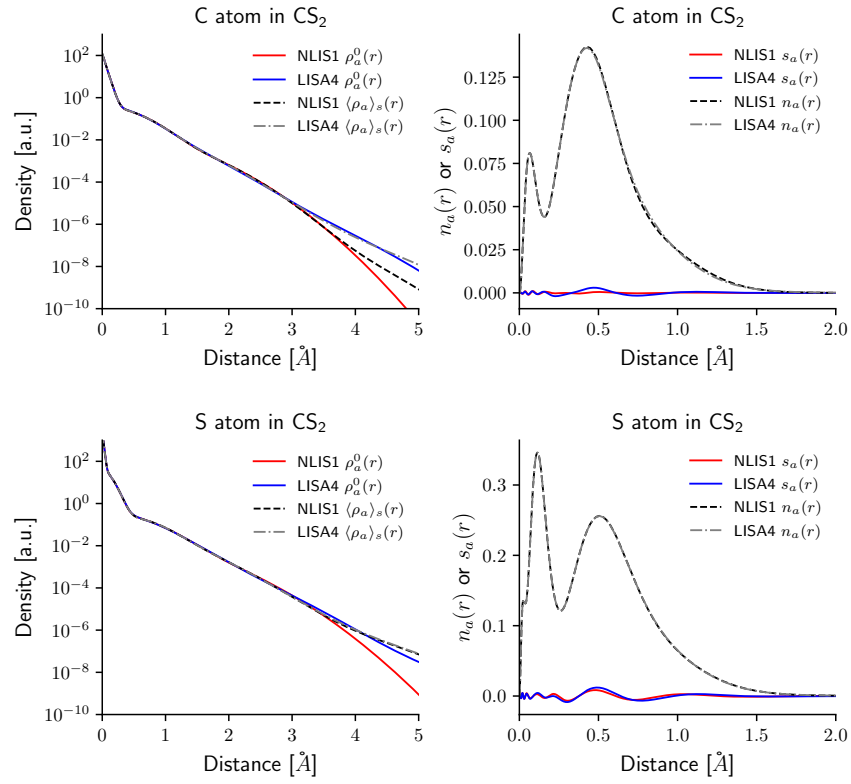

Figure S29: Comparison between the NLIS1 and LISA4 methods for  $\text{CS}_2$ .  $\rho_a^0(r)$  and  $\langle \rho_a \rangle_s(r)$  for different atoms (left), and  $s_a(r)$  and  $n_a(r)$  for different atoms (right).



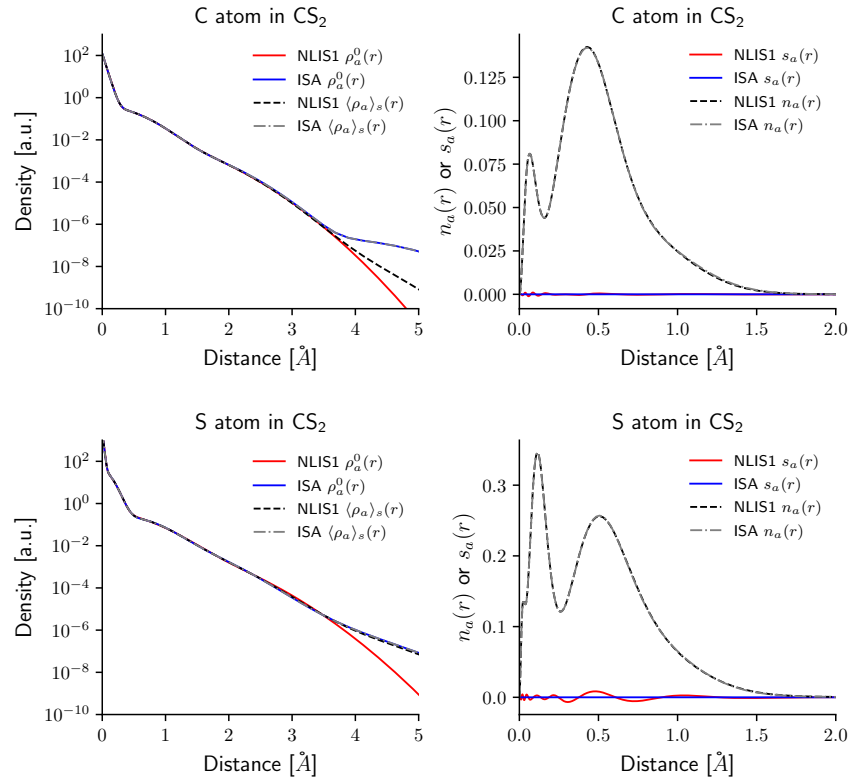

Figure S30: Comparison between the NLIS1 and ISA methods for CS<sub>2</sub>.  $\rho_a^0(r)$  and  $\langle \rho_a \rangle_s(r)$  for different atoms (left), and  $s_a(r)$  and  $n_a(r)$  for different atoms (right).

## S4.11 CCl<sub>4</sub>

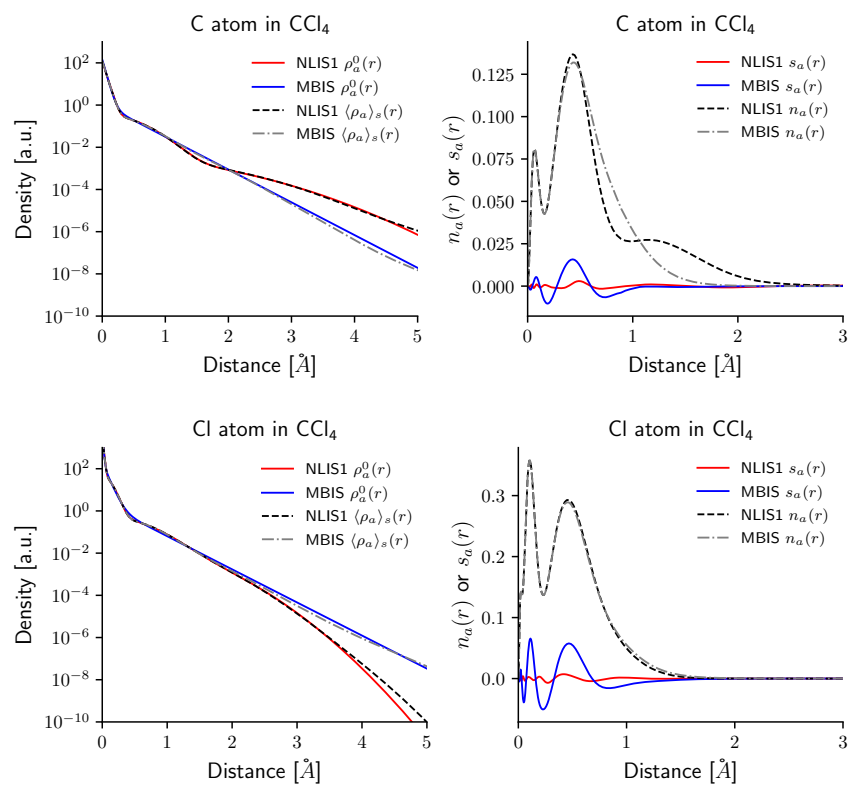

Figure S31: Comparison between the NLIS1 and MBIS methods for CCl<sub>4</sub>.  $\rho_a^0(r)$  and  $\langle \rho_a \rangle_s(r)$  for different atoms (left), and  $s_a(r)$  and  $n_a(r)$  for different atoms (right).

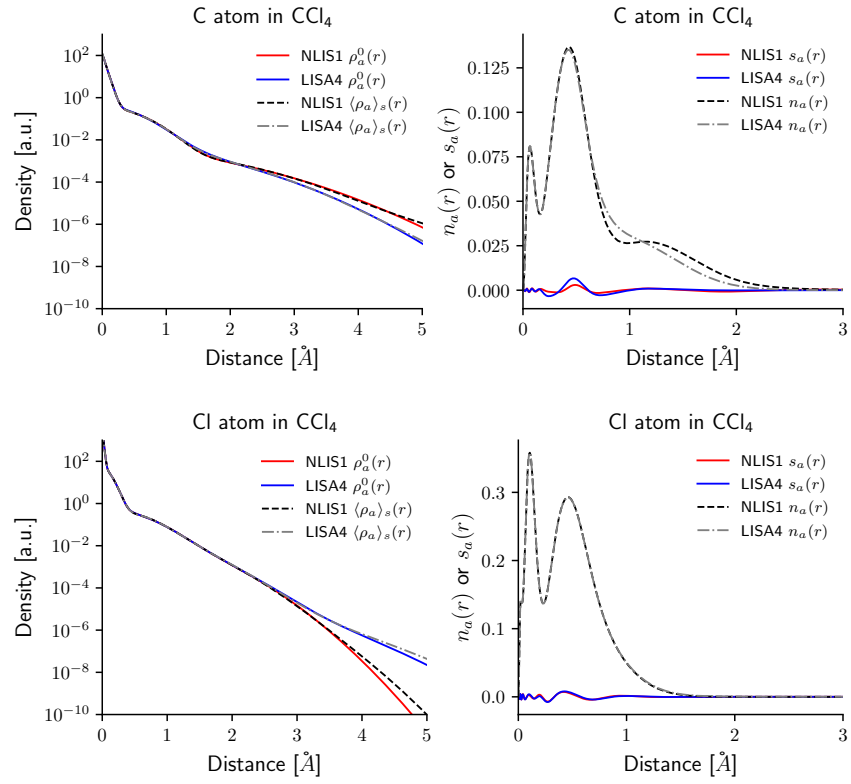

Figure S32: Comparison between the NLIS1 and LISA4 methods for CCl<sub>4</sub>.  $\rho_a^0(r)$  and  $\langle \rho_a \rangle_s(r)$  for different atoms (left), and  $s_a(r)$  and  $n_a(r)$  for different atoms (right).

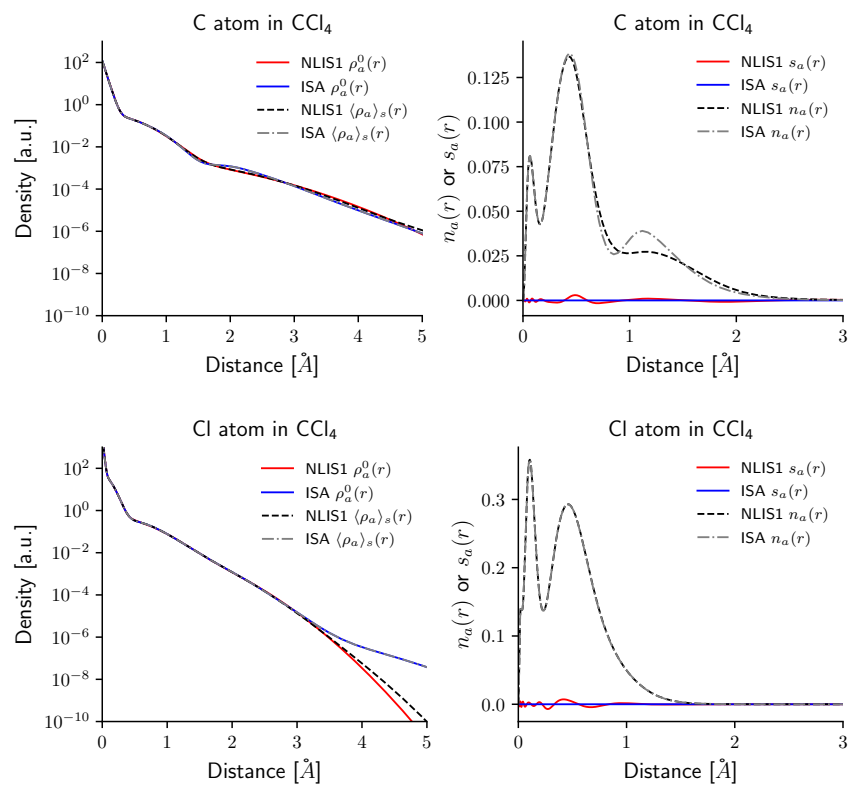

Figure S33: Comparison between the NLIS1 and ISA methods for  $\text{CCl}_4$ .  $\rho_a^0(r)$  and  $\langle \rho_a \rangle_s(r)$  for different atoms (left), and  $s_a(r)$  and  $n_a(r)$  for different atoms (right).

## S4.12 B<sub>8</sub>

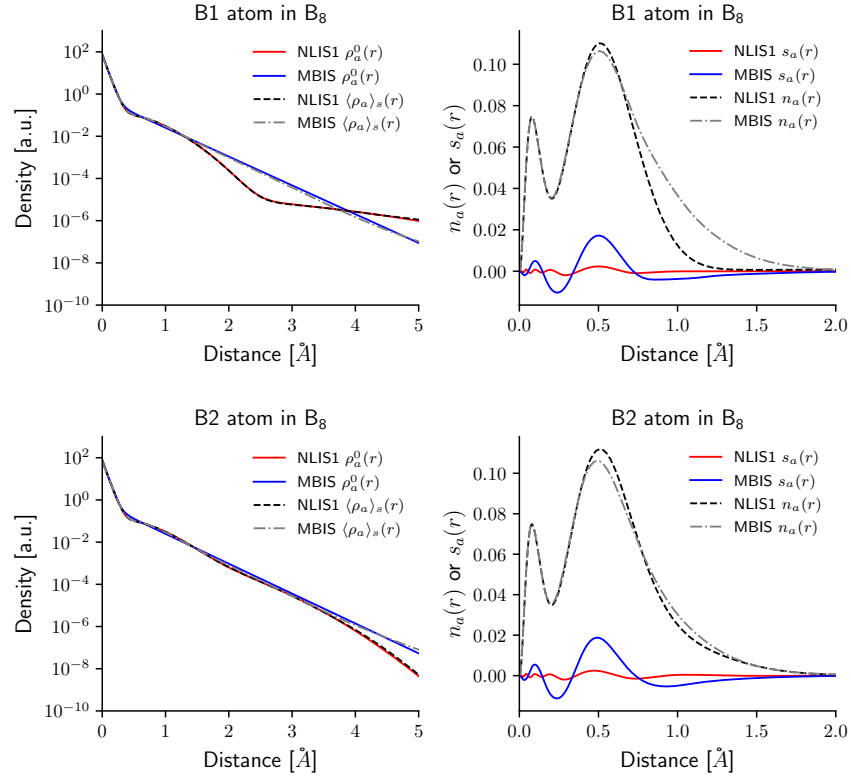

Figure S34: Comparison between the NLIS1 and MBIS methods for B<sub>8</sub>.  $\rho_a^0(r)$  and  $\langle \rho_a \rangle_s(r)$  for different atoms (left), and  $s_a(r)$  and  $n_a(r)$  for different atoms (right).

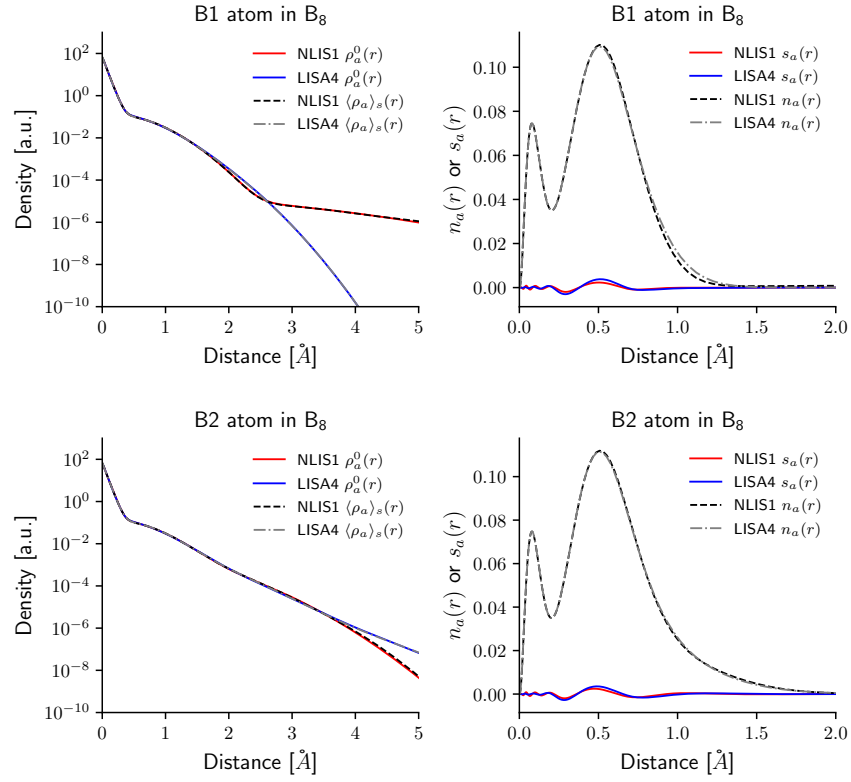

Figure S35: Comparison between the NLIS1 and LISA4 methods for B<sub>8</sub>.  $\rho_a^0(r)$  and  $\langle \rho_a \rangle_s(r)$  for different atoms (left), and  $s_a(r)$  and  $n_a(r)$  for different atoms (right).

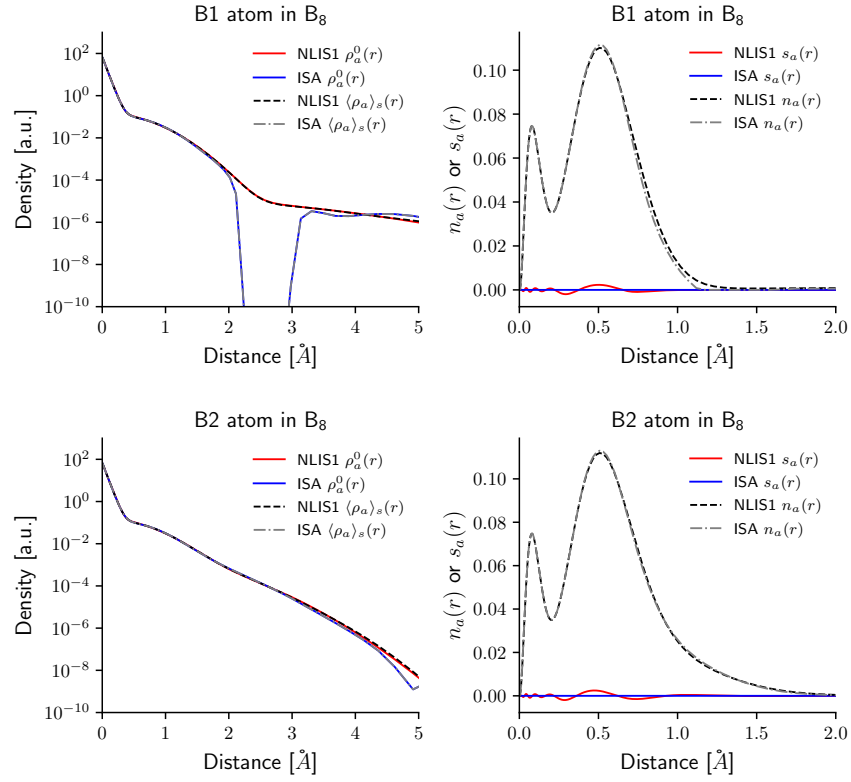

Figure S36: Comparison between the NLIS1 and ISA methods for B<sub>8</sub>.  $\rho_a^0(r)$  and  $\langle \rho_a \rangle_s(r)$  for different atoms (left), and  $s_a(r)$  and  $n_a(r)$  for different atoms (right).

### S4.13 B<sub>8</sub> triplet

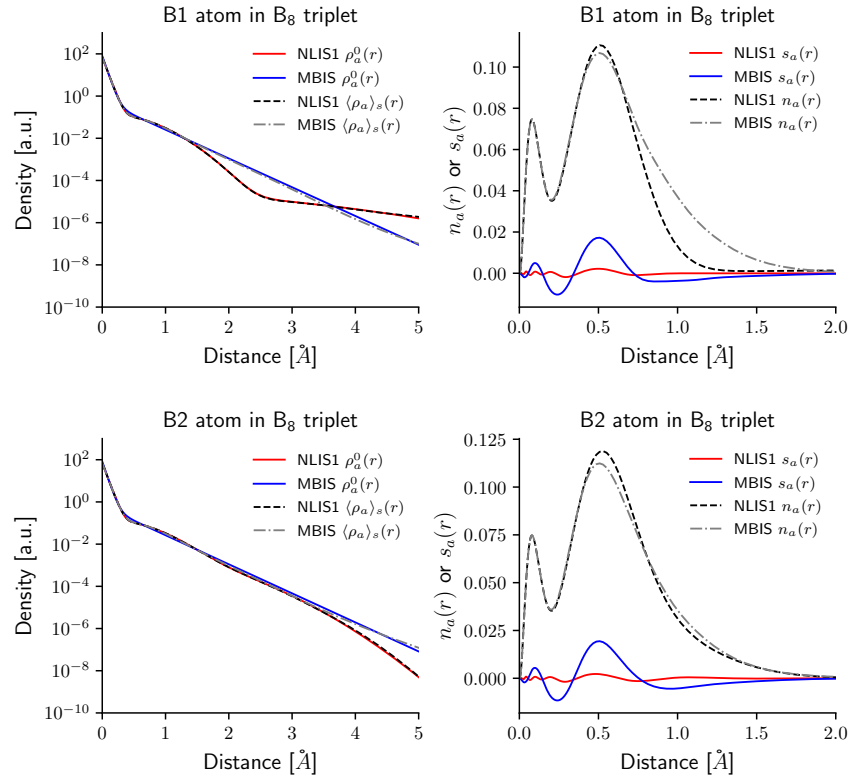

Figure S37: Comparison between the NLIS1 and MBIS methods for B<sub>8</sub> triplet.  $\rho_a^0(r)$  and  $\langle \rho_a \rangle_s(r)$  for different atoms (left), and  $s_a(r)$  and  $n_a(r)$  for different atoms (right).



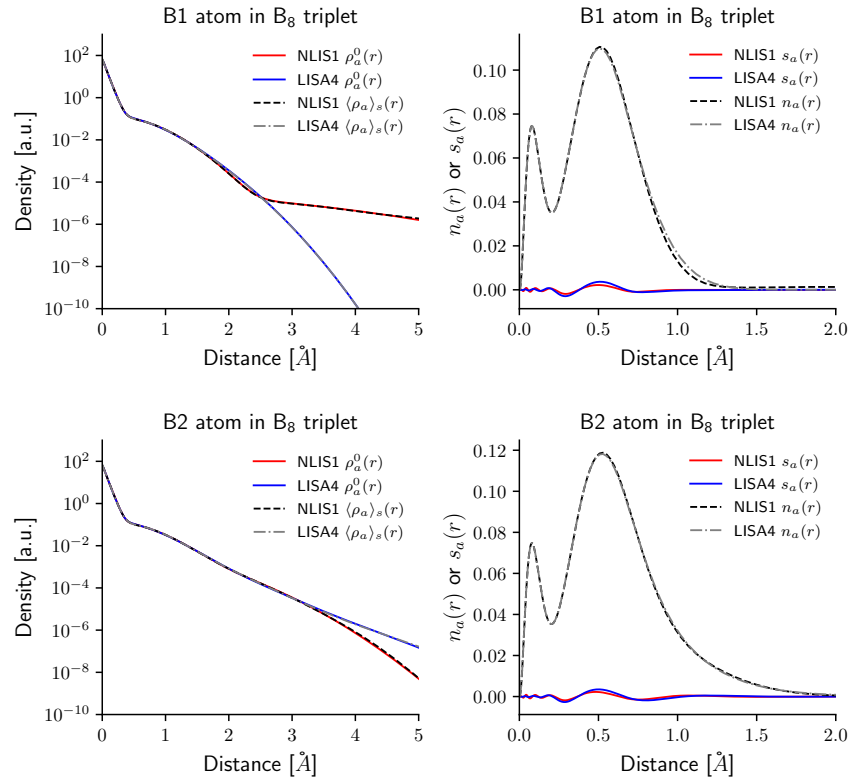

Figure S38: Comparison between the NLIS1 and LISA4 methods for B<sub>8</sub> triplet.  $\rho_a^0(r)$  and  $\langle \rho_a \rangle_s(r)$  for different atoms (left), and  $s_a(r)$  and  $n_a(r)$  for different atoms (right).

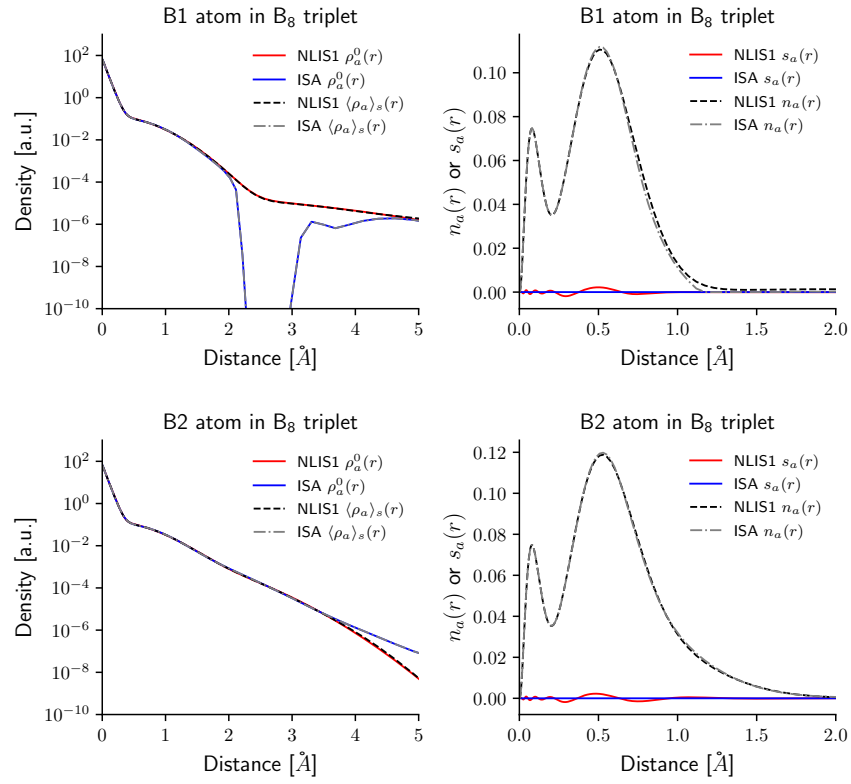

Figure S39: Comparison between the NLIS1 and ISA methods for B<sub>8</sub> triplet.  $\rho_a^0(r)$  and  $\langle \rho_a \rangle_s(r)$  for different atoms (left), and  $s_a(r)$  and  $n_a(r)$  for different atoms (right).

## S4.14 $B_8^{2-}$

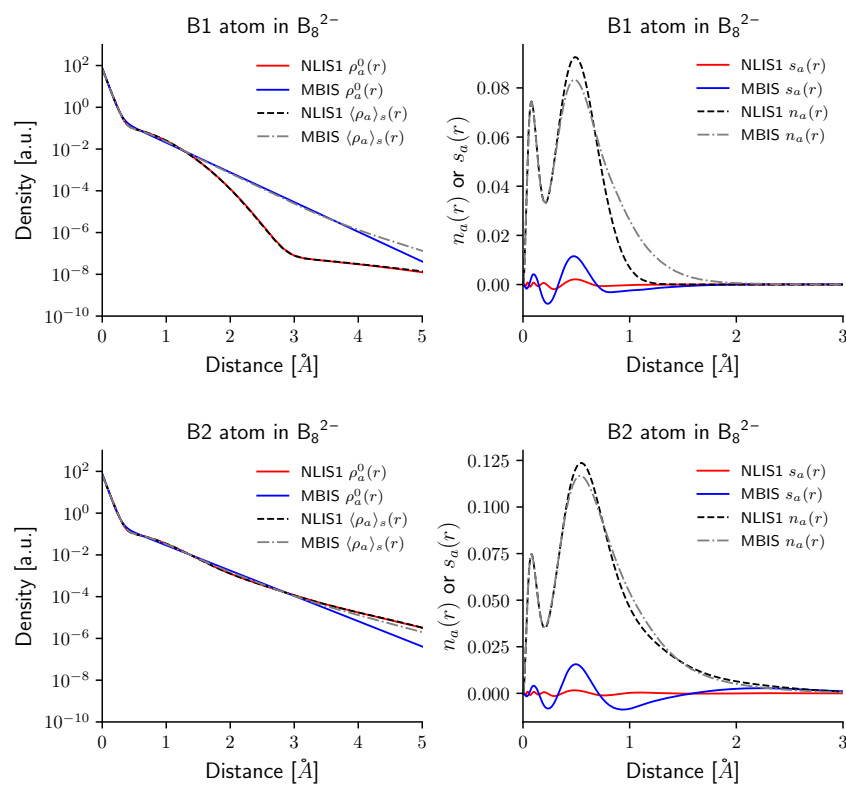

Figure S40: Comparison between the NLIS1 and MBIS methods for  $B_8^{2-}$ .  $\rho_a^0(r)$  and  $\langle \rho_a \rangle_s(r)$  for different atoms (left), and  $s_a(r)$  and  $n_a(r)$  for different atoms (right).

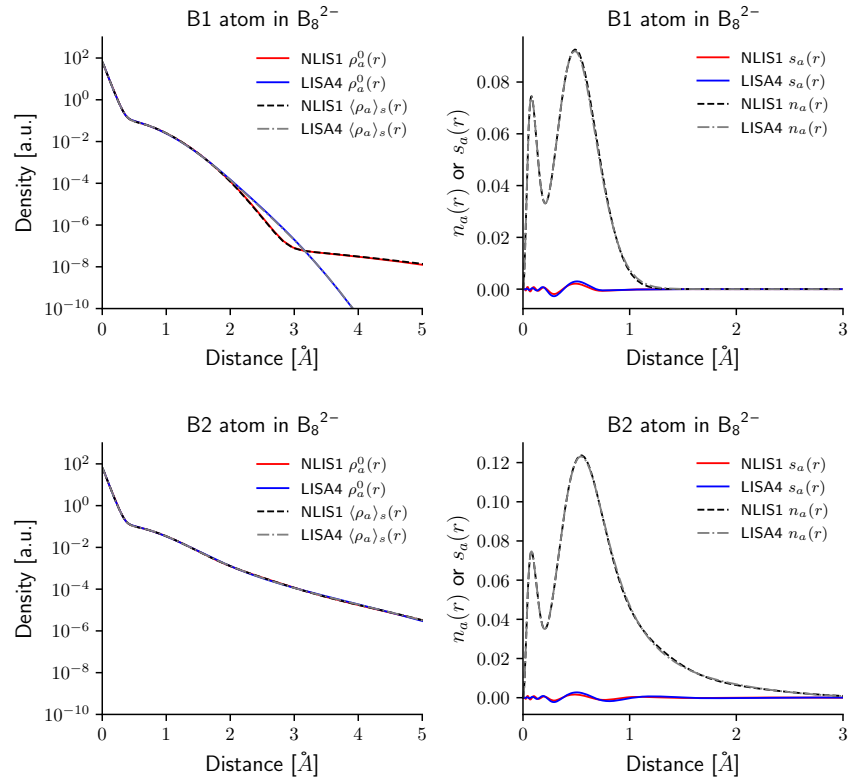

Figure S41: Comparison between the NLIS1 and LISA4 methods for  $B_8^{2-}$ .  $\rho_a^0(r)$  and  $\langle \rho_a \rangle_s(r)$  for different atoms (left), and  $s_a(r)$  and  $n_a(r)$  for different atoms (right).

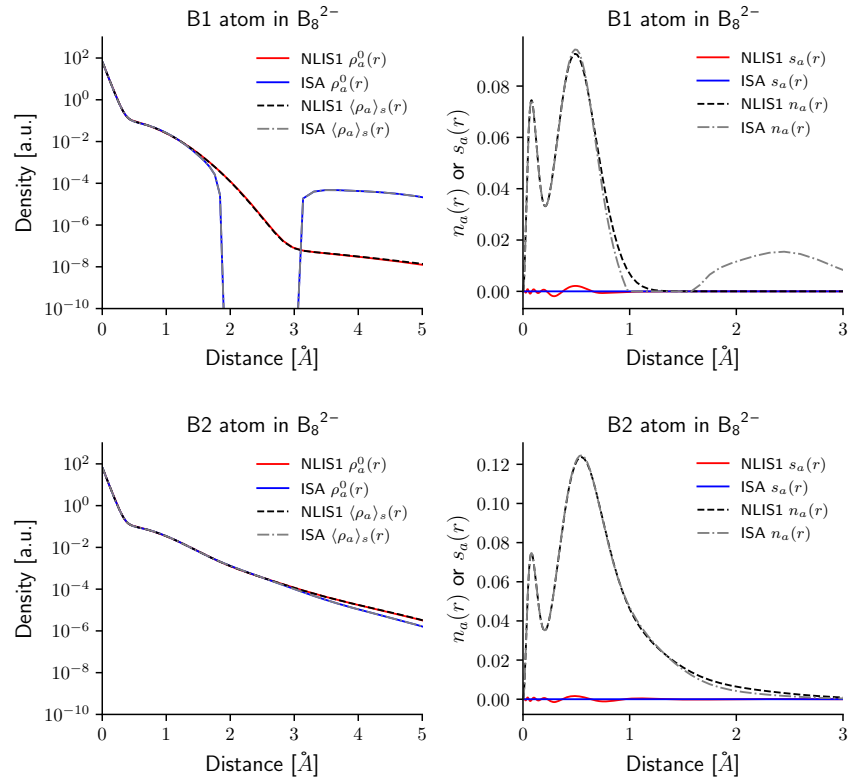

Figure S42: Comparison between the NLIS1 and ISA methods for  $B_8^{2-}$ .  $\rho_a^0(r)$  and  $\langle \rho_a \rangle_s(r)$  for different atoms (left), and  $s_a(r)$  and  $n_a(r)$  for different atoms (right).

## S4.15 $B_9^-$

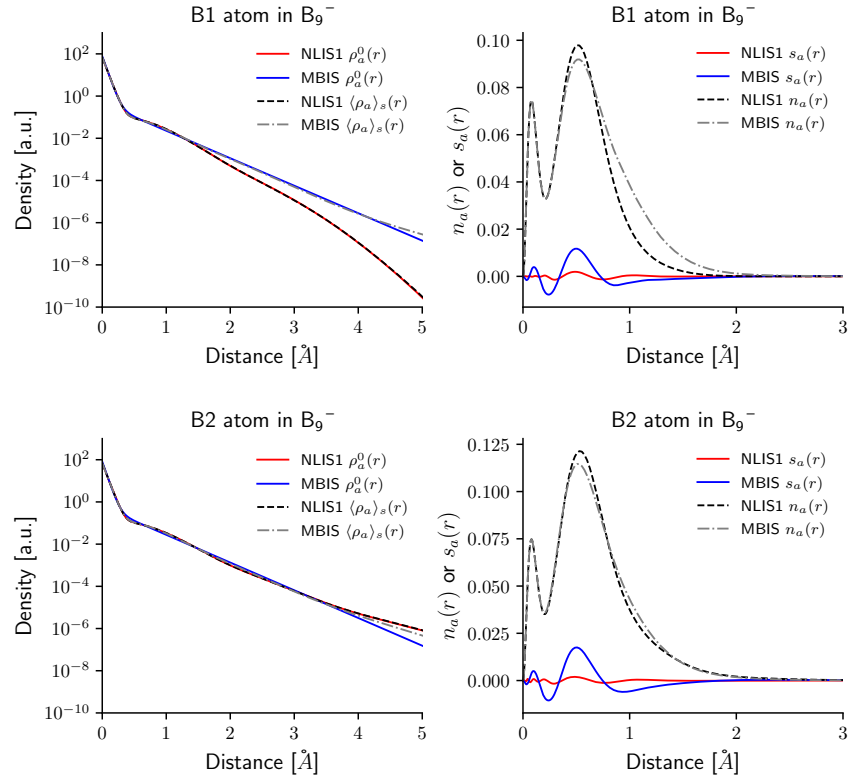

Figure S43: Comparison between the NLIS1 and MBIS methods for  $B_9^-$ .  $\rho_a^0(r)$  and  $\langle \rho_a \rangle_s(r)$  for different atoms (left), and  $s_a(r)$  and  $n_a(r)$  for different atoms (right).

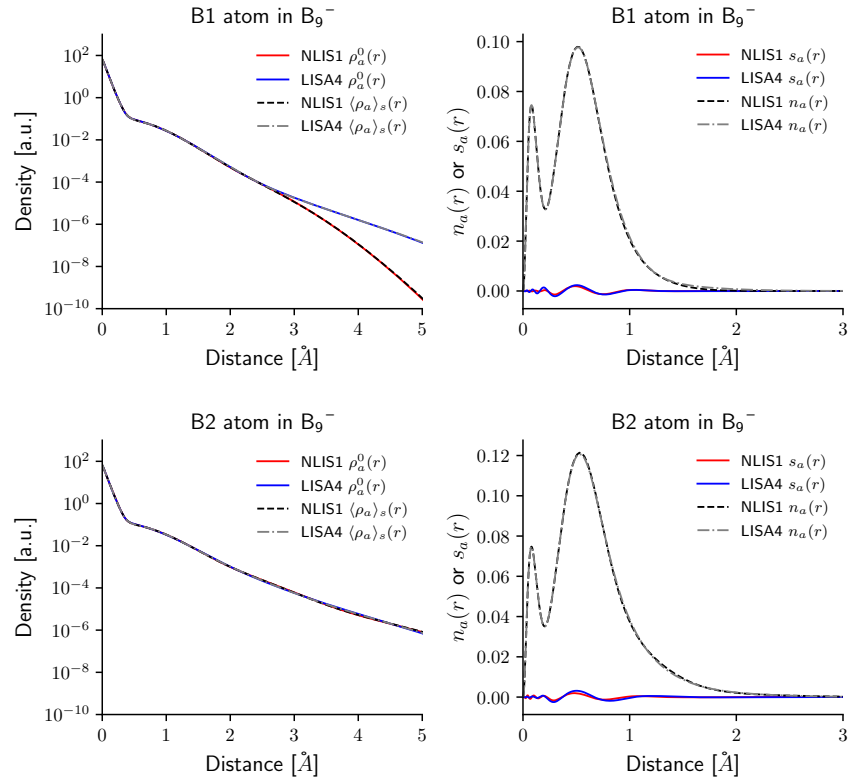

Figure S44: Comparison between the NLIS1 and LISA4 methods for  $B_9^-$ .  $\rho_a^0(r)$  and  $\langle \rho_a \rangle_s(r)$  for different atoms (left), and  $s_a(r)$  and  $n_a(r)$  for different atoms (right).

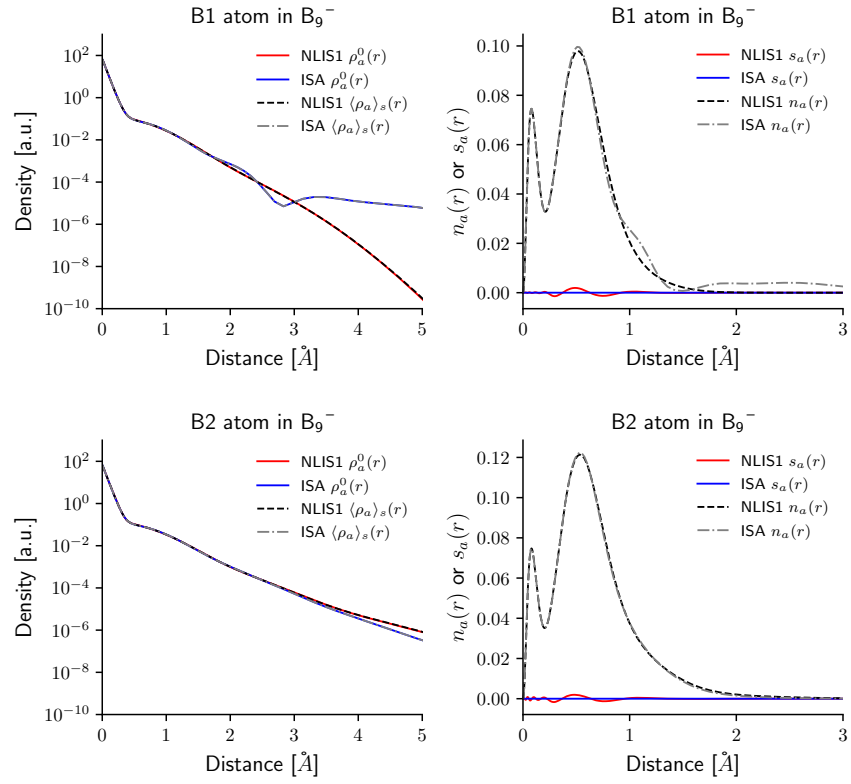

Figure S45: Comparison between the NLIS1 and ISA methods for  $B_9^-$ .  $\rho_a^0(r)$  and  $\langle \rho_a \rangle_s(r)$  for different atoms (left), and  $s_a(r)$  and  $n_a(r)$  for different atoms (right).



Table S46 lists all exceptions for  $T$  observed in this work. In these tables, each row is indexed as “X vs. Y”, where “X” represents method X and “Y” represents method Y being compared. The symbol  $>$  indicates that method “X” has a smaller  $S$  value but a larger  $T$  value than method “Y”. Conversely, the symbol  $<$  indicates that method “X” has a larger  $S$  value but a smaller  $T$  value than method “Y”.

Table S46: Inconsistent cases of  $S$  and  $T$  values. Each row is indexed as “X vs. Y”, representing the comparison between methods “X” and “Y”. The symbol  $>$  indicates that method “X” has a smaller  $S$  value but a larger  $T$  value than method “Y”. Conversely, the symbol  $<$  indicates that method “X” has a larger  $S$  value but a smaller  $T$  value than method “Y”.

|                 | $\text{CH}_3^+$ | $\text{CH}_4$ | $\text{CH}_3^-$ | $\text{NH}_4^+$ | $\text{NH}_3$ | $\text{NH}_2^-$ | $\text{H}_3\text{O}^+$ | $\text{H}_2\text{O}$ | $\text{OH}^-$ | $\text{CS}_2$ | $\text{CCl}_4$ | $\text{B}_8$ | $\text{B}_8$ triplet | $\text{B}_8^{2-}$ | $\text{B}_9^-$ |
|-----------------|-----------------|---------------|-----------------|-----------------|---------------|-----------------|------------------------|----------------------|---------------|---------------|----------------|--------------|----------------------|-------------------|----------------|
| LISA1 vs. LISA2 |                 |               |                 |                 |               |                 |                        | $<$                  |               |               |                |              |                      |                   |                |
| LISA1 vs. LISA4 |                 |               |                 |                 |               |                 |                        |                      |               | $<$           | $<$            |              |                      |                   |                |
| LISA1 vs. LISA5 |                 |               |                 |                 |               |                 |                        |                      | $<$           |               |                |              |                      |                   |                |
| LISA1 vs. LISA6 |                 |               |                 |                 |               | $<$             |                        |                      | $<$           |               |                |              |                      |                   |                |
| LISA1 vs. NLIS1 |                 |               |                 |                 |               |                 |                        | $<$                  |               |               |                |              |                      |                   |                |
| LISA1 vs. NLIS2 |                 |               |                 | $<$             | $<$           |                 | $<$                    |                      |               |               |                |              |                      | $<$               |                |
| LISA1 vs. NLIS3 |                 |               |                 |                 | $<$           |                 |                        | $<$                  |               |               | $>$            |              |                      | $<$               |                |
| LISA1 vs. NLIS4 |                 |               |                 |                 |               |                 |                        |                      | $<$           |               |                |              |                      |                   |                |
| LISA1 vs. MBIS  |                 |               |                 |                 |               | $<$             |                        |                      |               |               |                |              |                      |                   |                |
| LISA1 vs. GMBIS |                 |               |                 |                 |               | $<$             |                        |                      |               |               |                |              |                      |                   |                |
| LISA2 vs. LISA4 |                 |               |                 |                 |               |                 |                        |                      |               | $<$           | $<$            |              |                      |                   |                |
| LISA2 vs. LISA6 |                 |               | $<$             |                 |               | $<$             |                        |                      |               |               |                |              |                      |                   |                |
| LISA2 vs. NLIS1 |                 |               |                 |                 |               |                 |                        | $<$                  |               |               |                |              |                      |                   |                |
| LISA2 vs. NLIS2 |                 |               |                 | $<$             | $<$           |                 | $<$                    |                      |               |               |                |              |                      | $<$               |                |
| LISA2 vs. NLIS3 |                 |               |                 |                 | $<$           |                 |                        | $<$                  |               |               | $>$            |              |                      | $<$               |                |
| LISA2 vs. NLIS4 |                 |               | $<$             |                 |               | $<$             |                        |                      |               |               |                |              |                      |                   |                |
| LISA3 vs. NLIS1 |                 |               | $>$             |                 |               | $<$             |                        |                      | $<$           |               |                |              |                      |                   |                |
| LISA3 vs. NLIS2 |                 |               | $>$             |                 |               | $<$             |                        |                      | $<$           |               |                |              |                      |                   |                |
| LISA3 vs. NLIS3 |                 |               | $>$             |                 |               |                 |                        |                      | $<$           |               |                |              |                      |                   |                |
| LISA3 vs. ISA   |                 |               | $>$             |                 |               |                 |                        |                      |               |               |                |              |                      |                   |                |
| LISA4 vs. NLIS1 |                 |               |                 |                 | $<$           | $<$             | $<$                    |                      | $<$           |               |                | $<$          | $<$                  | $<$               | $<$            |
| LISA4 vs. NLIS2 |                 |               |                 |                 |               | $<$             |                        |                      | $<$           |               |                |              |                      | $<$               |                |
| LISA4 vs. NLIS3 |                 |               |                 |                 |               |                 | $<$                    |                      | $<$           |               | $>$            |              |                      | $<$               |                |
| LISA6 vs. MBIS  |                 |               | $>$             |                 |               |                 |                        |                      |               |               |                |              |                      | $>$               |                |

Continued on next page

Table S46: Inconsistent cases of  $S$  and  $T$  values. Each row is indexed as “X vs. Y”, representing the comparison between methods “X” and “Y”. The symbol  $>$  indicates that method “X” has a smaller  $S$  value but a larger  $T$  value than method “Y”. Conversely, the symbol  $<$  indicates that method “X” has a larger  $S$  value but a smaller  $T$  value than method “Y”.

|                 | $\text{CH}_3^+$ | $\text{CH}_4$ | $\text{CH}_3^-$ | $\text{NH}_4^+$ | $\text{NH}_3$ | $\text{NH}_2^-$ | $\text{H}_3\text{O}^+$ | $\text{H}_2\text{O}$ | $\text{OH}^-$ | $\text{CS}_2$ | $\text{CCl}_4$ | $\text{B}_8$ | $\text{B}_8$ triplet | $\text{B}_8^{2-}$ | $\text{B}_9^-$ |
|-----------------|-----------------|---------------|-----------------|-----------------|---------------|-----------------|------------------------|----------------------|---------------|---------------|----------------|--------------|----------------------|-------------------|----------------|
| LISA6 vs. GMBIS |                 |               | $>$             |                 |               |                 |                        |                      |               |               |                |              |                      | $>$               |                |
| NLIS1 vs. NLIS2 |                 |               | $>$             |                 |               |                 |                        |                      |               |               |                |              |                      |                   |                |
| NLIS1 vs. NLIS3 |                 |               | $>$             |                 |               |                 |                        |                      |               |               | $>$            |              |                      |                   |                |
| NLIS4 vs. MBIS  |                 | $>$           |                 |                 |               |                 |                        |                      |               |               |                | $>$          |                      |                   |                |
| NLIS4 vs. GMBIS |                 |               |                 |                 |               |                 |                        | $>$                  |               |               |                |              |                      | $>$               |                |
| MBIS vs. GMBIS  |                 |               |                 |                 |               |                 |                        |                      | $>$           |               |                |              |                      |                   |                |
